# Supplementary material for: The non-linear coupled spin 2 - spin 3 Cotton equation in three dimensions
Source: arXiv:1602.01682 ancillary file (2016-03-18)
Supplement: Supplementary file 1 [file cotton_spin3_frame.pdf]

$$\begin{aligned}
& \frac{1}{9}D_{[\mu D \nu] D} (a D | c D c e d | b) d + \frac{1}{18}D_{[\mu D \nu] D} (a D | c | D b) e^d c d - \frac{1}{9}D_{[\mu D \nu] D} (a D | c D d | e c b) d \\
& - \frac{1}{18}D_{[\mu D \nu] D} (a D | c D d | e b) c d - \frac{1}{6}D_{[\mu D \nu] D} c D (a D c e | d | b) d + \frac{1}{6}D_{[\mu D \nu] D} c D (a D | d | e c b) d \\
& + \frac{1}{12}D_{[\mu D \nu] D} c D d D c e d a b + \frac{1}{27}\eta^{a b} D_{[\mu D \nu] D} c D d D c e^f d f - \frac{1}{12}D_{[\mu D \nu] D} c D d D d e c a b - \\
& \frac{1}{27}\eta^{a b} D_{[\mu D \nu] D} c D d D d e^f c f - \frac{1}{27}\eta^{a b} D_{[\mu D \nu] D} c D d D f e c d f + \frac{1}{27}\eta^{a b} D_{[\mu D \nu] D} c D d D f e d c f \\
& + \frac{19}{96}D_{[\mu D (a D \nu) D | c D c e d | b) d} - \frac{1}{4}D_{[\mu D (a D \nu) D | c | D b) e^d c d} - \frac{19}{96}D_{[\mu D (a D \nu) D | c D d | e c b) d} \\
& + \frac{1}{4}D_{[\mu D (a D \nu) D | c D d | e b) c d} - \frac{19}{96}D_{[\mu D (a D b) D c D | c | e d \nu] d} + \frac{1}{4}D_{[\mu D (a D b) D c D \nu] e^d c d} + \\
& \frac{19}{96}D_{[\mu D (a D b) D c D d e | c d | \nu] d} - \frac{1}{4}D_{[\mu D (a D b) D c D d e \nu] c d} - \frac{1}{6}D_{[\mu D (a D | c D | c | D \nu] e d | b) d} + \\
& \frac{1}{6}D_{[\mu D (a D | c | D | c | D b) e^d \nu] d} + \frac{1}{6}D_{[\mu D (a D | c D | c | D d | e \nu] b) d} - \frac{1}{6}D_{[\mu D (a D | c D | c D d | e b) d | \nu] d} + \\
& + \frac{1}{6}D_{[\mu D (a D | c | D \nu] D b) e^d c d} - \frac{1}{6}D_{[\mu D (a D | c D \nu] D d | e b) c d} - \frac{1}{6}D_{[\mu D (a D | c | D b) D \nu] e^d c d} + \\
& \frac{1}{6}D_{[\mu D (a D | c | D b) D d e \nu] c d} - \frac{1}{6}D_{[\mu D (a D | c D d | D | d | e \nu] b) c} + \frac{1}{6}D_{[\mu D (a D | c D d | D | d e b) c | \nu] d} + \\
& \frac{1}{6}D_{[\mu D (a D | c D d | D \nu] e d b) c} - \frac{1}{6}D_{[\mu D (a D | c D d | D b) e | d c | \nu] d} - \frac{3}{32}D_{[\mu D c D | c | D \nu] D (a e | d | b) d} + \\
& \frac{3}{32}D_{[\mu D c D | c | D \nu] D d e (a b) d} + \frac{13}{48}D_{[\mu D c D | c | D (a D \nu) e | d | b) d} - \frac{3}{32}D_{[\mu D c D | c | D (a D b) e^d \nu] d} - \\
& \frac{13}{48}D_{[\mu D c D | c | D (a D | d | e \nu] b) d} + \frac{3}{32}D_{[\mu D c D | c D (a D | d | e b) d | \nu] d} + \frac{13}{96}D_{[\mu D c D | c D d D d | e \nu] a b} - \\
& \frac{3}{32}D_{[\mu D c D | c D d D d | e (a b) \nu] d} + \frac{61}{288}\eta^{a b} D_{[\mu D c D | c D d D d | e^f \nu] f} - \frac{13}{96}D_{[\mu D c D | c | D d \nu] e d a b} - \\
& \frac{1}{4}\eta^{a b} D_{[\mu D c D | c | D d \nu] e^f d f} + \frac{3}{32}D_{[\mu D c D | c D d D (a e d | b) \nu] d} - \frac{61}{288}\eta^{a b} D_{[\mu D c D | c D d D f e d f | \nu] d} \\
& + \frac{1}{4}\eta^{a b} D_{[\mu D c D | c | D d f e \nu] d f} + \frac{3}{32}D_{[\mu D c D \nu] D c D (a e | d | b) d} - \frac{3}{32}D_{[\mu D c D \nu] D c D d e (a b) d} \\
& - \frac{5}{48}D_{[\mu D c D \nu] D (a D c e | d | b) d} + \frac{3}{32}D_{[\mu D c D \nu] D (a D b) e^d c d} + \frac{5}{48}D_{[\mu D c D \nu] D (a D | d | e c b) d} \\
& - \frac{3}{32}D_{[\mu D c D \nu] D (a D | d | e b) c d} + \frac{5}{96}D_{[\mu D c D \nu] D d D c e d a b} + \frac{7}{36}\eta^{a b} D_{[\mu D c D \nu] D d D c e^f d f} \\
& - \frac{5}{96}D_{[\mu D c D \nu] D d D d e c a b} + \frac{3}{32}D_{[\mu D c D \nu] D d D d e (a b) c} - \frac{61}{288}\eta^{a b} D_{[\mu D c D \nu] D d D d e^f c f} - \\
& \frac{3}{32}D_{[\mu D c D \nu] D d D (a e d b) c} - \frac{7}{36}\eta^{a b} D_{[\mu D c D \nu] D d D f e c d f} + \frac{61}{288}\eta^{a b} D_{[\mu D c D \nu] D d D f e d c f} - \\
& \frac{3}{32}D_{[\mu D c D (a D | c | D \nu] e | d | b) d} - \frac{1}{12}D_{[\mu D c D (a D | c | D b) e^d \nu] d} + \frac{3}{32}D_{[\mu D c D (a D | c | D | d | e \nu] b) d} \\
& + \frac{1}{12}D_{[\mu D c D (a D | c D | d | e b) d | \nu] d} + \frac{3}{32}D_{[\mu D c D (a D \nu) D c e | d | b) d} - \frac{1}{12}D_{[\mu D c D (a D \nu) D b) e^d c d} \\
& - \frac{3}{32}D_{[\mu D c D (a D \nu) D | d | e c b) d} + \frac{1}{12}D_{[\mu D c D (a D \nu) D | d | e b) c d} + \frac{3}{32}D_{[\mu D c D (a D b) D | c | e d \nu] d} \\
& - \frac{3}{32}D_{[\mu D c D (a D b) D \nu] e^d c d} - \frac{3}{32}D_{[\mu D c D (a D b) D d e | c d | \nu] d} + \frac{3}{32}D_{[\mu D c D (a D b) D d e \nu] c d} - \\
& \frac{3}{32}D_{[\mu D c D (a D | d | D | c e d | b) \nu] d} + \frac{3}{32}D_{[\mu D c D (a D | d | D | d e c | b) \nu] d} - \frac{3}{32}D_{[\mu D c D (a D | d | D | d | e \nu] b) c} - \\
& \frac{1}{12}D_{[\mu D c D (a D | d | D | d e b) c | \nu] d} + \frac{3}{32}D_{[\mu D c D (a D | d | D \nu] e d b) c} + \frac{1}{12}D_{[\mu D c D (a D | d | D b) e | d c | \nu] d} +
\end{aligned}$$

$$\begin{aligned}
& \frac{1}{36} \eta^{a b D} [\mu D^c D^d D^e | c D d | e^f v] f + \frac{1}{8} \eta^{a b D} [\mu D^c D^d D^e | c | D v] e^f d f - \frac{1}{36} \eta^{a b D} [\mu D^c D^d D^e | c D^f e d f | v] \\
& - \frac{1}{8} \eta^{a b D} [\mu D^c D^d D^e | c | D^f e v] d f - \frac{1}{8} \eta^{a b D} [\mu D^c D^d D^e | d D c | e^f v] f + \frac{1}{8} \eta^{a b D} [\mu D^c D^d D^e | d | D v] e^f c f \\
& + \frac{1}{8} \eta^{a b D} [\mu D^c D^d D^e | d D^f e c f | v] - \frac{1}{8} \eta^{a b D} [\mu D^c D^d D^e | d | D^f e v] c f - \frac{1}{8} \eta^{a b D} [\mu D^c D^d D^e v] D c e^f d f \\
& + \frac{1}{36} \eta^{a b D} [\mu D^c D^d D^e v] D d e^f c f + \frac{1}{8} \eta^{a b D} [\mu D^c D^d D^e v] D^f e c d f - \frac{1}{36} \eta^{a b D} [\mu D^c D^d D^e v] D^f e d c f + \\
& \frac{1}{8} \eta^{a b D} [\mu D^c D^d D^f D | c e f d | v] - \frac{1}{36} \eta^{a b D} [\mu D^c D^d D^f D | d e f c | v] - \frac{1}{8} \eta^{a b D} [\mu D^c D^d D^f D | f e c d | v] + \\
& \frac{1}{36} \eta^{a b D} [\mu D^c D^d D^f D | f e d c | v] + \frac{1}{8} \eta^{a b D} [\mu D^c D^d D^f D | f | e v] c d - \frac{1}{8} \eta^{a b D} [\mu D^c D^d D^f D v] e f c d + \\
& \frac{1}{4} e [\mu^{(a} D v) D | c D^c D^d d | e^f | b) f] - \frac{11}{48} e [\mu^{(a} D v) D | c D^c D^d | D b) e^f d f] - \frac{1}{4} e [\mu^{(a} D v) D | c D^c D^d f | e d b) f] + \\
& \frac{11}{48} e [\mu^{(a} D v) D | c D^c D^d f | e b) d f] + \frac{11}{48} e [\mu^{(a} D v) D | c | D b) D^d D c e^f d f] - \frac{1}{4} e [\mu^{(a} D v) D | c | D b) D^d D d e^f c f] - \\
& \frac{11}{48} e [\mu^{(a} D v) D | c | D b) D^d D^f e c d f] + \frac{1}{4} e [\mu^{(a} D v) D | c | D b) D^d D^f e d c f] + \frac{11}{96} e [\mu^{(a} D v) D | c D^d | D c D b) e^f d f] - \\
& \frac{11}{96} e [\mu^{(a} D v) D | c D^d D^c D^f | e b) d f] - \frac{11}{96} e [\mu^{(a} D v) D | c D^d D^d D c e^f | b) f] + \frac{11}{96} e [\mu^{(a} D v) D | c D^d | D d D b) e^f c f] + \\
& \frac{11}{96} e [\mu^{(a} D v) D | c D^d D^d D^f | e c b) f] - \frac{11}{96} e [\mu^{(a} D v) D | c D^d D^d D^f | e b) c f] - \frac{11}{96} e [\mu^{(a} D v) D | c D^d | D b) D c e^f d f] + \\
& \frac{11}{96} e [\mu^{(a} D v) D | c D^d | D b) D^f e c d f] + \frac{11}{96} e [\mu^{(a} D v) D | c D^d D^f | D c e^f b) d] - \frac{11}{96} e [\mu^{(a} D v) D | c D^d D^f | D f e c b) d] \\
& + \frac{11}{96} e [\mu^{(a} D v) D | c D^d D^f | D f e b) c d] - \frac{11}{96} e [\mu^{(a} D v) D | c D^d D^f | D b) e f c d] - \frac{1}{96} f [\mu^c D | c | D v] D (a e | d | b) d \\
& + \frac{1}{96} f [\mu^c D | c | D v] D d e (a b) d + \frac{17}{48} f [\mu^c D | c | D (a D v) e | d | b) d] - \frac{1}{96} f [\mu^c D | c | D (a D b) e^d v] d \\
& - \frac{17}{48} f [\mu^c D | c | D (a D | d | e v) b) d] + \frac{1}{96} f [\mu^c D | c D (a D | d | e b) d | v] + \frac{17}{96} f [\mu^c D | c D^d d | e v] a b - \\
& \frac{1}{96} f [\mu^c D | c D^d d d | e (a b) v] + \frac{1}{16} \eta^{a b f} [\mu^c D | c D^d d d | e^f v] f + \frac{11}{72} e [\mu^{(a} f v) | c D^c D^d d | e^f | b) f] \\
& - \frac{17}{96} f [\mu^c D | c | D^d v] e d a b - \frac{13}{48} \eta^{a b f} [\mu^c D | c | D^d v] e^f d f + \frac{1}{96} f [\mu^c D | c D^d D (a e d | b) v] - \\
& \frac{37}{144} e [\mu^{(a} f v) | c D^c D^d | D b) e^f d f] - \frac{1}{16} \eta^{a b f} [\mu^c D | c D^d D^f e d f | v] - \frac{11}{72} e [\mu^{(a} f v) | c D^c D^d D^f | e d b) f] \\
& + \frac{13}{48} \eta^{a b f} [\mu^c D | c | D^d D^f e v] d f + \frac{37}{144} e [\mu^{(a} f v) | c D^c D^d D^f | e b) d f] - \frac{1}{48} D c D [v e^d (a | d | D \mu) f b) c \\
& + \frac{1}{48} D c D (a e | d | [v | d | D \mu] f b) c - \frac{7}{36} \eta^{a b D} c D d e^f [v | f | D \mu] f^c d - \frac{3}{16} D c D [v e | d | a^b D \mu] f^c d + \\
& \frac{5}{24} D c D [v e (a b) | d | D \mu] f^c d + \frac{17}{48} D c D (a e d b) [v D \mu] f^c d - \frac{3}{16} D c D (a e [v b) | d | D \mu] f^c d - \frac{3}{16} D c D (a e b) [v | d | D \mu] f^c d \\
& - \frac{71}{432} \eta^{a b D} c D [v e^d | f d | D \mu] f^c f + \frac{1}{4} \eta^{a b D} c D d e d [v | f | D \mu] f^c f - \frac{11}{36} \eta^{a b D} c D d e f d [v D \mu] f^c f \\
& + \frac{1}{4} \eta^{a b D} c D d e [v | d f | D \mu] f^c f + \frac{1}{48} D c D (a f | d | d [v e v) b) c - \frac{7}{36} \eta^{a b D} c D d f^f f D [\mu e v] c d \\
& + \frac{1}{6} D c D (a f b) d [v e v] c d - \frac{1}{18} \eta^{a b D} c D d f d f D [\mu e v] c f - \frac{1}{48} D c D [v f^d | d | D \mu] e (a b) c - \\
& \frac{3}{16} D c D [v f (a | d | D \mu) e b) c d] + \frac{3}{16} D c D (a f [v | d | D \mu] e b) c d + \frac{3}{16} D c D [v f^d | d | D \mu] e c a b - \frac{17}{48} D c D (a f | d d D [\mu e c | b) v] \\
& - \frac{3}{16} D c D [v f (a | d | D \mu) e | c | b) d] + \frac{3}{16} D c D (a f [v | d | D \mu] e | c | b) d + \frac{11}{36} \eta^{a b D} c D d f^f f D [\mu e^c d v]
\end{aligned}$$

$$\begin{aligned}
& + \frac{1}{6} D_c D (a f b) d D [\mu e c d v] - \frac{1}{4} \eta a b D_c D d f [v | f | D \mu] e c d f + \frac{71}{432} \eta a b D_c D [v f | d f | D \mu] e c d f \\
& - \frac{1}{18} \eta a b D_c D d f d f D [\mu e c f v] + \frac{1}{48} D_c D [v f (a | d | D \mu)] e | d | b) c - \frac{1}{48} D_c D (a f [v | d | D \mu] e | d | b) c \\
& + \frac{3}{8} D_c D [v f (a b) D \mu] e d c d - \frac{17}{48} D_c D (a f b) [v D \mu] e d c d - \frac{1}{4} \eta a b D_c D d f [v | f | D \mu] e d c f - \\
& \frac{13}{432} \eta a b D_c D [v f | d f | D \mu] e d c f + \frac{13}{432} \eta a b D_c D [v f d | d | D \mu] e f c f + \frac{11}{36} \eta a b D_c D d f d [v D \mu] e f c f \\
& + \frac{7}{36} \eta a b D_c D d f [v | f | D \mu] e f c d - \frac{7}{27} \eta a b e c d f D [\mu D | c D d f f | v] - \frac{7}{36} \eta a b f c d D [\mu D | c D d | e f v] f \\
& + \frac{11}{48} \eta a b e c d f D [\mu D | c | D v] f d f - \frac{3}{16} e (a | c d | D [\mu D | c | D v] f b) d - \frac{3}{16} e c (a | d | D [\mu D | c | D v] f b) d - \\
& \frac{1}{48} e (a b) c D [\mu D | c | D v] f d d + \frac{3}{16} e c a b D [\mu D | c | D v] f d d - \frac{3}{16} f c d D [\mu D | c | D v] e d a b + \frac{7}{48} f c d D [\mu D | c | D v] e (a b) d \\
& + \frac{23}{48} f (a | c D [\mu D | c | D v] e d | b) d - \frac{23}{48} \eta a b f c d D [\mu D | c | D v] e f d f + \frac{17}{48} f c d D [\mu D | c D (a e d | b) v] \\
& - \frac{7}{48} f c d D [\mu D | c | D (a e v) b) d - \frac{1}{6} f c d D [\mu D | c D (a e b) d | v] + \frac{1}{6} e (a | c d | D [\mu D | c D b) f d | v] + \\
& \frac{5}{24} e c (a | d | D [\mu D | c D b) f d | v] - \frac{23}{48} f (a | c | D [\mu D | c | D b) e d v] d - \frac{1}{2} f (a | c D [\mu D | c | D d | e v] b) d + \\
& \frac{1}{2} f (a | c D [\mu D | c D d | e b) d | v] - \frac{11}{36} \eta a b f c d D [\mu D | c D f e d f | v] + \frac{13}{54} \eta a b f c d D [\mu D | c D f e f d | v] \\
& + \frac{55}{108} \eta a b f c d D [\mu D | c | D f e v] d f - \frac{13}{54} \eta a b e c d f D [\mu D | d D c f f | v] + \frac{1}{2} f c d D [\mu D | d D c | e v] a b \\
& - f c d D [\mu D | d D c | e (a b) v] + \frac{2}{3} \eta a b f c d D [\mu D | d D c | e f v] f + \frac{7}{36} \eta a b e c d f D [\mu D | d D f c | e v] + \\
& \frac{5}{144} \eta a b e c d f D [\mu D | d | D v] f c f + \frac{3}{8} e c c d D [\mu D | d | D v] f (a b) + \frac{1}{48} e c (a | d | D [\mu D | d | D v] f b) c - \\
& \frac{5}{144} \eta a b e c c d D [\mu D | d | D v] f f f - \frac{1}{2} f c d D [\mu D | d | D v] e c a b - \frac{17}{48} e c c d D [\mu D | d | D (a f b) v] + f c d D [\mu D | d D (a e c | b) v] \\
& - \frac{1}{48} e c (a | d | D [\mu D | d D b) f c | v] + \frac{11}{36} \eta a b e c c d D [\mu D | d D f f f | v] - \frac{2}{3} \eta a b f c d D [\mu D | d D f e c f | v] - \\
& \frac{17}{48} D_c e d (a d D [\mu D v] f b) c - \frac{3}{16} D_c e d a b D [\mu D v] f c d + \frac{25}{24} D_c e (a b) d D [\mu D v] f c d - \frac{143}{432} \eta a b D_c e d f d D [\mu D v] f c f \\
& - \frac{17}{48} D_c f d d D [\mu D v] e (a b) c - \frac{3}{16} D_c f (a d D [\mu D v] e b) c d + \frac{3}{16} D_c f d d D [\mu D v] e c a b - \frac{3}{16} D_c f (a d D [\mu D v] e | c | b) d \\
& + \frac{71}{432} \eta a b D_c f d f D [\mu D v] e c d f + \frac{17}{48} D_c f (a d D [\mu D v] e | d | b) c + \frac{3}{8} D_c f (a b) D [\mu D v] e d c d - \\
& \frac{13}{432} \eta a b D_c f d f D [\mu D v] e d c f + \frac{13}{432} \eta a b D_c f d d D [\mu D v] e f c f - \frac{1}{3} e (a b) c D [\mu D v] D_c f d d + \\
& \frac{5}{6} f c d D [\mu D v] D_c e (a b) d - \frac{5}{6} f (a | c D [\mu D v] D_c e d | b) d + \frac{1}{3} e c (a | d | D [\mu D v] D d f b) c - \frac{1}{2} f c d D [\mu D v] D (a e c b) d - \\
& \frac{1}{3} f c d D [\mu D v] D (a e d b) c + \frac{4}{3} f c c D [\mu D v] D (a e | d | b) d - \frac{1}{3} e c (a | d | D [\mu D v] D b) f c d + \frac{1}{3} e c (a c D [\mu D v] D b) f d d + \\
& \frac{1}{3} e (a b) c D [\mu D v] D d f c d - \frac{1}{3} e c (a c D [\mu D v] D | d | f b) d + \frac{5}{6} f (a | c D [\mu D v] D d | e c b) d - \frac{4}{3} f c c D [\mu D v] D d e (a b) d + \\
& \frac{17}{48} D_c f d d D [\mu D (a e v) b) c - \frac{1}{3} D_c f d d D [\mu D (a e b) c v] - \frac{17}{48} D_c f d d D [\mu D (a e | c | b) v] - \frac{1}{2} f c d D [\mu D (a D | c | e v) b) d \\
& + \frac{1}{2} f c d D [\mu D (a D | c e b) d | v] + \frac{11}{48} e c c d D [\mu D (a D v] f b) d + \frac{1}{2} f c d D [\mu D (a D v] e c b) d + \frac{5}{48} f c d D [\mu D (a D v] e d b) c \\
& - \frac{11}{48} f c d D [\mu D (a D v] e b) c d - \frac{53}{48} f c c D [\mu D (a D v] e | d | b) d - \frac{11}{48} e c c d D [\mu D (a D b) f | d | v] -
\end{aligned}$$

$$\begin{aligned}
& \frac{1}{2} f^c d D [\mu D (a D b) e | c d | v] - \frac{5}{48} f^c d D [\mu D (a D b) e | d c | v] + \frac{11}{48} f^c d D [\mu D (a D b) e v] c d + \frac{53}{48} f^c c D [\mu D (a D b) e^d v] d \\
& + \frac{4}{3} f^c c D [\mu D (a D | d | e v) b] d - \frac{4}{3} f^c c D [\mu D (a D | d | e b) | d | v] - \frac{1}{3} D c e^d (a d D [\mu D b] f^c v) - \frac{1}{6} D c f (a d D [\mu D b) e v] c^d \\
& - \frac{1}{6} D c f (a d D [\mu D b) e c^d v] + \frac{1}{3} D c f (a d D [\mu D b) e^d c v] + \frac{1}{3} e (a | c d | D [\mu D b) D | c f d | v] + \frac{1}{3} e^c (a | d | D [\mu D b) D | c f d | v] \\
& - \frac{1}{6} f (a | c | D [\mu D b) D | c | e^d v] d - \frac{1}{3} e^c (a | d | D [\mu D b) D | d f c | v] - \frac{11}{48} e (a | c d | D [\mu D b) D v] f c d + \\
& \frac{5}{48} e^c (a | d | D [\mu D b) D v] f c d - \frac{5}{48} e^c (a c D [\mu D b) D v] f^d d + \frac{11}{48} f (a | c | D [\mu D b) D v] e^d c d - \frac{1}{3} e^c (a c D [\mu D b) D d f | d | v] \\
& + \frac{5}{6} f (a | c | D [\mu D b) D d e | c d | v] - \frac{1}{3} f (a | c | D [\mu D b) D d e | d c | v] - \frac{1}{3} f (a | c | D [\mu D b) D d e v] c d + \\
& \frac{17}{48} D c e^d (a d D [\mu D | c | f b) v] + \frac{11}{16} D c e^d a b D [\mu D c f^d v] - \frac{71}{48} D c e (a b) d D [\mu D c f^d v] + \frac{31}{48} \eta^a b D c e^d f d D [\mu D c f^f v] \\
& - \frac{3}{16} D c f^d d D [\mu D c e v] a b + \frac{3}{16} D c f (a d D [\mu D | c | e v] b) d - \frac{11}{48} \eta^a b D c f^d f D [\mu D c e v] d^f + \\
& \frac{17}{48} D c f^d d D [\mu D c e (a b) v] + \frac{3}{16} D c f (a d D [\mu D | c | e b) d v] - \frac{3}{8} D c f (a b) D [\mu D c e^d v] d - \frac{17}{48} D c f (a d D [\mu D | c e d | b) v] \\
& + \frac{11}{144} \eta^a b D c f^d f D [\mu D c e^d f v] - \frac{11}{144} \eta^a b D c f^d d D [\mu D c e^f v] f + \frac{13}{8} f (a b) D [\mu D c D | c | e^d v] d + \\
& \frac{3}{8} f (a b) D [\mu D c D v] e^d c d - 2 f (a b) D [\mu D c D d e | c d | v] - \frac{1}{2} D c e^d a b D [\mu D d f^c v] + \frac{7}{36} \eta^a b D c f^d f D [\mu D d e v] c^f \\
& + \frac{7}{36} \eta^a b D c f^d f D [\mu D d e c^f v] - \frac{11}{36} \eta^a b D c f^d f D [\mu D d e^f c v] + \frac{3}{2} f (a | c D [\mu D d | D | c e d | b) v] \\
& - \frac{13}{24} e (a b) c D [\mu D d D | d f c | v] + \frac{3}{16} e^c a b D [\mu D d D | d f c | v] + \frac{17}{48} e^c (a c D [\mu D | d | D | d | f b) v] - \\
& \frac{89}{48} f (a | c D [\mu D d | D | d e c | b) v] - \frac{19}{16} f^c c D [\mu D d D | d | e v] a b + \frac{9}{8} f (a | c D [\mu D d | D | d | e v) b) c + \\
& \frac{113}{48} f^c c D [\mu D d D | d | e (a b) v] - \frac{13}{16} f (a | c D [\mu D d | D | d e b) c | v] - \frac{235}{144} \eta^a b f^c c D [\mu D d D | d | e^f v] f + \\
& \frac{5}{24} e (a b) c D [\mu D d D v] f c d - \frac{3}{16} e^c a b D [\mu D d D v] f c d - \frac{1}{48} e^c (a c D [\mu D | d | D v] f b) d + \frac{1}{48} f (a | c D [\mu D d | D v] e c b) d \\
& + \frac{19}{16} f^c c D [\mu D d D v] e d a b - \frac{9}{8} f (a | c D [\mu D d | D v] e d b) c - \frac{1}{48} f^c c D [\mu D d D v] e (a b) d - \frac{3}{16} f (a | c D [\mu D d | D v] e b) c d \\
& + \frac{25}{48} \eta^a b f^c c D [\mu D d D v] e^f d f - \frac{113}{48} f^c c D [\mu D d D (a e | d | b) v] + \frac{1}{48} f^c c D [\mu D d D (a e v) b) d + \\
& \frac{55}{48} f (a | c D [\mu D d | D b) e | d c | v] + \frac{3}{16} f (a | c D [\mu D d | D b) e v] c d + \frac{67}{36} \eta^a b f^c c D [\mu D d D f e | d f | v] - \\
& \frac{3}{4} \eta^a b f^c c D [\mu D d D f e v] d f + \frac{11}{36} \eta^a b D c e^d f d D [\mu D f f^c v] + \frac{11}{36} \eta^a b D c f^d d D [\mu D f e | f | c v] - \\
& \frac{7}{18} \eta^a b D c f^d d D [\mu D f e v] f^c + \frac{11}{36} \eta^a b D c f^d d D [\mu D f e^c | f | v] - \frac{1}{9} \eta^a b f^c d D [\mu D f D | c e d f | v] - \\
& \frac{113}{108} \eta^a b f^c d D [\mu D f D | c e f d | v] + \frac{23}{108} \eta^a b f^c d D [\mu D f D | c | e v] d f + \frac{1}{9} \eta^a b f^c d D [\mu D f D | d e c f | v] \\
& - \frac{1}{9} \eta^a b f^c d D [\mu D f D | d e f c | v] + \frac{11}{48} \eta^a b e^c c^d D [\mu D f D | f f d | v] + \frac{29}{36} \eta^a b f^c d D [\mu D f D | f e c d | v] + \\
& \frac{55}{144} \eta^a b f^c d D [\mu D f D | f e d c | v] - \frac{109}{144} \eta^a b f^c d D [\mu D f D | f | e v] c d - \frac{11}{48} \eta^a b e^c c^d D [\mu D f D v] f d f \\
& - \frac{1}{12} \eta^a b f^c d D [\mu D f D v] e c d f - \frac{23}{144} \eta^a b f^c d D [\mu D f D v] e d c f + \frac{109}{144} \eta^a b f^c d D [\mu D f D v] e f c d - \\
& \frac{11}{48} D [\mu D (a e b) c d D v] f c d + \frac{5}{48} D [\mu D (a e | c | b) d D v] f c d + \frac{5}{24} D [\mu D c e (a b) d D v] f c d - \frac{3}{16} D [\mu D c e^d a b D v] f c d
\end{aligned}$$

$$\begin{aligned}
& -\frac{19}{48}\eta^{ab}D[\mu D^ce^d|d|fD_v]f^cf + \frac{11}{48}\eta^{ab}D[\mu D^ce|c|d^fD_v]f^da + \frac{29}{144}\eta^{ab}D[\mu D^ce^d|c|fD_v]f^da \\
& + \frac{3}{8}D[\mu D^ce^d|c^d|D_v]f^{(ab)} + \frac{23}{48}D[\mu D^ce^d(a|d|D_v)f^b]_c + \frac{11}{48}D[\mu D^c(ae|c|c|d|D_v)f^b]_d - \\
& - \frac{3}{16}D[\mu D^ce|c|(a|d|D_v)f^b]_d - \frac{3}{16}D[\mu D^ce(a|c|d|D_v)f^b]_d - \frac{23}{48}D[\mu D^ce^d(a|c|D_v)f^b]_d - \\
& - \frac{11}{48}e[\mu^{(a}D|cD^de|f|b)_{f|}D_v]f^cd - \frac{7}{36}e[\mu^{(a}D|cD^b)e^d_{f|}D_v]f^cf + \frac{11}{48}e[\mu^{(a}D|cD|d|e^db)_{f|}D_v]f^cf \\
& - \frac{11}{48}e[\mu^{(a}D|cD|d|e^fb)_{d|}D_v]f^cf + \frac{11}{48}e[\mu^{(a}D|cD|d|e^b)_{d|}D_v]f^cf - \frac{29}{48}D[\mu D^c(ae|c|b)_{|c|}D_v]f^da \\
& + \frac{3}{16}D[\mu D^ce|c|a^bD_v]f^da + \frac{23}{48}D[\mu D^ce(a^b)_{|c|}D_v]f^da - \frac{5}{144}\eta^{ab}D[\mu D^ce^d|c^d|D_v]f^ff \\
& + \frac{109}{144}\eta^{ab}D[\mu D^cf^dfD_v]e^cd + \frac{15}{16}D[\mu D^cf^d|d|D_v]e^ca^b + \frac{1}{2}D[\mu D^c(af|c^d|D_v)e^cb]_d - \\
& - \frac{9}{8}D[\mu D^cf(a|d|D_v)e^cb]_d - \frac{1}{12}\eta^{ab}D[\mu D^cf^dfD_v]e^dcf - \frac{11}{16}D[\mu D^cf|c|d^dD_v]e^da^b + \frac{5}{48}D[\mu D^c(af|c^d|D_v)e^db]_c \\
& + \frac{1}{48}D[\mu D^cf(a|d|D_v)e^db]_c - \frac{23}{144}\eta^{ab}D[\mu D^cf^dfD_v]e^cd - \frac{1}{48}D[\mu D^cf^d|d|D_v]e^{(ab)}_c \\
& + \frac{7}{48}D[\mu D^cf|c|d^dD_v]e^{(ab)}_d - \frac{11}{48}D[\mu D^c(af|c^d|D_v)e^b]_cd - \frac{3}{16}D[\mu D^cf(a|d|D_v)e^b]_cd - \\
& - \frac{11}{48}e[\mu^{(a}D|cD^df|f|_{f|}D_v]e^b)cd + \frac{11}{48}e[\mu^{(a}D|cD^df|f|_{f|}D_v]e^{(b)}_cd - \frac{11}{48}e[\mu^{(a}D|cD^df^b)_{f|}D_v]e^cdf \\
& + \frac{7}{36}e[\mu^{(a}D|cD^b)f^d_{f|}D_v]e^cdf + \frac{11}{48}D[\mu D^c(af^b)_cD_v]e^cd + \frac{3}{8}D[\mu D^cf(a^b)D_v]e^cd - \\
& - \frac{29}{48}D[\mu D^c(af|c|c|D_v]e^db)_{d|} + \frac{23}{48}D[\mu D^cf(a|c|D_v]e^db)_{d|} - \frac{11}{48}e[\mu^{(a}D|cD^df^b)_{f|}D_v]e^dcf - \\
& - \frac{5}{144}e[\mu^{(a}D|cD^b)f^d_{f|}D_v]e^cdf + \frac{35}{144}\eta^{ab}D[\mu D^cf^d|d|D_v]e^fcf - \frac{23}{48}\eta^{ab}D[\mu D^cf|c|d^dD_v]e^fda + \\
& - \frac{5}{144}e[\mu^{(a}D|cD^b)f^d_{d|}D_v]e^fcf + \frac{11}{48}e[\mu^{(a}D|cD|d|f^b)_{d|}D_v]e^fcf + \frac{11}{48}e[\mu^{(a}D|cD^df^b)_{f|}D_v]e^fcf \\
& - \frac{109}{144}\eta^{ab}D[\mu e^cdfD_v]D^cf^da + \frac{3}{16}D[\mu e(a|c^d|D_v]D^cf^b)_{d|} + \frac{9}{8}D[\mu e^c(a|d|D_v]D^cf^b)_{d|} + \\
& - \frac{1}{48}D[\mu e^{(ab)}_cD_v]D^cf^da - \frac{15}{16}D[\mu e^cabD_v]D^cf^da + \frac{3}{16}D[\mu f^cdD_v]D^ce^da^b - \frac{5}{24}D[\mu f^cdD_v]D^ce^{(ab)}_d \\
& - \frac{23}{48}D[\mu f(a|cD_v]D^ce^db)_{d|} + \frac{19}{48}\eta^{ab}D[\mu f^cdD_v]D^ce^fda - \frac{17}{72}e[\mu^{(a}e|c^df|D_v]D^cd^df^b)_{f|} \\
& + \frac{7}{36}\eta^{ab}e[\mu^cdD_v]D^cd^df^ff - \frac{11}{48}e[\mu^{(a}e^b)_cD_v]D^cd^df^ff - \frac{11}{36}\eta^{ab}e^c[\mu^dD_v]D^cd^df^ff \\
& + \frac{11}{48}e[\mu^{(a}e|c|b)_{d|}D_v]D^cd^df^ff - \frac{11}{48}e[\mu^{(a}f|c^dD_v]D^cd^de^f|b)_{f|} - \frac{3}{16}e[\mu^cdD_v]D^cd^{(af^b)}_d \\
& - \frac{7}{48}e^c[\mu^dD_v]D^cd^{(af^b)}_d + \frac{97}{96}f[\mu^cD_v]D^cd^{(ae|d|b)}_d + \frac{13}{48}e[\mu^{(a}e|c^df|D_v]D^cd^b)f^da \\
& - \frac{1}{48}e[\mu^{(a|c|D_v]D^cd^b)f^d]_d + \frac{17}{48}e^c(a[\mu D_v]D^cd^b)f^d - \frac{7}{12}e[\mu^{(a}f|c^d|D_v]D^cd^b)e^fda - \\
& - \frac{97}{96}f[\mu^cD_v]D^cd^de^{(ab)}_d + \frac{7}{108}\eta^{ab}e[\mu^cdD_v]D^cd^ffda - \frac{1}{144}e[\mu^{(a}e^b)_cD_v]D^cd^ffda + \\
& - \frac{5}{108}\eta^{ab}e^c[\mu^dD_v]D^cd^ffda + \frac{1}{144}e[\mu^{(a}e|c|b)_{d|}D_v]D^cd^ffda - \frac{11}{48}e[\mu^{(a}f|c^dD_v]D^cd^f|e^db)_{f|} \\
& + \frac{2}{9}e[\mu^{(a}f|c^dD_v]D^cd^f|e^b)_{d|} + \frac{79}{144}e[\mu^{(a}f|c^dD_v]D^cd^f|e^b)_{d|} - \frac{5}{144}\eta^{ab}D[\mu e^cdfD_v]D^dfcf \\
& - \frac{3}{8}D[\mu e^c|c|d^dD_v]D^df^{(ab)} - \frac{1}{48}D[\mu e^c(a|d|D_v]D^df^b)_c - \frac{35}{144}\eta^{ab}D[\mu e^c|c|d^dD_v]D^df^ff -
\end{aligned}$$

$$\begin{aligned}
& \frac{2}{9}e_{[\mu} (a e | c d f | D_{\nu}] D_d D_c f b)_{\mathfrak{f}} + \frac{11}{48}e_{[\mu} (a e | c d f | D_{\nu}] D_d D_{\mathfrak{f}} f b)_{\mathfrak{c}} + \frac{1}{24}e_{[\mu} (a e | c d f | D_{\nu}] D_d D^b)_{\mathfrak{f}} f_{\mathfrak{c}} - \\
& \frac{1}{24}e_{[\mu} (a e | c | c | d | D_{\nu}] D_d D^b)_{\mathfrak{f}} f_{\mathfrak{f}} + \frac{11}{48}e_{[\mu} (a e | c | c | d | D_{\nu}] D_d D_{\mathfrak{f}} f b)_{\mathfrak{f}} + \frac{5}{18}\eta^{ab} D_{[\mu} e^{cd} f D_{\nu]} D_{\mathfrak{f}} f_{\mathfrak{c}} d - \\
& \frac{11}{48}D_{[\mu} e^c | c | d | D_{\nu]} D (a f b)_{\mathfrak{d}} - \frac{17}{48}D_{\mathfrak{c}} e^d | \mu | d | D_{\nu]} D (a f b)_{\mathfrak{c}} - \frac{5}{48}D_{[\mu} f^c d | D_{\nu]} D (a e d b)_{\mathfrak{c}} + \frac{11}{48}D_{[\mu} f^c d | D_{\nu]} D (a e b)_{\mathfrak{c}} d \\
& - \frac{25}{48}D_{\mathfrak{c}} f | \mu | d | D_{\nu]} D (a e b)_{\mathfrak{c}} d - \frac{25}{48}D_{\mathfrak{c}} f | \mu | d | D_{\nu]} D (a e | c | b)_{\mathfrak{d}} + \frac{29}{48}D_{[\mu} f^c | c | D_{\nu]} D (a e | d | b)_{\mathfrak{d}} + \\
& \frac{17}{48}D_{\mathfrak{c}} f | \mu | d | D_{\nu]} D (a e | d | b)_{\mathfrak{c}} + \frac{1}{3}e_{[\mu} e^{cd} D_{\nu]} D (a d_{\mathfrak{c}} f b)_{\mathfrak{d}} + \frac{1}{3}e^c | \mu | d | D_{\nu]} D (a d_{\mathfrak{c}} f b)_{\mathfrak{d}} - \frac{11}{16}f_{[\mu} e^c D_{\nu]} D (a d_{\mathfrak{c}} e | d | b)_{\mathfrak{d}} \\
& - \frac{1}{3}e^c | \mu | d | D_{\nu]} D (a d_{\mathfrak{d}} f b)_{\mathfrak{c}} - \frac{11}{48}e_{[\mu} e^{cd} D_{\nu]} D (a d b)_{\mathfrak{f}} f_{\mathfrak{c}} d + \frac{5}{48}e^c | \mu | d | D_{\nu]} D (a d b)_{\mathfrak{f}} f_{\mathfrak{c}} d - \frac{5}{48}e^c | \mu | c | D_{\nu]} D (a d b)_{\mathfrak{f}} f_{\mathfrak{d}} d \\
& + \frac{71}{96}f_{[\mu} e^c D_{\nu]} D (a d b)_{\mathfrak{e}} d_{\mathfrak{c}} d - \frac{1}{3}e^c | \mu | c | D_{\nu]} D (a d | d | f b)_{\mathfrak{d}} + \frac{65}{48}f_{[\mu} e^c D_{\nu]} D (a d | d | e c b)_{\mathfrak{d}} - \\
& \frac{1}{3}f_{[\mu} e^c D_{\nu]} D (a d | d | e d b)_{\mathfrak{c}} - \frac{27}{32}f_{[\mu} e^c D_{\nu]} D (a d | d | e b)_{\mathfrak{c}} d + \frac{11}{48}D_{[\mu} e (a | c d | D_{\nu]} D b)_{\mathfrak{f}} f_{\mathfrak{c}} d - \frac{29}{48}D_{[\mu} e^c (a | d | D_{\nu]} D b)_{\mathfrak{f}} f_{\mathfrak{c}} d \\
& - \frac{17}{48}D_{\mathfrak{c}} e d (a | \mu D_{\nu]} D b)_{\mathfrak{f}} f_{\mathfrak{c}} d + \frac{11}{16}D_{\mathfrak{c}} e | \mu | a | d | D_{\nu]} D b)_{\mathfrak{f}} f_{\mathfrak{c}} d - \frac{5}{16}D_{\mathfrak{c}} e (a | \mu | d | D_{\nu]} D b)_{\mathfrak{f}} f_{\mathfrak{c}} d - \\
& \frac{7}{36}e_{[\mu} (a d | c e | d | f_{\mathfrak{d}} | D_{\nu]} D b)_{\mathfrak{f}} f_{\mathfrak{c}} f + \frac{29}{48}D_{[\mu} e^c (a | c | D_{\nu]} D b)_{\mathfrak{f}} f_{\mathfrak{d}} d + \frac{7}{36}e_{[\mu} (a d | c f_{\mathfrak{d}} d | D_{\nu]} D b)_{\mathfrak{e}} e^{cd} f \\
& - \frac{11}{48}D_{[\mu} f (a | c | D_{\nu]} D b)_{\mathfrak{e}} d_{\mathfrak{c}} d + \frac{17}{48}D_{\mathfrak{c}} f (a | \mu D_{\nu]} D b)_{\mathfrak{e}} d_{\mathfrak{c}} d - \frac{5}{144}e_{[\mu} (a d | c f_{\mathfrak{d}} d | D_{\nu]} D b)_{\mathfrak{e}} d_{\mathfrak{c}} f \\
& + \frac{5}{144}e_{[\mu} (a d | c f | d | d | D_{\nu]} D b)_{\mathfrak{e}} f_{\mathfrak{c}} f - \frac{1}{3}e_{[\mu} (a | c | D_{\nu]} D b)_{\mathfrak{d}} D_{\mathfrak{c}} f_{\mathfrak{d}} d + \frac{1}{3}e (a | \mu | c | D_{\nu]} D b)_{\mathfrak{d}} D_{\mathfrak{c}} f_{\mathfrak{d}} d \\
& - \frac{5}{8}D_{\mathfrak{c}} e^d | \mu | d | D_{\nu]} D c f (a b) + \frac{65}{48}D_{\mathfrak{c}} e d (a | \mu D_{\nu]} D | c | f b)_{\mathfrak{d}} - \frac{9}{8}D_{\mathfrak{c}} e | \mu | (a | d | D_{\nu]} D | c | f b)_{\mathfrak{d}} + \\
& \frac{13}{16}D_{\mathfrak{c}} e (a | \mu | d | D_{\nu]} D | c | f b)_{\mathfrak{d}} + \frac{7}{12}e_{[\mu} (a d | c e | d_{\mathfrak{f}} d | D_{\nu]} D c | f b)_{\mathfrak{f}} + \frac{15}{16}D_{\mathfrak{c}} e | \mu | a b D_{\nu]} D c f_{\mathfrak{d}} d - \\
& \frac{89}{48}D_{\mathfrak{c}} e (a b)_{[\mu} D_{\nu]} D c f_{\mathfrak{d}} d - \frac{23}{36}\eta^{ab} D_{\mathfrak{c}} e d | \mu | f | D_{\nu]} D c f_{\mathfrak{d}} f + \frac{5}{48}e_{[\mu} (a d | c e d b)_{\mathfrak{f}} | D_{\nu]} D c f_{\mathfrak{d}} f + \\
& \frac{109}{144}\eta^{ab} D_{\mathfrak{c}} e | \mu | d f | D_{\nu]} D c f_{\mathfrak{d}} f - \frac{11}{12}e_{[\mu} (a d | c e b)_{\mathfrak{d}} f | D_{\nu]} D c f_{\mathfrak{d}} f + \frac{49}{48}\eta^{ab} D_{\mathfrak{c}} e d | \mu | d | D_{\nu]} D c f_{\mathfrak{f}} f - \\
& \frac{7}{24}e_{[\mu} (a d | c e | d | b)_{\mathfrak{d}} | D_{\nu]} D c f_{\mathfrak{f}} f - \frac{55}{144}\eta^{ab} D_{\mathfrak{c}} e d | \mu | f | D_{\nu]} D c f_{\mathfrak{f}} f + \frac{3}{16}e_{[\mu} (a d | c e d b)_{\mathfrak{f}} | D_{\nu]} D c f_{\mathfrak{f}} f \\
& + \frac{13}{24}D_{\mathfrak{c}} f | \mu | d | D_{\nu]} D c e (a b)_{\mathfrak{d}} - \frac{13}{48}e_{[\mu} (a d | c f_{\mathfrak{d}} f | D_{\nu]} D | c | e b)_{\mathfrak{d}} f_{\mathfrak{d}} - \frac{3}{8}D_{[\mu} f (a b)_{\mathfrak{d}} D_{\nu]} D c e^d_{\mathfrak{c}} d - \\
& \frac{3}{16}D_{\mathfrak{c}} f | \mu | d | D_{\nu]} D c e^d a b - \frac{17}{48}D_{\mathfrak{c}} f (a | \mu D_{\nu]} D | c e^d | b)_{\mathfrak{d}} - \frac{1}{24}e_{[\mu} (a d | c f_{\mathfrak{d}} f | D_{\nu]} D | c e^d | b)_{\mathfrak{f}} + \\
& \frac{1}{24}e_{[\mu} (a d | c f | d_{\mathfrak{d}} | D_{\nu]} D c e^f | b)_{\mathfrak{f}} - \frac{11}{48}\eta^{ab} D_{\mathfrak{c}} f | \mu | d | D_{\nu]} D c e^f_{\mathfrak{d}} f + \frac{13}{48}e_{[\mu} (a d | c f b)_{\mathfrak{d}} | D_{\nu]} D c e^f_{\mathfrak{d}} f + \\
& \frac{3}{16}e_{[\mu} a b D_{\nu]} D c D_{\mathfrak{c}} f_{\mathfrak{d}} d - \frac{17}{48}e (a b)_{[\mu} D_{\nu]} D c D_{\mathfrak{c}} f_{\mathfrak{d}} d + \frac{31}{144}f (a | \mu D_{\nu]} D | c D_{\mathfrak{c}} e^d | b)_{\mathfrak{d}} - \frac{5}{72}f (a | \mu D_{\nu]} D | c | D b)_{\mathfrak{e}} d_{\mathfrak{c}} d \\
& - \frac{41}{72}f (a | \mu D_{\nu]} D | c D^d | e c b)_{\mathfrak{d}} + \frac{61}{144}f (a | \mu D_{\nu]} D | c D^d | e b)_{\mathfrak{c}} d - \frac{7}{48}D_{[\mu} e (a b)_{\mathfrak{c}} D_{\nu]} D^d f_{\mathfrak{c}} d + \\
& \frac{11}{16}D_{[\mu} e^c a b D_{\nu]} D^d f_{\mathfrak{c}} d - \frac{1}{2}D_{\mathfrak{c}} e | \mu | a b D_{\nu]} D^d f_{\mathfrak{d}} c + D_{\mathfrak{c}} e (a b)_{[\mu} D_{\nu]} D^d f_{\mathfrak{d}} c - \frac{23}{48}D_{[\mu} e^c (a | c | D_{\nu]} D | d | f b)_{\mathfrak{d}} \\
& - D_{\mathfrak{c}} e d (a | \mu D_{\nu]} D | d | f b)_{\mathfrak{c}} + \frac{23}{36}\eta^{ab} D_{\mathfrak{c}} e d | \mu | f | D_{\nu]} D^d f_{\mathfrak{c}} f - \frac{5}{48}e_{[\mu} (a d | c e d b)_{\mathfrak{f}} | D_{\nu]} D^d f_{\mathfrak{c}} f - \\
& \frac{17}{36}\eta^{ab} D_{\mathfrak{c}} e | \mu | d f | D_{\nu]} D^d f_{\mathfrak{c}} f + \frac{9}{16}e_{[\mu} (a d | c e b)_{\mathfrak{d}} f | D_{\nu]} D^d f_{\mathfrak{c}} f + \frac{1}{9}\eta^{ab} D_{\mathfrak{c}} e d | \mu | f | D_{\nu]} D^d f_{\mathfrak{f}} c \\
& + \frac{23}{48}D_{[\mu} f (a | c D_{\nu]} D^d | e c b)_{\mathfrak{d}} - \frac{3}{16}D_{[\mu} f^c | c | D_{\nu]} D^d e d a b + \frac{3}{16}D_{[\mu} f (a | c D_{\nu]} D^d | e d b)_{\mathfrak{c}}
\end{aligned}$$

$$\begin{aligned}
& \frac{23}{48} D_{[\mu} f^c |c| D_{\nu]} D^d e^{(ab)}_d + \frac{3}{16} D_{[\mu} f^c (a |c D_{\nu]} D^d |e b)_c d + \frac{11}{48} e_{[\mu} (a D |c f^c_d | D_{\nu]} D^d |d |e b)_c f + \\
& \frac{11}{48} e_{[\mu} (a D |c f^c_d | D_{\nu]} D^d |d e |c b)_f + \frac{5}{144} \eta^{ab} D_{[\mu} f^c |c| D_{\nu]} D^d e^f_d f - \frac{11}{48} e_{[\mu} (a D |c f^c_d | D_{\nu]} D^d |d e f |b)_c \\
& - \frac{11}{36} \eta^{ab} D_{c f} [\mu |d | D_{\nu]} D^d e^f_c f + \frac{11}{48} e_{[\mu} (a D |c f^c_b)_d | D_{\nu]} D^d e^f_c f + \frac{97}{96} f_{[\mu}^c D_{\nu]} D^d D_c e^f_d a b \\
& + \frac{59}{144} \eta^{ab} f_{[\mu}^c D_{\nu]} D^d D_c e^f_d f - \frac{5}{48} e_{[\mu} (a f^c b)_c D_{\nu]} D^d D_c e^f_d f + \frac{3}{8} e^c_{[\mu} |c| D_{\nu]} D^d D_d f^{(ab)} \\
& - \frac{3}{16} e_{[\mu} (a |c D_{\nu]} D^d |D_d f^b)_c - \frac{3}{16} e_{[\mu} (a |c D_{\nu]} D^d |D_d f^b)_c + \frac{17}{48} e^c (a_{[\mu} D_{\nu]} D^d |D_d f^b)_c + \\
& \frac{11}{144} \eta^{ab} e^c_{[\mu} |c| D_{\nu]} D^d D_d f^f_f + \frac{1}{24} e_{[\mu} (a e |c |b)_c |c| D_{\nu]} D^d D_d f^f_f - \frac{115}{96} f_{[\mu}^c D_{\nu]} D^d D_d e^f_c a b \\
& + \frac{191}{96} f_{[\mu}^c D_{\nu]} D^d D_d e^{(ab)}_c - \frac{107}{72} \eta^{ab} f_{[\mu}^c D_{\nu]} D^d D_d e^f_c f + \frac{11}{12} e_{[\mu} (a f^c b)_c D_{\nu]} D^d D_d e^f_c f \\
& - \frac{5}{8} e_{[\mu} (a f^c |c |c | D_{\nu]} D^d D_d e^f |b)_f - \frac{1}{48} e^c_{[\mu} |c| D_{\nu]} D^d D_d (a f^c b)_d + \frac{1}{48} f_{[\mu}^c D_{\nu]} D^d D_d (a e^c b)_d - \\
& \frac{53}{32} f_{[\mu}^c D_{\nu]} D^d D_d (a e^c b)_c - \frac{1}{6} f_{[\mu}^c D_{\nu]} D^d D_d (a e^c b)_c d + \frac{5}{24} e_{[\mu} (a |c D_{\nu]} D^d |D_d b)_f c d + \frac{1}{6} e_{[\mu} (a |c D_{\nu]} D^d |D_d b)_f c d \\
& - \frac{17}{48} e^c (a_{[\mu} D_{\nu]} D^d |D_d b)_f c d + \frac{5}{8} e_{[\mu} (a f^c |c |c | D_{\nu]} D^d |D_d b)_e f_d f + \frac{7}{36} \eta^{ab} e^c_{[\mu} |c| D_{\nu]} D^d D_d f^f_d f - \\
& \frac{11}{48} e_{[\mu} (a e |c |b)_c |c| D_{\nu]} D^d D_d f^f_d f - \frac{131}{144} \eta^{ab} f_{[\mu}^c D_{\nu]} D^d D_d f^f_e c d f + \frac{9}{16} e_{[\mu} (a f^c b)_c D_{\nu]} D^d D_d f^f_e c d f + \\
& \frac{655}{432} \eta^{ab} f_{[\mu}^c D_{\nu]} D^d D_d f^f_e d c f - \frac{127}{144} e_{[\mu} (a f^c b)_c D_{\nu]} D^d D_d f^f_e d c f + \frac{43}{48} e_{[\mu} (a f^c |c |c | D_{\nu]} D^d D_d f^f |e d b)_f \\
& + \frac{13}{54} \eta^{ab} f_{[\mu}^c D_{\nu]} D^d D_d f^f_e f c d - \frac{2}{9} e_{[\mu} (a f^c b)_c D_{\nu]} D^d D_d f^f_e f c d - \frac{43}{48} e_{[\mu} (a f^c |c |c | D_{\nu]} D^d D_d f^f |e b)_d f + \\
& \frac{23}{48} \eta^{ab} D_{[\mu} e^c |c| D_{\nu]} D^d f^f_d f - \frac{1}{9} \eta^{ab} D_{c e^d} [\mu |d | D_{\nu]} D^d f^f_f c - \frac{11}{24} e_{[\mu} (a D |c e |d |b)_d | D_{\nu]} D^d f^f_f c + \\
& \frac{11}{48} e_{[\mu} (a D |c e |d^f_d | D_{\nu]} D^d |f |f b)_c + \frac{5}{12} \eta^{ab} D_{c e^d} [\mu |f | D_{\nu]} D^d f^f_c d - \frac{11}{48} e_{[\mu} (a D |c e^d b)_f | D_{\nu]} D^d f^f_c d \\
& - \frac{1}{9} \eta^{ab} D_{c e^d} [\mu |f | D_{\nu]} D^d f^f_d c - \frac{13}{36} \eta^{ab} D_{[\mu} f^c d D_{\nu]} D^d f^f_e c d f + \frac{23}{144} \eta^{ab} D_{[\mu} f^c d D_{\nu]} D^d f^f_e d c f - \\
& \frac{11}{48} \eta^{ab} D_{[\mu} f^c d D_{\nu]} D^d f^f_e f c d + \frac{11}{48} e_{[\mu} (a D |c f^c |d | D_{\nu]} D^d |f |e f b)_c + \frac{1}{2} \eta^{ab} D_{c f} [\mu |d | D_{\nu]} D^d f^f_e f c d - \\
& \frac{11}{24} e_{[\mu} (a D |c f^c b)_d | D_{\nu]} D^d f^f_e f c d - \frac{11}{24} e_{[\mu} (a D |c f^c |d | D_{\nu]} D^d |f |e b)_f c + \frac{1}{2} \eta^{ab} D_{c f} [\mu |d | D_{\nu]} D^d f^f_e f c d - \\
& \frac{11}{24} e_{[\mu} (a D |c f^c b)_d | D_{\nu]} D^d f^f_e f c d + \frac{11}{48} e_{[\mu} (a D |c f^c |d | D_{\nu]} D^d f^f_e c |b)_f - \frac{7}{18} \eta^{ab} D_{c f} [\mu |d | D_{\nu]} D^d f^f_e d f c \\
& + \frac{11}{24} e_{[\mu} (a D |c f^c b)_d | D_{\nu]} D^d f^f_e d f c - \frac{7}{27} \eta^{ab} e_{[\mu}^c d D_{\nu]} D^d f^f_c d f + \frac{17}{72} e_{[\mu} (a e^c b)_c d D_{\nu]} D^d f^f_c d f - \\
& \frac{13}{54} \eta^{ab} e^c_{[\mu} d D_{\nu]} D^d f^f_c d f + \frac{2}{9} e_{[\mu} (a e |c |b)_c d D_{\nu]} D^d f^f_c d f - \frac{47}{144} e_{[\mu} (a f^c |c d D_{\nu]} D^d |D_c e^f b)_d + \\
& \frac{47}{144} e_{[\mu} (a f^c |c d D_{\nu]} D^d |D_c e^f b)_d f + \frac{11}{36} \eta^{ab} e^c_{[\mu} d D_{\nu]} D^d f^f_d f c f - \frac{11}{48} e_{[\mu} (a e |c |b)_c d D_{\nu]} D^d f^f_d f c f \\
& + \frac{11}{48} \eta^{ab} e_{[\mu}^c d D_{\nu]} D^d f^f_d f c d - \frac{13}{48} e_{[\mu} (a e^c b)_c d D_{\nu]} D^d f^f_d f c d - \frac{11}{144} \eta^{ab} e^c_{[\mu} d D_{\nu]} D^d f^f_d f c d - \\
& \frac{1}{24} e_{[\mu} (a e |c |b)_c d D_{\nu]} D^d f^f_d f c d + \frac{13}{48} e_{[\mu} (a e |c |c |d D_{\nu]} D^d |D_d f^f b)_d + \frac{5}{48} e_{[\mu} (a f^c |c d D_{\nu]} D^d |D_d f^f_e c b)_d \\
& + \frac{3}{16} e_{[\mu} (a f^c |c d D_{\nu]} D^d |D_d f^f_e d b)_c - \frac{11}{12} e_{[\mu} (a f^c |c d D_{\nu]} D^d |D_d f^f_e b)_c d - \frac{13}{48} e_{[\mu} (a e |c |c |d D_{\nu]} D^d |D_d b)_f d f \\
& - \frac{5}{48} e_{[\mu} (a f^c |c d D_{\nu]} D^d |D_d b)_e c d f - \frac{3}{16} e_{[\mu} (a f^c |c d D_{\nu]} D^d |D_d b)_e d c f + \frac{11}{12} e_{[\mu} (a f^c |c d D_{\nu]} D^d |D_d b)_e f c d -
\end{aligned}$$

$$\begin{aligned}
& \frac{17}{48} D [\mu D^c e^d | c d] D (a f b) v_j + \frac{17}{48} D [\mu D | c] e^d v_j d D (a f b) c + \frac{11}{48} D [\mu D v_j] e^d c d D (a f b) c + \frac{1}{3} D [\mu D d e | c d] v_j D (a f b) c - \\
& \frac{3}{16} D [\mu D d e | d c] v_j D (a f b) c - \frac{7}{48} D [\mu D d e v_j] c d D (a f b) c + \frac{17}{48} D [\mu D | c f d] d D (a e v_j) b) c - \frac{7}{48} D [\mu D d f | c d] D (a e v_j) b) c \\
& - \frac{1}{3} D [\mu D | c f d] d D (a e b) v_j c - \frac{1}{6} D [\mu D d f | c d] D (a e b) v_j c + \frac{1}{2} D [\mu D | c f d] v_j D (a e b) c d - \frac{11}{48} D [\mu D v_j] f c d D (a e b) c d \\
& + \frac{35}{48} D [\mu D v_j] f^d d D (a e | c | b) c - \frac{5}{6} D [\mu D d f | d] v_j D (a e | c | b) c - \frac{89}{48} D [\mu D | c f d] d D (a e | c | b) v_j + \\
& \frac{65}{48} D [\mu D d f | c d] D (a e | c | b) v_j + \frac{71}{48} D [\mu D | c f d] v_j D (a e | c | b) d - \frac{17}{48} D [\mu D | d f c] v_j D (a e | c | b) d \\
& - \frac{35}{48} D [\mu D v_j] f c d D (a e | c | b) d - \frac{17}{96} f [\mu^c D (a D | c | D v_j) e | d | b] d - \frac{1}{6} f [\mu^c D (a D | c | D b) e^d v_j] d + \\
& \frac{17}{96} f [\mu^c D (a D | c | D | d | e v_j) b] d + \frac{1}{6} f [\mu^c D (a D | c D | d | e b) d] v_j + \frac{11}{48} D [\mu e^d | c d] D (a D v_j) f b) c - \\
& \frac{11}{48} D [\mu f | c d] D (a D v_j) e b) c d - \frac{53}{48} D [\mu f^d | d] D (a D v_j) e | c | b) c + \frac{29}{48} D [\mu f | c d] D (a D v_j) e | c | b) d + \\
& \frac{17}{96} f [\mu^c D (a D v_j) D c e | d | b] d - \frac{1}{6} f [\mu^c D (a D v_j) D b) e^d c d - \frac{17}{96} f [\mu^c D (a D v_j) D | d | e c b) d + \frac{1}{6} f [\mu^c D (a D v_j) D | d | e b) c d - \\
& \frac{11}{48} D [\mu e^d | c d] D (a D b) f v_j c + \frac{5}{48} D [\mu e^d v_j] d D (a D b) f c c - \frac{5}{48} D [\mu e | d c] v_j D (a D b) f c d + \frac{11}{48} D [\mu e v_j] c d D (a D b) f c d \\
& + \frac{11}{48} D [\mu f | c d] D (a D b) e v_j c d - \frac{35}{48} D [\mu f | d] v_j D (a D b) e^c c d + \frac{53}{48} D [\mu f^d | d] D (a D b) e^c v_j c \\
& - \frac{29}{48} D [\mu f | c d] D (a D b) e^c v_j d + \frac{17}{96} f [\mu^c D (a D b) D | c | e^d v_j] d - \frac{17}{96} f [\mu^c D (a D b) D v_j] e^d c d - \\
& \frac{17}{96} f [\mu^c D (a D b) D d e | c d] v_j + \frac{17}{96} f [\mu^c D (a D b) D d e v_j] c d + \frac{1}{3} D [\mu e^d v_j] d D (a D | c | f b) c - \frac{1}{3} D [\mu e | c d] v_j D (a D | c | f b) d \\
& + \frac{1}{3} D [\mu e | d c] v_j D (a D | c | f b) d - \frac{1}{3} D [\mu e v_j] c d D (a D | c | f b) d + \frac{1}{3} D [\mu f | d] v_j D (a D | c | e c b) d + \\
& \frac{4}{3} D [\mu f^d | d] D (a D | c | e v_j) b) c - \frac{1}{2} D [\mu f | c d] D (a D | c | e v_j) b) d - \frac{4}{3} D [\mu f^d | d] D (a D | c | e b) c | v_j + \\
& \frac{5}{6} D [\mu f | d] v_j D (a D | c | e b) c d + \frac{1}{2} D [\mu f | c d] D (a D | c | e b) v_j d - \frac{4}{3} D [\mu f | d] v_j D (a D | c e d | b) c + \\
& \frac{2}{3} D [\mu f | c | v_j] D (a D | c e d | b) d - \frac{17}{96} f [\mu^c D (a D | d | D | c e d | b) v_j] + \frac{17}{96} f [\mu^c D (a D | d | D | d e c | b) v_j] \\
& - \frac{17}{96} f [\mu^c D (a D | d | D | d | e v_j) b) c - \frac{1}{6} f [\mu^c D (a D | d | D | d e b) c | v_j] + \frac{17}{96} f [\mu^c D (a D | d | D v_j) e d b) c \\
& + \frac{1}{6} f [\mu^c D (a D | d | D b) e | d c | v_j] - \frac{1}{3} D [\mu D | c e^d (a d | D b) f v_j] c - \frac{11}{24} D [\mu D (a e | d | | c d | D b) f v_j] c - \\
& \frac{17}{48} D [\mu D d e | c (a d | D b) f v_j] c + \frac{13}{24} D [\mu D d e | d (a c | D b) f v_j] c + \frac{1}{2} D [\mu D d e (a | c d | D b) f v_j] c - \frac{13}{48} D [\mu D v_j] e^d (a d D b) f c c \\
& + \frac{17}{24} D [\mu D (a e | d | v_j) d D b) f c c - \frac{17}{48} D [\mu D d e | d | (a v_j) D b) f c c + \frac{41}{48} D [\mu D d e v_j] (a d D b) f c c - \\
& \frac{5}{6} D [\mu D d e (a | d | v_j) D b) f c c - \frac{1}{24} e [\mu (a D v_j) D | d e f | d f D b) f c c + \frac{17}{48} D [\mu D | c e d | (a v_j) D b) f c d - \\
& \frac{17}{24} D [\mu D | c | e v_j] (a d D b) f c d + \frac{1}{3} D [\mu D | c e (a d | v_j) D b) f c d + \frac{1}{2} D [\mu D v_j] e c (a d D b) f c d - \frac{11}{48} D [\mu D v_j] e d (a c D b) f c d - \\
& \frac{11}{48} D [\mu D v_j] e (a c d D b) f c d - \frac{1}{2} D [\mu D (a e | c d | v_j) D b) f c d - \frac{5}{24} D [\mu D (a e | d c | v_j) D b) f c d + \frac{11}{24} D [\mu D (a e v_j) c d D b) f c d \\
& - \frac{13}{48} e [\mu (a D v_j) D c e | f | d f D b) f c d + \frac{11}{48} e [\mu (a D v_j) D | f | e c d f D b) f c d - \frac{3}{16} e [\mu (a D v_j) D | f | e d c f D b) f c d \\
& + \frac{13}{48} e [\mu (a D v_j) D | f | e f c d D b) f c d - \frac{7}{48} D [\mu D | c f (a d | D b) e v_j] c d + \frac{11}{24} D [\mu D (a f | c d | D b) e v_j] c d
\end{aligned}$$



$$\begin{aligned}
& -\frac{17}{48}D[\mu D|d|f(a_v)Db)e^c c^d + \frac{11}{48}D[\mu D_v]f(a_d Db)e^c c^d - \frac{11}{24}D[\mu D(a_f|d|v)Db)e^c c^d + \\
& \frac{7}{24}e[\mu(aD_v)D_d f|f|fDb)e^c c^d - \frac{7}{12}e[\mu(aD_v)D|f|f_d fDb)e^c c^d + \frac{17}{24}D[\mu D(a_f|d|d|Db)e^c v]c \\
& -\frac{7}{48}D[\mu D_d f(a|d|Db)e^c v]c + \frac{13}{16}D[\mu D|c f(a_d|Db)e^c v]d + \frac{1}{3}D[\mu D|d f(a_c|Db)e^c v]d - \\
& \frac{17}{24}D[\mu D(a_f|c_d|Db)e^c v]d + \frac{11}{12}e[\mu(aD_v)D_c f_d fDb)e^c d f + \frac{1}{24}e[\mu(aD_v)D_d f_c fDb)e^c d f \\
& -\frac{1}{3}e[\mu(aD_v)D_f f_c d Db)e^c d f - \frac{5}{48}D[\mu e_d(a|d|Db)D_v]f_c c + \frac{5}{48}D[\mu e|d(a_c|Db)D_v]f_c d - \\
& \frac{11}{48}D[\mu e(a|c_d|Db)D_v]f_c d + \frac{11}{48}D[\mu f(a|d|Db)D_v]e^c c^d - \frac{1}{3}D[\mu e_d(a|d|Db)D_c f_c|v] + \frac{1}{3}D[\mu e|c(a_d|Db)D_c f_v]d \\
& -\frac{1}{3}D[\mu e|d(a_c|Db)D_c f_v]d + \frac{1}{3}D[\mu e(a|c_d|Db)D_c f_v]d + \frac{1}{3}D[\mu e_v(a_c|Db)D_c f_d]d - \frac{1}{3}D[\mu e(a|c|v)Db)D_c f_d]d \\
& -\frac{1}{3}D[\mu f(a|d|Db)D_c e_c|v]d - \frac{1}{3}D[\mu f(a|d|Db)D_c e_v]c^d + \frac{5}{6}D[\mu f(a|d|Db)D_c e_d|c|v] - \frac{1}{6}D[\mu f(a|c|Db)D_c e_d|v]d \\
& -\frac{1}{72}f(a[\mu Db)D^c D|c|e^d v]d + \frac{29}{144}f(a[\mu Db)D^c D_v]e^d c^d + \frac{1}{72}f(a[\mu Db)D^c D_e|c_d|v] - \\
& \frac{29}{144}f(a[\mu Db)D^c D_d e_v]c^d + \frac{53}{144}e[\mu(a_f v)|c|Db)D^d D_c e^f d f - \frac{43}{72}e[\mu(a_f v)|c|Db)D^d D_d e^f c f \\
& -\frac{53}{144}e[\mu(a_f v)|c|Db)D^d D_f e^c d f + \frac{43}{72}e[\mu(a_f v)|c|Db)D^d D_f e^d c f + \frac{5}{8}D[\mu D|c|e^d v]d D_c f(a b) \\
& +\frac{17}{48}D[\mu D|c e^d(a_d|D|c|f b)_v] - \frac{65}{48}D[\mu D|c e_d|(a_v)D|c|f b]d + \frac{9}{8}D[\mu D|c|e_v|(a_d|D|c|f b) d \\
& -\frac{13}{16}D[\mu D|c|e(a_v)d D|c|f b]d - \frac{15}{16}D[\mu D_v]e_c(a_d D|c|f b) d + \frac{47}{48}D[\mu D(a_e|c|v)d D|c|f b]d \\
& +\frac{1}{48}D[\mu D(a_e v)_c d D|c|f b]d + \frac{7}{12}e[\mu(aD_v)D_c e|d f_d D|c|f b]f - \frac{15}{16}D[\mu D|c|e_v]a b D_c f_d d + \\
& \frac{89}{48}D[\mu D|c|e(a b)_v]D_c f_d d + \frac{3}{4}D[\mu D_v]e_c a b D_c f_d d - \frac{3}{2}D[\mu D(a_e|c|b)_v]D_c f_d d + \frac{11}{16}D[\mu D|c e_d|a b D_c f_d v] \\
& -\frac{71}{48}D[\mu D|c e(a b)_d]D_c f_d v] + \frac{23}{24}D[\mu D(a_e|c b)_d]D_c f_d v] - \frac{1}{48}D[\mu D(a_e b)|c_d|D_c f_d v] + \\
& \frac{23}{36}\eta^{a b}D[\mu D|c e_d|v]f D_c f_d f - \frac{109}{144}\eta^{a b}D[\mu D|c|e_v]d f D_c f_d f + \frac{16}{27}\eta^{a b}D[\mu D_v]e_c d f D_c f_d f + \\
& \frac{5}{48}e[\mu(aD_v)D_c e_d b]f D_c f_d f - \frac{11}{12}e[\mu(aD_v)D_c e_b]d f D_c f_d f + \frac{13}{18}e[\mu(aD_v)Db)e^c d f D_c f_d f - \\
& \frac{49}{48}\eta^{a b}D[\mu D|c|e^d v]d D_c f_f f - \frac{7}{24}e[\mu(aD_v)D_c e|d|b]d D_c f_f f + \frac{31}{48}\eta^{a b}D[\mu D|c e^d f_d]D_c f_f v] \\
& +\frac{55}{144}\eta^{a b}D[\mu D|c e_d|v]f D_c f_f d + \frac{3}{16}e[\mu(aD_v)D_c e_d b]f D_c f_f d - \frac{3}{16}D[\mu D|c f^d_d|D_c e_v]a b \\
& +\frac{3}{16}D[\mu D|c f(a_d|D|c|e_v)b]d - \frac{1}{48}D[\mu D(a_f|c_d|D|c|e_v)b]d - \frac{11}{48}\eta^{a b}D[\mu D|c f_d f|D_c e_v]d f \\
& +\frac{17}{48}D[\mu D|c f^d_d|D_c e(a b)_v] - \frac{13}{24}D[\mu D|c|f v]d D_c e(a b)_d + \frac{3}{16}D[\mu D|c f(a_d|D|c|e_b)_d v] + \\
& \frac{1}{48}D[\mu D(a_f|c_d|D|c|e_b)_d v] - \frac{13}{48}e[\mu(aD_v)D_c f_d f D|c|e_b]d f + \frac{3}{8}D[\mu D_v]f(a b)D_c e^d c d - \\
& \frac{17}{48}D[\mu D(a_f b)_v]D_c e^d c d - \frac{3}{8}D[\mu D|c|f(a b)D_c e^d v]d + \frac{3}{16}D[\mu D|c|f v]d D_c e^d a b + \frac{17}{48}D[\mu D|c|f(a_v)D|c e_d|b]d \\
& -\frac{17}{48}D[\mu D|c f(a_d|D|c e_d|b)_v] - \frac{1}{24}e[\mu(aD_v)D_c f_d f D|c e_d|b]f + \frac{11}{144}\eta^{a b}D[\mu D|c f_d f|D_c e^d f v] - \\
& \frac{11}{144}\eta^{a b}D[\mu D|c f^d_d|D_c e^f v]f + \frac{1}{24}e[\mu(aD_v)D_c f^d_d D_c e^f|b]f + \frac{11}{48}\eta^{a b}D[\mu D|c|f v]d D_c e^f d f
\end{aligned}$$

$$\begin{aligned}
& -\frac{7}{108}\eta^{ab}D_{[\mu}D_{\nu]}f_{cd}D_{ce}f^ef^f + \frac{13}{48}e_{[\mu}(aD_{\nu]}D_{cd}f^b)_{d}D_{ce}f^ef^f - \frac{11}{144}e_{[\mu}(aD_{\nu]}D^b)f_{cd}D_{ce}f^ef^f \\
& -\frac{3}{16}D_{[\mu}e_{\nu]}^{ab}D_{cd}D_{ce}f^d{}_a + \frac{17}{48}D_{[\mu}e^{(ab)}_{\nu]}D_{cd}D_{ce}f^d{}_a + \frac{13}{8}D_{[\mu}f^{(ab)}D_{cd}|c|e^d{}_{\nu]}{}_a + \\
& \frac{1}{48}D_{[\mu}f^{(a}{}_{\nu]}D_{|cd}D_{ce}d|b)_{d}{}_a - \frac{7}{96}f^{(a}{}_{[\mu}D_{|cd}|c|D_{\nu]}e^d|b)_{d}{}_a + \frac{7}{96}f^{(a}{}_{[\mu}D_{|cd}|c|D^b)e^d{}_{\nu]}{}_a + \\
& \frac{7}{96}f^{(a}{}_{[\mu}D_{|cd}|c|D^d|e_{\nu]}b)_{d}{}_a - \frac{7}{96}f^{(a}{}_{[\mu}D_{|cd}|cdD^d|e^b)_{d}|_{\nu]}{}_a + \frac{7}{108}\eta^{ab}D_{[\mu}e_{cd}f_{\nu]}D_{cd}D_{\nu]}f^d{}_f - \\
& \frac{1}{16}D_{[\mu}f_{|cd}|D_{cd}D_{\nu]}e^{(ab)}{}_d + \frac{3}{8}D_{[\mu}f^{(ab)}D_{cd}D_{\nu]}e^d{}_c{}_d - \frac{1}{2}D_{[\mu}f_{|cd}|D_{cd}D_{\nu]}e^d{}_a{}_b + \frac{1}{2}D_{[\mu}f^{(a}{}_{|c|}D_{|cd}D_{\nu]}e^d|b)_{d}{}_a \\
& -\frac{17}{54}\eta^{ab}D_{[\mu}f_{|cd}|D_{cd}D_{\nu]}e^f{}_d{}_f - \frac{1}{6}f^{(a}{}_{[\mu}D_{|cd}D_{\nu]}D_{ce}d|b)_{d}{}_a + \frac{7}{96}f^{(a}{}_{[\mu}D_{|cd}|D_{\nu]}D^b)e^d{}_c{}_d + \\
& \frac{1}{6}f^{(a}{}_{[\mu}D_{|cd}D_{\nu]}D^d|e^c{}_b)_{d}{}_a - \frac{7}{96}f^{(a}{}_{[\mu}D_{|cd}D_{\nu]}D^d|e^b)_{c}{}_d - \frac{1}{48}D_{[\mu}e_{|c|}{}_{\nu]}{}_aD_{cd}(af^b)_{d}{}_a + \frac{1}{48}D_{[\mu}e_{\nu]}{}_c{}_dD_{cd}(af^b)_{d}{}_a \\
& + \frac{1}{24}D_{[\mu}f_{|cd}|D_{cd}(ae^{\nu}{}_b)_{d}{}_a + \frac{1}{48}D_{[\mu}f_{|cd}|D_{cd}(ae^b)_{d}{}_{\nu]}{}_a - D_{[\mu}f_{\nu]}{}_c{}_dD_{cd}(ae^d|b)_{d}{}_a + D_{[\mu}f_{|cd}|D_{cd}(ae^d|b)_{\nu]}{}_a \\
& + \frac{1}{48}D_{[\mu}e_{|c}{}^{(a}{}_d|D_{|cd}D^b)f^d{}_{\nu]}{}_a - \frac{1}{48}D_{[\mu}e^{(a}{}_{|cd}|D_{|cd}D^b)f^d{}_{\nu]}{}_a + \frac{11}{144}e_{[\mu}(aD_{\nu]}e_{cd}f_{\nu]}D_{|cd}D^b)f^d{}_f \\
& -\frac{1}{48}D_{[\mu}f^{(a}{}_{\nu]}D_{|cd}D^b)e^d{}_c{}_d - \frac{1}{2}D_{[\mu}f^{(a}{}_{|c|}D_{|cd}D^b)e^d{}_{\nu]}{}_a - \frac{7}{18}e_{[\mu}(aD_{\nu]}f_{cd}D_{|cd}D^b)e^f{}_d{}_f \\
& -\frac{1}{6}f^{(a}{}_{[\mu}D_{|cd}D^b)D_{|c|}e^d{}_{\nu]}{}_a - \frac{7}{96}f^{(a}{}_{[\mu}D_{|cd}D^b)D_{\nu]}e^d{}_c{}_d + \frac{1}{6}f^{(a}{}_{[\mu}D_{|cd}D^b)D^d|e^c{}_d|_{\nu]}{}_a + \\
& \frac{7}{96}f^{(a}{}_{[\mu}D_{|cd}D^b)D^d|e^c{}_d|_{\nu]}{}_a - \frac{1}{144}e_{[\mu}(aD_{\nu]}e_{cd}f_{\nu]}D_{|cd}D^d|f^b)_{\nu]}{}_f - \frac{1}{108}\eta^{ab}D_{[\mu}e_{cd}f_{\nu]}D_{cd}D^d|f^f{}_{\nu]}{}_a - \\
& 2D_{[\mu}f^{(ab)}D_{cd}D^d|e^c{}_d|_{\nu]}{}_a + \frac{1}{3}D_{[\mu}f^{(a}{}_{\nu]}D_{|cd}D^d|e^c{}_b)_{d}{}_a + \frac{1}{2}D_{[\mu}f_{|cd}|D_{cd}D^d|e^{\nu}{}_a{}_b - \frac{1}{2}D_{[\mu}f^{(a}{}_{|c|}D_{|cd}D^d|e^{\nu}{}_b)_{d}{}_a \\
& + D_{[\mu}f_{\nu]}{}_c{}_dD_{cd}D^d|e^{(ab)}{}_d - D_{[\mu}f_{|cd}|D_{cd}D^d|e^{(ab)}{}_{\nu]}{}_a - \frac{1}{3}D_{[\mu}f^{(a}{}_{\nu]}D_{|cd}D^d|e^b)_{c}{}_d + \frac{1}{2}D_{[\mu}f^{(a}{}_{|cd}D_{|cd}D^d|e^b)_{d}|_{\nu]}{}_a \\
& + \frac{2}{3}\eta^{ab}D_{[\mu}f_{|cd}|D_{cd}D^d|e^f{}_{\nu]}{}_f + \frac{1}{6}f^{(a}{}_{[\mu}D_{|cd}D^d|D_{|ce}d|b)_{\nu]}{}_a - \frac{2}{9}e_{[\mu}(af^b)_{\nu]}D_{cd}D^d|ce^f{}_d{}_f \\
& -\frac{1}{6}f^{(a}{}_{[\mu}D_{|cd}D^d|D_{|de}c|b)_{\nu]}{}_a - \frac{7}{96}f^{(a}{}_{[\mu}D_{|cd}D^d|D_{|d|e}{}_{\nu]}{}_b)_{c}{}_a + \frac{7}{96}f^{(a}{}_{[\mu}D_{|cd}D^d|D_{|de}^b)_{c|}{}_{\nu]}{}_a + \\
& \frac{2}{9}e_{[\mu}(af^b)_{\nu]}D_{cd}D^d|de^f{}_c{}_f + \frac{7}{96}f^{(a}{}_{[\mu}D_{|cd}D^d|D_{\nu]}e^d{}_c{}_a - \frac{7}{96}f^{(a}{}_{[\mu}D_{|cd}D^d|D^b)e^d|c|_{\nu]}{}_a + \\
& \frac{2}{9}e_{[\mu}(af^b)_{\nu]}D_{cd}D^d|fe^c{}_d{}_f - \frac{2}{9}e_{[\mu}(af^b)_{\nu]}D_{cd}D^d|fe^d{}_c{}_f + \frac{1}{108}\eta^{ab}D_{[\mu}e_{|c|}{}_{\nu]}{}_aD_{cd}D^d|ff^f{}_d - \\
& \frac{1}{108}\eta^{ab}D_{[\mu}e_{\nu]}{}_c{}_dD_{cd}D^d|ff^f{}_f{}_d + \frac{1}{144}e_{[\mu}(aD_{\nu]}e^b)_{cd}D_{cd}D^d|ff^f{}_f{}_d - \frac{1}{144}e_{[\mu}(aD_{\nu]}e^b)_{cd}D_{cd}D^d|ff^f{}_f{}_d - \\
& \frac{1}{144}e_{[\mu}(aD_{\nu]}f_{cd}D_{|cd}D^f|e^f{}_b)_{d}{}_a - \frac{1}{108}\eta^{ab}D_{[\mu}f_{|cd}D_{cd}D^f|e^f|_{\nu]}{}_d + \frac{7}{27}\eta^{ab}D_{[\mu}f_{|cd}|D_{cd}D^f|e^{\nu}{}_f{}_f{}_d \\
& + \frac{23}{72}e_{[\mu}(aD_{\nu]}f_{cd}D_{|cd}D^f|e^b)_{\nu]}{}_f{}_d - \frac{2}{3}\eta^{ab}D_{[\mu}f_{|cd}D_{cd}D^f|e^d{}_f|_{\nu]}{}_a + \frac{23}{48}D_{[\mu}D_{\nu]}e^{(ab)}{}_c{}_dD^d|f^d{}_a{}_c - \\
& \frac{11}{16}D_{[\mu}D_{\nu]}e^{cab}D^d|f^d{}_a{}_c - \frac{7}{48}D_{[\mu}D^b(ae^{\nu}{}_b)_{cd}D^d|f^d{}_a{}_c - \frac{1}{6}D_{[\mu}D^b(ae^b)_{c\nu]}D^d|f^d{}_a{}_c + \frac{65}{48}D_{[\mu}D^b(ae^b)_{|c|}{}_{\nu]}D^d|f^d{}_a{}_c \\
& + \frac{1}{2}D_{[\mu}D^ce^{\nu}{}_b]^{ab}D^d|f^d{}_a{}_c - D_{[\mu}D^ce^{(ab)}{}_{\nu]}D^d|f^d{}_a{}_c - \frac{5}{6}D_{[\mu}D^b(ae^b)_{|c|}{}_{\nu]}D_{cd}D^d|f^d|_{\nu]}{}_a + \frac{1}{2}D_{[\mu}D^ce^{(ab)}{}_{|c|}{}_{\nu]}D_{cd}D^d|f^d|_{\nu]}{}_a - \\
& D_{[\mu}D^ce^d|c|_{\nu]}D^d|f^{(ab)}{}_a + \frac{7}{48}D_{[\mu}D_{\nu]}e^c(a^c{}_d|d|f^b)_{d}{}_a - \frac{7}{48}D_{[\mu}D^b(ae^b)_{c\nu]}D_{cd}D^d|f^b)_{d}{}_a - \frac{1}{2}D_{[\mu}D^ce^{\nu}{}_b(a^c{}_d|d|f^b)_{d}{}_a \\
& + \frac{1}{2}D_{[\mu}D^ce^{(a}{}_{|c|}{}_{\nu]}D_{|d|}f^b)_{d}{}_a + D_{[\mu}D_{|ce}d|_{\nu]}(a^{\nu}{}_d|d|f^b)_{c}{}_a - \frac{5}{16}e_{[\mu}(aD_{\nu]}D_{|ce}d^c{}_fD^d|f^b)_{\nu]}{}_f \\
& -\frac{1}{2}D_{[\mu}D_{|ce}d|_{\nu]}^{ab}D^d|f^c{}_a{}_c - \frac{5}{6}\eta^{ab}D_{[\mu}D_{|ce}d|_{\nu]}{}_fD^d|f^c{}_f{}_f + \frac{5}{18}\eta^{ab}D_{[\mu}D_{|c|}{}_{\nu]}{}_aD^d|f^d{}_f{}_f -
\end{aligned}$$

$$\begin{aligned}
& \frac{5}{18} \eta^{ab} D_{[\mu} D_{\nu]} e_c d f D d f c f - \frac{1}{3} e_{[\mu} (a D_{\nu]} D_c e d b) f D d f c f + \frac{1}{3} e_{[\mu} (a D_{\nu]} D_c e b) d f D d f c f - \\
& \frac{1}{3} e_{[\mu} (a D_{\nu]} D b) e_c d f D d f c f + \frac{23}{108} \eta^{ab} D_{[\mu} D_{\nu]} e^c d c D d f f f + \frac{17}{18} \eta^{ab} D_{[\mu} D^c e | d c | \nu] D d f f f - \\
& \frac{5}{18} \eta^{ab} D_{[\mu} D^c e \nu] c d D d f f f + \frac{37}{144} e_{[\mu} (a D_{\nu]} D b) e^c d c D d f f f + \frac{1}{3} e_{[\mu} (a D_{\nu]} D | c | e d b) c D d f f f \\
& - \frac{1}{3} e_{[\mu} (a D_{\nu]} D | c | e b) c d D d f f f - \frac{5}{12} \eta^{ab} D_{[\mu} D^c e | d c f | D d f f \nu] - \frac{1}{9} \eta^{ab} D_{[\mu} D | c e d | \nu] f D d f f c \\
& + \frac{7}{108} \eta^{ab} D_{[\mu} D_{\nu]} e_c d f D d f f c + \frac{11}{144} e_{[\mu} (a D_{\nu]} D b) e_c d f D d f f c + \frac{1}{3} D_{[\mu} D (a f b) c D d e | c d | \nu] - \\
& D_{[\mu} D c f (a b) D d e | c d | \nu] + \frac{17}{48} D_{[\mu} D_{\nu]} f (a | c D d | e c b) d - \frac{17}{48} D_{[\mu} D (a f | c \nu] D d | e c b) d - \frac{3}{16} D_{[\mu} D (a f b) c D d e | d | \nu] c + \\
& \frac{3}{16} D_{[\mu} D_{\nu]} f c c D d e d a b - \frac{3}{16} D_{[\mu} D_{\nu]} f (a | c D d | e d b) c + \frac{13}{24} D_{[\mu} D (a f | c \nu] D d | e d b) c - \frac{17}{48} D_{[\mu} D (a f | c | c D d | e d | b) \nu] \\
& - \frac{7}{48} D_{[\mu} D (a f b) c D d e \nu] d c + \frac{41}{48} D_{[\mu} D (a f | c | c | D d | e \nu] b) d - \frac{1}{2} D_{[\mu} D c f (a | c | D d | e \nu] b) d - \\
& \frac{41}{48} D_{[\mu} D_{\nu]} f c c D d e (a b) d + \frac{1}{2} D_{[\mu} D c f | c | \nu] D d e (a b) d - \frac{3}{16} D_{[\mu} D_{\nu]} f (a | c D d | e b) d c + \frac{1}{2} D_{[\mu} D (a f | c \nu] D d | e b) d c \\
& - \frac{5}{6} D_{[\mu} D (a f | c | c D d | e b) d | \nu] + \frac{1}{2} D_{[\mu} D c f (a | c D d | e b) d | \nu] - \frac{5}{144} \eta^{ab} D_{[\mu} D_{\nu]} f c c D d e f d f + \\
& \frac{11}{36} \eta^{ab} D_{[\mu} D c f | c | \nu] D d e f d f - \frac{1}{24} e_{[\mu} (a D_{\nu]} D b) f c c D d e f d f + \frac{11}{48} e_{[\mu} (a D_{\nu]} D | c | f b) c D d e f d f - \\
& D_{[\mu} f c \nu] D d D_c e d a b + \frac{3}{2} D_{[\mu} f (a | c D d | D | c e d | b) \nu] - \frac{1}{4} \eta^{ab} D_{[\mu} f c \nu] D d D_c e f d f - \frac{5}{48} e_{[\mu} (a D_{\nu]} f b) c D d D_c e f d f \\
& + \frac{1}{6} \eta^{ab} f_{[\mu} c D d D | c D d | e f \nu] f + \frac{1}{6} e_{[\mu} (a f \nu] | c D d D_c D d e f | b) f + \frac{13}{96} \eta^{ab} f_{[\mu} c D d D | c | D \nu] e f d f \\
& + \frac{5}{32} e_{[\mu} (a f \nu] | c D d | D_c D b) e f d f - \frac{1}{6} \eta^{ab} f_{[\mu} c D d D | c D f e d f | \nu] - \frac{1}{6} e_{[\mu} (a f \nu] | c D d D_c D f | e d b) f \\
& - \frac{13}{96} \eta^{ab} f_{[\mu} c D d D | c | D f e \nu] d f - \frac{5}{32} e_{[\mu} (a f \nu] | c D d D_c D f | e b) d f - \frac{13}{24} D_{[\mu} e (a b) c D d D | d | f \nu] c + \\
& \frac{3}{16} D_{[\mu} e c a b D d D | d | f \nu] c - \frac{3}{8} D_{[\mu} e c \nu] c D d D d f (a b) + \frac{3}{16} D_{[\mu} e \nu] (a | c D d | D d f b) c + \frac{3}{16} D_{[\mu} e (a | c \nu] D d | D d f b) c \\
& - \frac{17}{48} D_{[\mu} e c (a \nu] D | d | D d f b) c + \frac{17}{48} D_{[\mu} e c (a | c D d | d | D d | f b) \nu] - \frac{11}{144} \eta^{ab} D_{[\mu} e c \nu] c D d D d f f f \\
& + \frac{1}{24} e_{[\mu} (a D_{\nu]} e | c | b) c D d D d f f f + \frac{19}{16} D_{[\mu} f c \nu] D d D d e c a b - \frac{89}{48} D_{[\mu} f (a | c D d | D | d e c | b) \nu] - \\
& \frac{19}{16} D_{[\mu} f c | c D d d | e \nu] a b + \frac{9}{8} D_{[\mu} f (a | c D d | D | d | e \nu] b) c - \frac{95}{48} D_{[\mu} f c \nu] D d D d e (a b) c + \frac{113}{48} D_{[\mu} f c | c D d d | e (a b) \nu] \\
& - \frac{13}{16} D_{[\mu} f (a | c D d | D | d | e b) \nu] c + \frac{173}{144} \eta^{ab} D_{[\mu} f c \nu] D d D d e f c f + \frac{11}{12} e_{[\mu} (a D_{\nu]} f b) c D d D d e f c f - \\
& \frac{235}{144} \eta^{ab} D_{[\mu} f c | c D d d | e f \nu] f - \frac{5}{8} e_{[\mu} (a D_{\nu]} f | c c D d D d e f | b) f - \frac{13}{96} \eta^{ab} f_{[\mu} c D d D | d D c | e f \nu] f - \\
& \frac{5}{32} e_{[\mu} (a f \nu] | c D d D d c e f | b) f + \frac{13}{96} \eta^{ab} f_{[\mu} c D d D | d | D \nu] e f c f + \frac{5}{32} e_{[\mu} (a f \nu] | c D d | D d D b) e f c f \\
& + \frac{13}{96} \eta^{ab} f_{[\mu} c D d D | d D f e c f | \nu] + \frac{5}{32} e_{[\mu} (a f \nu] | c D d D d f | e c b) f - \frac{13}{96} \eta^{ab} f_{[\mu} c D d D | d | D f e \nu] c f \\
& - \frac{5}{32} e_{[\mu} (a f \nu] | c D d D d f | e b) c f + \frac{5}{24} D_{[\mu} e (a b) c D d D \nu] f d c - \frac{3}{16} D_{[\mu} e c a b D d D \nu] f d c - \\
& \frac{1}{48} D_{[\mu} e c (a | c | D d | D \nu] f b) d - \frac{7}{108} \eta^{ab} D_{[\mu} e c | d c | D d D \nu] f f f + \frac{7}{108} \eta^{ab} D_{[\mu} e | c d f | D d D \nu] f f c + \\
& \frac{1}{48} D_{[\mu} f (a | c D d | D \nu] e c b) d + \frac{19}{16} D_{[\mu} f c | c | D d D \nu] e d a b - \frac{9}{8} D_{[\mu} f (a | c D d | D \nu] e d b) c - \frac{1}{48} D_{[\mu} f c | c | D d D \nu] e (a b) d
\end{aligned}$$

$$\begin{aligned}
& -\frac{3}{16}D[\mu f(a|cDd|Dv)e^b]_d c + \frac{25}{48}\eta^{ab}D[\mu f^c|c|DdDv]e^f d f - \frac{13}{96}\eta^{ab}f[\mu^cDdDv]Dce^f d f \\
& + \frac{1}{6}\eta^{ab}f[\mu^cDdDv]Dde^f c f + \frac{13}{96}\eta^{ab}f[\mu^cDdDv]Dfe^c d f - \frac{1}{6}\eta^{ab}f[\mu^cDdDv]Dfe^d c f + \\
& \frac{1}{48}D[\mu e^c v]_c Dd(a f b)_d - \frac{1}{48}D[\mu f^c v]_D d(a e c b)_d + \frac{79}{48}D[\mu f^c v]_D d(a e d b)_c - \frac{113}{48}D[\mu f^c|c|DdD(a e d|b)_v] \\
& + \frac{1}{48}D[\mu f^c|c|DdD(a e v)_b]_d + \frac{1}{6}D[\mu f^c v]_D d(a e b)_d c - \frac{5}{24}D[\mu e v]_D(a|cDd|D b)f d c - \frac{1}{6}D[\mu e(a|c v)_D d|D b)f d c \\
& + \frac{17}{48}D[\mu e^c(a v)_D d|D b)f d c] - \frac{11}{144}e[\mu(a D v)]e|c d c D d|D b)f f f + \frac{11}{144}e[\mu(a D v)]e c d f D d|D b)f f c \\
& + \frac{55}{48}D[\mu f(a|cDd|D b)e|d|v]_c + \frac{3}{16}D[\mu f(a|cDd|D b)e v]_d c + \frac{5}{8}e[\mu(a D v)]f|c c D d|D b)e^f d f - \\
& \frac{5}{32}e[\mu(a f v)]|c D d|D b)Dce^f d f + \frac{1}{6}e[\mu(a f v)]|c D d|D b)Dde^f c f + \frac{5}{32}e[\mu(a f v)]|c D d|D b)Dfe^c d f - \\
& \frac{1}{6}e[\mu(a f v)]|c D d|D b)Dfe^d c f + \frac{1}{144}e[\mu(a D v)]e c d f D d|D c|f b)f + \frac{1}{108}\eta^{ab}D[\mu e|c d f|D dD c f f v] \\
& - \frac{7}{36}\eta^{ab}D[\mu e^c v]_c DdD f f d f - \frac{11}{48}e[\mu(a D v)]e|c|b)_c DdD f f d f + \frac{3}{4}\eta^{ab}D[\mu f^c v]_D dD f e^c d f + \\
& \frac{9}{16}e[\mu(a D v)]f b)_c DdD f e^c d f - \frac{133}{108}\eta^{ab}D[\mu f^c v]_D dD f e^d f c - \frac{127}{144}e[\mu(a D v)]f b)_c DdD f e^d f c \\
& + \frac{67}{36}\eta^{ab}D[\mu f^c|c|DdD f e^d f|v] + \frac{43}{48}e[\mu(a D v)]f|c c D dD f|e d b)_f - \frac{13}{54}\eta^{ab}D[\mu f^c v]_D dD f e^f d c \\
& - \frac{2}{9}e[\mu(a D v)]f b)_c DdD f e^f d c - \frac{3}{4}\eta^{ab}D[\mu f^c|c|DdD f e v]_d f - \frac{43}{48}e[\mu(a D v)]f|c c D dD f|e b)_d f + \\
& \frac{13}{96}\eta^{ab}f[\mu^cDdD f D|c e f d|v] + \frac{5}{32}e[\mu(a f v)]|c D dD f|D c e f b)_d - \frac{1}{6}\eta^{ab}f[\mu^cDdD f D|d e f c|v] - \\
& \frac{1}{6}e[\mu(a f v)]|c D dD f|D d e f b)_c - \frac{13}{96}\eta^{ab}f[\mu^cDdD f D|f e c d|v] - \frac{5}{32}e[\mu(a f v)]|c D dD f|D f e c b)_d \\
& + \frac{1}{6}\eta^{ab}f[\mu^cDdD f D|f e d c|v] + \frac{1}{6}e[\mu(a f v)]|c D dD f|D f e d b)_c + \frac{13}{96}\eta^{ab}f[\mu^cDdD f D|f|e v]_c d + \\
& \frac{5}{32}e[\mu(a f v)]|c D dD f|D f e b)_c d - \frac{13}{96}\eta^{ab}f[\mu^cDdD f D v]e^f c d - \frac{5}{32}e[\mu(a f v)]|c D dD f|D b)e^f c d \\
& + \frac{1}{9}\eta^{ab}D[\mu D c e^d v]_d D f f f c - \frac{11}{24}e[\mu(a D v)]D|c e d|b)_d D f f f c - \frac{23}{48}\eta^{ab}D[\mu D v]e^c d c D f f f d + \\
& \frac{7}{36}\eta^{ab}D[\mu D c e|c|d v]_D f f f d + \frac{4}{9}\eta^{ab}D[\mu D c e v]_c d D f f f d - \frac{29}{36}\eta^{ab}D[\mu D c e^d|c|v]_D f f f d - \\
& \frac{7}{12}e[\mu(a D v)]D b)e^c d c D f f f d + \frac{11}{48}e[\mu(a D v)]D|c|e c b)_d D f f f d + \frac{13}{24}e[\mu(a D v)]D|c|e b)_c d D f f f d \\
& - \frac{11}{48}e[\mu(a D v)]D|c e d|b)_c D f f f d + \frac{11}{36}\eta^{ab}D[\mu D c e^d|c d D f f|v] + \frac{11}{48}e[\mu(a D v)]D|c e^d c d D f|f b)_f \\
& - \frac{1}{9}\eta^{ab}D[\mu D|c e d|v]_f D f f c d + \frac{1}{9}\eta^{ab}D[\mu D|c e d|v]_f D f f d c + \frac{13}{36}\eta^{ab}D[\mu D v]f^c d D f e^c f d - \\
& \frac{11}{12}\eta^{ab}D[\mu D c f^d v]_D f e^c c f d + \frac{11}{48}e[\mu(a D v)]D b)f^c d D f e^c c f d - \frac{37}{48}e[\mu(a D v)]D|c|f b)_d D f e^c c f d \\
& + \frac{5}{4}\eta^{ab}D[\mu D c f^d|d D f e^c c f|v] + \frac{9}{16}e[\mu(a D v)]D|c f^d d D f|e c b)_f - \frac{23}{144}\eta^{ab}D[\mu D v]f^c d D f e^d f c \\
& + \frac{7}{18}\eta^{ab}D[\mu D c f^d v]_D f e^d f c - \frac{3}{16}e[\mu(a D v)]D b)f^c d D f e^d f c + \frac{11}{24}e[\mu(a D v)]D|c|f b)_d D f e^d f c \\
& - \frac{29}{36}\eta^{ab}D[\mu D c f|c d D f e^d f|v] - \frac{11}{48}e[\mu(a D v)]D|c f c^d D f|e d b)_f + \frac{11}{48}\eta^{ab}D[\mu D v]f^c d D f e^f c d \\
& - \frac{1}{2}\eta^{ab}D[\mu D c f^d v]_D f e^f c d + \frac{13}{48}e[\mu(a D v)]D b)f^c d D f e^f c d - \frac{11}{24}e[\mu(a D v)]D|c|f b)_d D f e^f c d
\end{aligned}$$

$$\begin{aligned}
& \frac{11}{36} \eta^a b D_{[\mu} D^c f^d | d D^f e f | v] c + \frac{7}{36} \eta^a b D_{[\mu} D^c f | c^d D^f e f | v] d + \frac{11}{48} e_{[\mu} (a D_v] D | c f^d d D^f | e f^b) c + \\
& \frac{11}{48} e_{[\mu} (a D_v] D | c f c^d D^f | e f^b) d - \frac{2}{3} \eta^a b D_{[\mu} D^c f^d | d | D^f e v] f c + \frac{4}{9} \eta^a b D_{[\mu} D^c f | c | d D^f e v] f d - \\
& \frac{19}{24} e_{[\mu} (a D_v] D | c f^d d D^f | e b) f c + \frac{13}{24} e_{[\mu} (a D_v] D | c f c^d D^f | e b) f d + \frac{7}{27} \eta^a b D_{[\mu} e v] c^d D^f D c f f d \\
& + \frac{13}{54} \eta^a b D_{[\mu} e c^d v] D^f D c f f d + \frac{17}{72} e_{[\mu} (a D_v] e b) c^d D^f D c f f d + \frac{2}{9} e_{[\mu} (a D_v] e | c | b) d D^f D c f f d - \\
& \frac{1}{9} \eta^a b D_{[\mu} f c^d D^f D | c e d f | v] - \frac{113}{108} \eta^a b D_{[\mu} f c^d D^f D | c e f | v] d - \frac{47}{144} e_{[\mu} (a D_v] f | c^d D^f | D c e f^b) d + \\
& \frac{23}{108} \eta^a b D_{[\mu} f c^d D^f D | c | e v] f d + \frac{47}{144} e_{[\mu} (a D_v] f | c^d D^f | D c e b) f d - \frac{11}{36} \eta^a b D_{[\mu} e c^d v] D^f D d f f c \\
& - \frac{11}{48} e_{[\mu} (a D_v] e | c | b) d D^f D d f f c + \frac{1}{9} \eta^a b D_{[\mu} f c^d D^f D | d e c f | v] - \frac{1}{9} \eta^a b D_{[\mu} f c^d D^f D | d e f | v] c \\
& - \frac{11}{48} \eta^a b D_{[\mu} e v] c^d D^f D f f c d + \frac{11}{144} \eta^a b D_{[\mu} e c^d v] D^f D f f c d - \frac{13}{48} e_{[\mu} (a D_v] e b) c^d D^f D f f c d - \\
& \frac{1}{24} e_{[\mu} (a D_v] e | c | b) d D^f D f f c d + \frac{11}{48} \eta^a b D_{[\mu} e c^d | c D^f D f | f v] d + \frac{13}{48} e_{[\mu} (a D_v] e | c^d c D^f | D f f^b) d + \\
& \frac{29}{36} \eta^a b D_{[\mu} f c^d D^f D | f e c | v] d + \frac{5}{48} e_{[\mu} (a D_v] f | c^d D^f | D f e c^b) d + \frac{55}{144} \eta^a b D_{[\mu} f c^d D^f D | f e d | v] c + \\
& \frac{3}{16} e_{[\mu} (a D_v] f | c^d D^f | D f e d^b) c - \frac{109}{144} \eta^a b D_{[\mu} f c^d D^f D | f | e v] c d - \frac{11}{12} e_{[\mu} (a D_v] f | c^d D^f | D f e b) c d \\
& - \frac{11}{48} \eta^a b D_{[\mu} e c^d | c | D^f D v] f f d - \frac{1}{12} \eta^a b D_{[\mu} f c^d D^f D v] e c f d - \frac{23}{144} \eta^a b D_{[\mu} f c^d D^f D v] e d f c + \\
& \frac{109}{144} \eta^a b D_{[\mu} f c^d D^f D v] e f c d - \frac{13}{48} e_{[\mu} (a D_v] e | c^d c D^f | D b) f f d - \frac{5}{48} e_{[\mu} (a D_v] f | c^d D^f | D b) e c f d \\
& - \frac{3}{16} e_{[\mu} (a D_v] f | c^d D^f | D b) e d f c + \frac{11}{12} e_{[\mu} (a D_v] f | c^d D^f | D b) e f c d - \frac{3}{16} \eta^a b f_{[\mu} c e v] d^f D c f d f \\
& - \frac{7}{16} e_{[\mu} (a f v] | c | e b) d^f D c f d f + \frac{5}{12} \eta^a b f_{[\mu} c e d v] f D c f d f + \frac{5}{24} e_{[\mu} (a f v] | c e d | b) f D c f d f - \\
& \frac{17}{24} f_{[\mu} c e (a b) d D | c f d | v] - \frac{1}{24} f_{[\mu} (a e b) c^d D | c f d | v] + \frac{1}{3} f_{[\mu} (a e | c | b) d D | c f d | v] + \frac{1}{48} f_{[\mu} c e d a b D | c f d | v] + \\
& \frac{3}{16} \eta^a b f_{[\mu} c e d | d^f D c f f | v] - \frac{1}{24} f_{[\mu} c e d v] d D c f (a b) + \frac{1}{48} f_{[\mu} c e v] (a | d | D c f b) d + \frac{1}{24} f_{[\mu} (a e v] | c d | D c f b) d + \\
& \frac{1}{48} f_{[\mu} c e (a v] | d | D c f b) d - \frac{1}{3} f_{[\mu} (a e | c v] d | D c f b) d - \frac{11}{16} f_{[\mu} c e d (a v] D c f b) d + \frac{7}{16} e_{[\mu} (a f v] | c e d^f | D c f b) f \\
& + \frac{11}{16} f_{[\mu} c e d (a | d c | f b) v] - \frac{1}{48} f_{[\mu} c e v] a b D c f^d d - \frac{3}{16} f_{[\mu} (a e v] b) c D c f^d d + \frac{11}{16} f_{[\mu} c e (a b) v] D c f^d d \\
& - \frac{23}{48} f_{[\mu} (a e b) v] c D c f^d d - \frac{5}{12} \eta^a b f_{[\mu} c e d v] d D c f f f - \frac{5}{24} e_{[\mu} (a f v] | c e d | b) d D c f f f - \\
& \frac{7}{144} \eta^a b f_{[\mu} c f^d f D | c e d f | v] + \frac{1}{48} f_{[\mu} c f v] d D c e d a b + \frac{1}{48} e_{[\mu} (a f v] | c f d f | D c e d b) f - f_{[\mu} d f (a | c | D | c e d | b) v] \\
& + \frac{67}{144} \eta^a b f_{[\mu} c f^d f D | c e f d | v] + \frac{3}{16} e_{[\mu} (a f v] | c f d f | D c e f b) d - \frac{3}{8} \eta^a b f_{[\mu} c f^d f D | c | e v] d f - \\
& \frac{1}{48} f_{[\mu} c f^d | d D c | e v] a b + \frac{7}{48} f_{[\mu} (a f | c d | D | c | e v) b) d - \frac{31}{48} f_{[\mu} c f v] d D c e (a b) d + \frac{11}{16} f_{[\mu} c f^d | d D c | e (a b) v] \\
& - \frac{1}{2} e_{[\mu} (a f v] | c f d f | D c e b) d f + \frac{25}{48} f_{[\mu} (a f | c d | D | c e b) d | v] + \frac{47}{24} f_{[\mu} c f (a b) D | c | e d v] d - \\
& \frac{3}{16} f_{[\mu} (a | c | f b) | \mu D | c | e d v] d - \frac{3}{16} f_{[\mu} (a f b) c D | c | e d v] d - \frac{5}{6} f_{[\mu} c f (a v] D c e | d | b) d + \frac{37}{48} \eta^a b f_{[\mu} c f v] d D c e f d f \\
& + \frac{31}{48} e_{[\mu} (a f v] | d | f b) c D c e f d f + \frac{2}{9} e_{[\mu} (a f b) v] f c^d D c e f d f - \frac{17}{12} \eta^a b f_{[\mu} c f^d | d D c | e f v] f
\end{aligned}$$

$$\begin{aligned}
& -\frac{29}{24}e_{[\mu}(a f v) | c f d d D c e f | b) f + \frac{5}{24}\eta^{ab} f_{[\mu} c e v) d f D d f c f + \frac{7}{24}e_{[\mu}(a f v) | c | e b) d f D d f c f \\
& + \frac{1}{3}\eta^{ab} f_{[\mu} c e d v) f D d f c f + \frac{1}{3}e_{[\mu}(a f v) | c e d | b) f D d f c f + \frac{3}{16}f(a_{[\mu} e | c | b) d D | d f c | v) \\
& - \frac{5}{24}\eta^{ab} f_{[\mu} c e | c d f D d f f | v) - \frac{1}{3}\eta^{ab} f_{[\mu} c e d | c f D d f f | v) + \frac{23}{48}f(a_{[\mu} e | c v) d | D d f b) c - \\
& \frac{7}{24}e_{[\mu}(a f v) | c e c d f | D d f b) f - \frac{1}{3}e_{[\mu}(a f v) | c e d c f | D d f b) f + \frac{29}{48}\eta^{ab} f_{[\mu} c e | c | v) d D d f f f + \\
& \frac{31}{48}e_{[\mu}(a f v) | c | e c b) d D d f f f + \frac{1}{16}\eta^{ab} f_{[\mu} c e v) c d D d f f f + \frac{1}{48}e_{[\mu}(a f v) | c | e b) c d D d f f f \\
& - \frac{19}{48}\eta^{ab} f_{[\mu} c f d f D | d e c f | v) - \frac{1}{48}f_{[\mu} c f v) d D d e c a b - \frac{17}{48}e_{[\mu}(a f v) | c f d f | D d e c b) f + \\
& \frac{5}{16}f_{[\mu} d f (a | c | D | d e c | b) v) - \frac{13}{48}\eta^{ab} f_{[\mu} c f d f D | d | e v) c f - \frac{1}{24}f_{[\mu} d f (a | c | D | d | e v) b) c + \\
& \frac{31}{48}f_{[\mu} c f v) d D d e (a b) c + f c d f c_{[\mu} D | d | e (a b) v) - \frac{5}{16}e_{[\mu}(a f v) | c f d f | D d e b) c f - \frac{47}{48}f_{[\mu} d f (a | c | D | d e b) c | v) \\
& - \frac{37}{48}\eta^{ab} f_{[\mu} c f v) d D d e f c f + \frac{1}{2}e_{[\mu}(a f v) | d | f b) c D d e f c f + \frac{1}{9}e_{[\mu}(a f b) v) f c d D d e f c f + \\
& \frac{1}{16}\eta^{ab} f_{[\mu} | c f c d D d | e f v) f + \frac{1}{48}e_{[\mu}(a f v) c f | c d D d e f | b) f - \frac{29}{48}\eta^{ab} f_{[\mu} c e d v) f D f f c d - \\
& \frac{31}{48}e_{[\mu}(a f v) | c e d | b) f D f f c d - \frac{1}{16}\eta^{ab} f_{[\mu} c e d | c f D f f d | v) - \frac{1}{48}e_{[\mu}(a f v) | c e d c f | D f f b) d + \\
& f c d e d a b D_{[\mu} f | c | v) - 2f c d e (a b) d D_{[\mu} f | c | v) + \eta^{ab} f c d e f d f D_{[\mu} f | c | v) - \frac{2}{3}f(a | c | e c b) d D_{[\mu} f | d | v) \\
& + 2f c c e (a b) d D_{[\mu} f | d | v) + \frac{2}{3}f(a | c | e b) c d D_{[\mu} f | d | v) - 2f(a b) e c c d D_{[\mu} f | d | v) - 2f c c e d a b D_{[\mu} f | d | v) \\
& + 2f(a | c e d | b) c D_{[\mu} f | d | v) - \frac{1}{3}\eta^{ab} f c d e f c f D_{[\mu} f | d | v) - \frac{1}{3}\eta^{ab} f c c e d d f D_{[\mu} f | f | v) - \\
& \frac{2}{3}\eta^{ab} f c d e f c d D_{[\mu} f | f | v) + \frac{2}{3}f(a | c | f b) d D_{[\mu} e | c d | v) + \frac{2}{3}f(a | c | f b) d D_{[\mu} e | d c | v) - 2f(a b) f c d D_{[\mu} e | d c | v) \\
& - \frac{1}{3}\eta^{ab} f c d f c f D_{[\mu} e | d f | v) - \frac{1}{3}\eta^{ab} f c d f c f D_{[\mu} e | f d | v) + \eta^{ab} f c c f d f D_{[\mu} e | f d | v) + \\
& \frac{2}{3}f(a | c | f b) d D_{[\mu} e v) c d + \frac{2}{3}\eta^{ab} f c c f d f D_{[\mu} e v) d f - \frac{1}{3}\eta^{ab} f c d f c f D_{[\mu} e v) f d + f c c f d d D_{[\mu} e v) a b - \\
& 2f(a | c f d | d D_{[\mu} e v) b) c + \frac{2}{3}f c d f (a | c | D_{[\mu} e v) b) d - 2f(a | c f d | d D_{[\mu} e b) | c | v) + \frac{4}{3}f c d f (a | c | D_{[\mu} e b) | d | v) \\
& - 2f(a | c | f b) c D_{[\mu} e d v) d + 4f(a b) f c c D_{[\mu} e d v) d + \frac{1}{3}\eta^{ab} f c d f c d D_{[\mu} e f v) f - \frac{2}{3}\eta^{ab} f c c f d d D_{[\mu} e f v) f \\
& - \frac{2}{3}f(a | c | e [\mu^b) d D v) f c d + \frac{49}{24}f_{[\mu} c e (a b) d D v) f c d - \frac{4}{3}f(a | c | e b) [\mu^d D v) f c d - \frac{5}{48}f(a_{[\mu} e b) c d D v) f c d \\
& + 2f(a b) e c [\mu^d D v) f c d - \frac{7}{24}f(a_{[\mu} e | c | b) d D v) f c d - \frac{49}{48}f_{[\mu} c e d a b D v) f c d - \frac{2}{3}\eta^{ab} f c d e f_{[\mu} | f | D v) f c d \\
& + \frac{2}{3}\eta^{ab} f c d e d [\mu^f D v) f c f + \frac{2}{3}\eta^{ab} f c d e_{[\mu} | d | f D v) f c f - \frac{41}{48}\eta^{ab} f_{[\mu} c e d | d | f D v) f c f \\
& + \frac{1}{3}\eta^{ab} f c d e f d [\mu D v) f c f + \frac{41}{48}\eta^{ab} f_{[\mu} c e | c | d f D v) f d f - \frac{2}{3}\eta^{ab} f c c e_{[\mu} d f D v) f d f + \\
& \frac{1}{4}\eta^{ab} f_{[\mu} c e d | c | f D v) f d f - \eta^{ab} f c c e d_{[\mu} f D v) f d f + \frac{1}{3}\eta^{ab} f c d e f c_{[\mu} D v) f d f + 2f c d e d c_{[\mu} D v) f (a b) \\
& + \frac{49}{24}f_{[\mu} c e d | c d | D v) f (a b) - 4f c c e d_{[\mu} | d | D v) f (a b) - \frac{2}{3}f c d e_{[\mu} (a | d | D v) f b) c - \frac{4}{3}f c d e (a d_{[\mu} D v) f b) c + \\
& 2f(a | c e d |_{[\mu} | d | D v) f b) c - \frac{1}{48}f_{[\mu} c e d (a | d | D v) f b) c - \frac{2}{3}f(a | c e c_{[\mu} d | D v) f b) d - \frac{97}{48}f_{[\mu} c e | c | (a | d | D v) f b) d
\end{aligned}$$

$$\begin{aligned}
& -\frac{2}{3}f(a|c|e[\mu|c|d|D_v]f|b)_d + 2f(c|c|e[\mu(a|d|D_v]f|b)_d - \frac{11}{16}f[\mu|c|e(a|c|d|D_v]f|b)_d + 2f(c|c|e(a[\mu|d|D_v]f|b)_d \\
& + \frac{5}{48}f(a[\mu|e|c|c|d|D_v]f|b)_d - \frac{2}{3}f(a|c|e|c|[\mu D_v]f|b)_d + \frac{11}{16}f[\mu|c|e|d(a|c|D_v]f|b)_d + \frac{97}{48}f[\mu|c|e|c|a|b|D_v]f|d)_d \\
& - 2f(c|c|e[\mu(a|b|D_v]f|d)_d + 2f(a|c|e[\mu|b|c|D_v]f|d)_d - \frac{97}{48}f[\mu|c|e(a|b|c|D_v]f|d)_d + 2f(a|c|e|b|c|[\mu D_v]f|d)_d - \\
& 4f(a|b|e|c|[\mu|c|D_v]f|d)_d + \frac{7}{24}f(a[\mu|e|c|b|c|D_v]f|d)_d - \eta(a|b|f|c|d|e|c|[\mu D_v]f|f)_d - \frac{2}{3}\eta(a|b|f|c|d|e[\mu|c|d|D_v]f|f)_d \\
& + \frac{1}{12}\eta(a|b|f[\mu|c|e|d|c|d|D_v]f|f)_d + \frac{4}{3}\eta(a|b|f|c|c|e|d[\mu|d|D_v]f|f)_d + \frac{25}{24}\eta(a|b|f[\mu|c|f|d|f|D_v]e|c|d)_d + \\
& \frac{97}{48}f[\mu|c|f|d|d|D_v]e|c|a|b|_d + \frac{11}{16}f[\mu|d|f(a|c|D_v]e|c|b)_d - \frac{7}{48}f(a[\mu|f|c|d|D_v]e|c|b)_d + \frac{7}{144}\eta(a|b|f[\mu|c|f|d|f|D_v]e|d|c|f)_d - \\
& \frac{49}{48}f[\mu|c|f|c|d|D_v]e|d|a|b|_d - \frac{47}{24}f[\mu|d|f(a|c|D_v]e|d|b)_c - \frac{7}{48}f(a[\mu|f|c|d|D_v]e|d|b)_c + \frac{29}{144}\eta(a|b|f[\mu|c|f|d|f|D_v]e|f|c|d)_d \\
& - \frac{97}{48}f[\mu|c|f|d|d|D_v]e(a|b)_c - \frac{1}{16}f(c|d|f|c|[\mu D_v]e(a|b)_d + \frac{49}{24}f[\mu|c|f|c|d|D_v]e(a|b)_d - \frac{11}{16}f[\mu|d|f(a|c|D_v]e|b)_c|d)_d \\
& - \frac{2}{3}f(a[\mu|f|c|d|D_v]e|b)_c|d)_d + \frac{49}{24}f[\mu|c|f(a|b|D_v]e|d|c|d)_d + \frac{2}{3}f(a|c|f|b|[\mu D_v]e|d|c|d)_d + \frac{2}{3}f(a[\mu|f|b|c|D_v]e|d|c|d)_d \\
& - \frac{1}{48}f(c[\mu|f(a|c|D_v]e|d|b)_d + \frac{7}{24}f(a[\mu|f|c|c|D_v]e|d|b)_d + \frac{1}{12}\eta(a|b|f[\mu|c|f|d|d|D_v]e|f|c|f)_d - \\
& \frac{11}{18}\eta(a|b|f|c|d|f|c|[\mu D_v]e|f|d|f)_d - \frac{31}{72}\eta(a|b|f[\mu|c|f|c|d|D_v]e|f|d|f)_d + \frac{1}{48}f[\mu|c|e|d|v|d|D(a|f|b)_c + \frac{5}{16}f[\mu|c|e|c|v|d|D(a|f|b)_d \\
& + \frac{17}{48}f[\mu|c|e|v|c|d|D(a|f|b)_d - \frac{11}{16}f[\mu|c|e|d|c|d|D(a|f|b)_v] + \frac{1}{3}f[\mu|c|f|v|d|D(a|e|c|b)_d - \frac{11}{16}f[\mu|c|f|d|d|D(a|e|c|b)_v] \\
& - \frac{1}{3}f[\mu|c|f|v|d|D(a|e|d|b)_c - f|c|d|f|c|[\mu D(a|e|d|b)_v] + \frac{11}{16}f[\mu|c|f|c|d|D(a|e|d|b)_v] + \frac{1}{48}f[\mu|c|f|d|d|D(a|e|v|b)_c + \\
& \frac{1}{24}f|c|d|f|c|[\mu D(a|e|v|b)_d - \frac{17}{48}f[\mu|c|f|c|d|D(a|e|v|b)_d + \frac{1}{48}f|c|d|f|c|[\mu D(a|e|b)_d|v] - \frac{17}{48}f[\mu|c|f|c|d|D(a|e|b)_d|v] \\
& - \frac{3}{8}f[\mu|c|e|v|(a|d|D|b)f|c|d)_d + \frac{5}{48}f(a[\mu|e|v|c|d|D|b)f|c|d)_d - \frac{1}{3}f[\mu|c|e(a|v|d|D|b)f|c|d)_d - \frac{3}{8}f(a[\mu|e|c|v|d|D|b)f|c|d)_d \\
& + \frac{11}{16}f[\mu|c|e|d(a|v|D|b)f|c|d)_d - \frac{7}{16}e[\mu(a|f|v|c|e|d|d|D|b)f|c|f)_d + \frac{7}{16}e[\mu(a|f|v|c|e|c|d|d|D|b)f|d|f)_d \\
& + \frac{11}{24}e[\mu(a|f|v|c|e|d|c|d|D|b)f|d|f)_d + \frac{3}{8}f[\mu|c|e|c|(a|d|D|b)f|d|v] + \frac{1}{3}f[\mu|c|e(a|c|d|D|b)f|d|v] - \\
& \frac{5}{48}f(a[\mu|e|c|c|d|D|b)f|d|v] - \frac{1}{48}f[\mu|c|e|d(a|c|D|b)f|d|v] - \frac{11}{16}f[\mu|c|e|c|(a|v|D|b)f|d|d)_d + \frac{1}{48}f[\mu|c|e|v|(a|c|D|b)f|d|d)_d \\
& + \frac{3}{8}f(a[\mu|e|c|v|c|D|b)f|d|d)_d - \frac{11}{24}e[\mu(a|f|v|c|e|d|c|d|D|b)f|f|f)_d + \frac{1}{2}e[\mu(a|f|v|c|f|d|d|D|b)e|c|d|f)_d \\
& + \frac{7}{48}f(a[\mu|f|c|d|D|b)e|c|d|v] - \frac{1}{48}e[\mu(a|f|v|c|f|d|d|D|b)e|d|c|f)_d + \frac{21}{16}f[\mu|d|f(a|c|D|b)e|d|c|v] \\
& - \frac{25}{48}f(a[\mu|f|c|d|D|b)e|d|c|v] + \frac{23}{48}e[\mu(a|f|v|c|f|d|d|D|b)e|f|c|d)_d + \frac{17}{48}f[\mu|d|f(a|c|D|b)e|v|c|d)_d + \\
& \frac{2}{3}f(a[\mu|f|c|d|D|b)e|v|c|d)_d + \frac{47}{48}f[\mu|c|f(a|v|D|b)e|d|c|d)_d - \frac{47}{48}f|c|[\mu|f(a|c|D|b)e|d|v|d)_d + \frac{11}{8}f(a[\mu|f|c|c|D|b)e|d|v|d)_d \\
& - \frac{11}{24}e[\mu(a|f|v|c|f|d|d|D|b)e|f|c|f)_d - \frac{1}{18}e[\mu(a|f|c|c|d|f|c|v|D|b)e|f|d|f)_d - \frac{4}{9}e[\mu(a|f|v|c|f|c|d|D|b)e|f|d|f)_d + \\
& \frac{7}{48}f(a[\mu|e|v|b|c|D|d|f|c|d)_d + \frac{25}{48}f(a[\mu|e|b|v|c|D|d|f|c|d)_d - \frac{23}{48}f(a[\mu|e|c|b|c|D|d|f|d|v] - \frac{3}{16}f(a[\mu|e|c|v|c|D|d|f|b)_d - \\
& 2f[\mu|c|f(a|b|D|d|e|c|d|v] + \frac{23}{48}f(a|c|f|b|[\mu D|d|e|c|d|v] + \frac{23}{48}f(a[\mu|f|b|c|D|d|e|c|d|v] + \frac{29}{16}f[\mu|c|f(a|v|D|d|e|c|b)_d \\
& - \frac{1}{3}f(a|c|f|b|[\mu D|d|e|d|c|v] - \frac{1}{3}f(a[\mu|f|b|c|D|d|e|d|c|v] - \frac{1}{3}f[\mu|c|f(a|v|D|d|e|d|b)_c - \frac{25}{48}f(a|c|f|b|[\mu D|d|e|v|c|d)_d
\end{aligned}$$

$$\begin{aligned}
& -\frac{25}{48}f(a[\mu f b]cDde_v)cd - \frac{3}{16}f(a[\mu f |c|_c|Dd|e_v]b)_d - \frac{73}{48}f([\mu^c f(a_v)D|d|e b]_c d + f_c[\mu f(a|cDd|e b)|d|_v] \\
& - \frac{71}{48}f(a[\mu f |c|_c|Dd|e b]_d|_v) + \frac{1}{16}\eta^{ab}f([\mu^c e^d_v]dDff_c f) + \frac{1}{48}e_{[\mu}(a f_v)|c|e^d|b]_d Dff_c f - \\
& \frac{19}{48}\eta^{ab}f([\mu^c e|c|_v]dDff_d f) - \frac{17}{48}e_{[\mu}(a f_v)|c|e_c b]_d Dff_d f - \frac{13}{48}\eta^{ab}f([\mu^c e_v]c^d Dff_d f - \\
& \frac{5}{16}e_{[\mu}(a f_v)|c|e b]_c^d Dff_d f + \frac{29}{48}\eta^{ab}f([\mu^c e^d|c dDff_f|_v] + \frac{31}{48}e_{[\mu}(a f_v)|c|e^d c dDff|f b]_f \\
& - \frac{4}{3}\eta^{ab}f([\mu^c f_v]dDff_e c d f) - \frac{1}{48}e_{[\mu}(a f_v)|d|f b]_c Dff_e c d f - \frac{2}{9}e_{[\mu}(a f b)_v]f c^d Dff_e c d f + \\
& \frac{77}{48}\eta^{ab}f([\mu^c f^d|dDff_e c f|_v] + \frac{79}{48}e_{[\mu}(a f_v)|c f^d dDff|e c b]_f + \frac{4}{3}\eta^{ab}f([\mu^c f_v]dDff_e d c f - \\
& \frac{17}{48}e_{[\mu}(a f_v)|d|f b]_c Dff_e d c f - \frac{1}{9}e_{[\mu}(a f b)_v]f c^d Dff_e d c f - \frac{29}{48}\eta^{ab}f([\mu|c f c^d Dff_e d f|_v] - \\
& \frac{31}{48}e_{[\mu}(a f_v)cf|c dDff|e d b]_f - \frac{1}{3}e_{[\mu}(a f_v)|d|f b]_c Dff_e f c d + \frac{1}{16}\eta^{ab}f(c^d f_c[\mu Dff_e|f d|_v] + \\
& \frac{13}{48}\eta^{ab}f([\mu|c f c^d Dff_e f d|_v] + \frac{1}{48}e_{[\mu}(a f|c|d f c_v]Dff|e f b]_d + \frac{5}{16}e_{[\mu}(a f_v)cf|c dDff|e f b]_d \\
& + \frac{1}{16}\eta^{ab}f([\mu^c f^d|d|Dff_e v]_c f) + \frac{1}{8}\eta^{ab}f(c^d f_c[\mu Dff_e v]_d f) + \frac{13}{48}\eta^{ab}f([\mu|c|f c^d Dff_e v]_d f + \\
& \frac{1}{48}e_{[\mu}(a f_v)|c f^d dDff|e b]_c f) + \frac{1}{24}e_{[\mu}(a f|c|d f c_v]Dff|e b]_d f) + \frac{5}{16}e_{[\mu}(a f_v)cf|c dDff|e b]_d f
\end{aligned}$$
