# Supplementary material for: The non-linear coupled spin 2 - spin 3 Cotton equation in three dimensions
Source: arXiv:1602.01682 ancillary file (2016-03-18)
Supplement: Supplementary file 2 [file cotton_spin3_metric.pdf]

$$\begin{aligned}
& \frac{1}{6}D_{[\mu D \nu] D} (a D | c | D c h b) d_a + \frac{1}{12}D_{[\mu D \nu] D} (a D | c | D b) h_c d_a - \frac{1}{6}D_{[\mu D \nu] D} (a D | c D d | h b) c_a - \frac{1}{6}D_{[\mu D \nu] D} c D (a D c h b) d_a \\
& - \frac{1}{12}D_{[\mu D \nu] D} c D (a D b) h_c d_a + \frac{1}{6}D_{[\mu D \nu] D} c D (a D | d | h b) c_a + \frac{1}{6}D_{[\mu D \nu] D} c D d D c h (a b) d_a - \frac{1}{6}D_{[\mu D \nu] D} c D d D d h (a b) c \\
& + \frac{11}{192}D_{[\mu D (a D \nu) D b] D} c h c d_a - \frac{5}{96}D_{[\mu D (a D \nu) D | c | D c h b) d_a} - \frac{1}{12}D_{[\mu D (a D \nu) D | c | D b) h c d_a} \\
& + \frac{5}{96}D_{[\mu D (a D \nu) D | c D d | h b) c_a} - \frac{11}{192}D_{[\mu D (a D b) D \nu] D} c h c d_a + \frac{5}{96}D_{[\mu D (a D b) D c D | c | h d \nu] d_a} \\
& + \frac{1}{12}D_{[\mu D (a D b) D c D \nu] h c d_a} - \frac{5}{96}D_{[\mu D (a D b) D c D d h | c d | \nu]} - \frac{1}{12}D_{[\mu D (a D | c | D | c | D \nu] h b) d_a} \\
& + \frac{1}{12}D_{[\mu D (a D | c | D | c | D b) h d \nu] d_a} + \frac{1}{12}D_{[\mu D (a D | c | D \nu] D c h b) d_a} + \frac{1}{6}D_{[\mu D (a D | c | D \nu] D b) h c d_a} \\
& - \frac{1}{6}D_{[\mu D (a D | c D \nu] D d | h b) c_a} - \frac{1}{12}D_{[\mu D (a D | c | D b) D | c | h d \nu] d_a} - \frac{1}{6}D_{[\mu D (a D | c | D b) D \nu] h c d_a} \\
& + \frac{1}{6}D_{[\mu D (a D | c | D b) D d h | c d | \nu]} + \frac{1}{6}D_{[\mu D (a D | c D d | \nu] h b) c_a} - \frac{1}{6}D_{[\mu D (a D | c D d | b) h | c d | \nu]} - \\
& \frac{9}{64}D_{[\mu D c D | c | D \nu] D (a h b) d_a} + \frac{11}{192}\eta^{a b} D_{[\mu D c D | c | D \nu] D d h d^f f} + \frac{3}{16}D_{[\mu D c D | c | D \nu] D d h (a b) d_a} \\
& + \frac{43}{192}D_{[\mu D c D | c | D (a D \nu] h b) d_a} + \frac{1}{24}D_{[\mu D c D | c | D (a D b) h d \nu] d_a} - \frac{17}{96}D_{[\mu D c D | c D (a D | d | h b) d | \nu]} + \\
& \frac{1}{12}D_{[\mu D c D | c D d d | h (a b) \nu]} - \frac{11}{288}\eta^{a b} D_{[\mu D c D | c D d d | h^f \nu] f} - \frac{11}{144}\eta^{a b} D_{[\mu D c D | c | D d \nu] h d^f f} \\
& - \frac{13}{48}D_{[\mu D c D | c | D d \nu] h (a b) d_a} + \frac{3}{32}D_{[\mu D c D | c D d d (a h b) d | \nu]} + \frac{11}{288}\eta^{a b} D_{[\mu D c D | c D d d^f h d f | \nu]} \\
& + \frac{9}{64}D_{[\mu D c D \nu] D c D (a h b) d_a} - \frac{11}{192}\eta^{a b} D_{[\mu D c D \nu] D c D d h d^f f} - \frac{3}{16}D_{[\mu D c D \nu] D c D d h (a b) d_a} \\
& - \frac{11}{192}D_{[\mu D c D \nu] D (a D c h b) d_a} + \frac{1}{24}D_{[\mu D c D \nu] D (a D b) h c d_a} + \frac{1}{96}D_{[\mu D c D \nu] D (a D | d | h b) c_a} + \\
& \frac{7}{144}\eta^{a b} D_{[\mu D c D \nu] D d D c h d^f f} + \frac{5}{48}D_{[\mu D c D \nu] D d D c h (a b) d_a} - \frac{5}{288}\eta^{a b} D_{[\mu D c D \nu] D d D d h c^f f} \\
& + \frac{1}{12}D_{[\mu D c D \nu] D d D d h (a b) c} - \frac{3}{32}D_{[\mu D c D \nu] D d D (a h b) c_a} + \frac{5}{288}\eta^{a b} D_{[\mu D c D \nu] D d D^f h c d f} - \\
& \frac{13}{96}D_{[\mu D c D (a D | c | D \nu] h b) d_a} - \frac{25}{192}D_{[\mu D c D (a D | c | D b) h d \nu] d_a} + \frac{17}{96}D_{[\mu D c D (a D | c D | d | h b) d | \nu]} \\
& + \frac{5}{96}D_{[\mu D c D (a D \nu) D c h b) d_a} - \frac{7}{192}D_{[\mu D c D (a D \nu) D b) h c d_a} - \frac{1}{96}D_{[\mu D c D (a D \nu) D | d | h b) c_a} + \\
& \frac{3}{64}D_{[\mu D c D (a D b) D | c | h d \nu] d_a} - \frac{3}{64}D_{[\mu D c D (a D b) D \nu] h c d_a} - \frac{3}{32}D_{[\mu D c D (a D | d | D | c h b) d | \nu]} - \\
& \frac{1}{12}D_{[\mu D c D (a D | d | D | d h b) c | \nu]} + \frac{3}{32}D_{[\mu D c D (a D | d | D \nu] h b) c_a} + \frac{1}{12}D_{[\mu D c D (a D | d | D b) h | c d | \nu]} + \\
& \frac{13}{144}\eta^{a b} D_{[\mu D c D d D | c D d | h^f \nu] f} + \frac{5}{36}\eta^{a b} D_{[\mu D c D d D | c | D \nu] h d^f f} - \frac{11}{72}\eta^{a b} D_{[\mu D c D d D | c D^f h d f | \nu]} \\
& - \frac{1}{16}\eta^{a b} D_{[\mu D c D d D | d D c | h^f \nu] f} + \frac{1}{16}\eta^{a b} D_{[\mu D c D d D | d | D \nu] h c^f f} - \frac{1}{9}\eta^{a b} D_{[\mu D c D d \nu] D c h d^f f} \\
& - \frac{5}{144}\eta^{a b} D_{[\mu D c D d \nu] D d h c^f f} + \frac{7}{72}\eta^{a b} D_{[\mu D c D d \nu] D^f h c d f} + \frac{1}{8}\eta^{a b} D_{[\mu D c D d^f D | c h d f | \nu]} - \\
& \frac{1}{36}\eta^{a b} D_{[\mu D c D d^f D | d h c f | \nu]} + \frac{1}{36}\eta^{a b} D_{[\mu D c D d^f D | f h c d | \nu]} - \frac{1}{8}\eta^{a b} D_{[\mu D c D d^f D \nu] h c d f} + \\
& \frac{13}{192}e_{[\mu (a D \nu) D | c | D c D b) D d h d^f f} + \frac{1}{48}e_{[\mu (a D \nu) D | c D c D d | D d h b) f f} - \frac{11}{192}e_{[\mu (a D \nu) D | c D c D d | D b) h d^f f} - \\
& \frac{1}{48}e_{[\mu (a D \nu) D | c D c D d^f | h b) d f} - \frac{13}{192}e_{[\mu (a D \nu) D | c | D b) D c D d h d^f f} + \frac{11}{192}e_{[\mu (a D \nu) D | c | D b) D d D c h d^f f}
\end{aligned}$$

$$\begin{aligned}
& -\frac{1}{48}e_{[\mu} (aD_{\nu]}D|c|D^b)D^dD_d h_c^f f + \frac{1}{48}e_{[\mu} (aD_{\nu]}D|c|D^b)D^dD^f h_c^d f + \frac{11}{192}e_{[\mu} (aD_{\nu]}D|cD^d|D_cD_d h^b) f f \\
& + \frac{11}{96}e_{[\mu} (aD_{\nu]}D|cD^d|D_cD^b)h_d^f f - \frac{11}{96}e_{[\mu} (aD_{\nu]}D|cD^dD_cD^f|h^b) f f - \frac{11}{192}e_{[\mu} (aD_{\nu]}D|cD^d|D_dD_c h^b) f f \\
& + \frac{11}{192}e_{[\mu} (aD_{\nu]}D|cD^d|D_dD^b)h_c^f f - \frac{11}{96}e_{[\mu} (aD_{\nu]}D|cD^d|D^b)D_c h_d^f f - \frac{11}{192}e_{[\mu} (aD_{\nu]}D|cD^d|D^b)D_d h_c^f f \\
& + \frac{11}{96}e_{[\mu} (aD_{\nu]}D|cD^d|D^b)D^f h_c^d f + \frac{11}{96}e_{[\mu} (aD_{\nu]}D|cD^dD^f|D_c h^b) f f - \frac{11}{96}e_{[\mu} (aD_{\nu]}D|cD^dD^f|D^b)h_c^d f \\
& - \frac{1}{64}f_{[\mu} c^D|c|D_{\nu]}D(a h^b)^d_d + \frac{3}{64}\eta^{ab}f_{[\mu} c^D|c|D_{\nu]}D^d h_d^f f + \frac{1}{48}f_{[\mu} c^D|c|D_{\nu]}D^d h_d(a b)_d \\
& + \frac{67}{192}f_{[\mu} c^D|c|D(aD_{\nu]}h^b)^d_d + \frac{1}{6}f_{[\mu} c^D|c|D(aD^b)h^d_{\nu]}_d - \frac{11}{32}f_{[\mu} c^D|cD(aD|d|h^b)_d|_{\nu]} + \\
& \frac{7}{64}e_{[\mu} (a f_{\nu]}|c|D_cD^b)D^d h_d^f f + \frac{1}{3}f_{[\mu} c^D|cD^dD_d|h(a b)_{\nu]} - \frac{5}{48}e_{[\mu} (a f_{\nu]}|cD_cD^d|D_d h^b) f f - \\
& \frac{5}{24}\eta^{ab}f_{[\mu} c^D|cD^dD_d|h^f_{\nu]}_f - \frac{29}{192}\eta^{ab}f_{[\mu} c^D|c|D^dD_{\nu]}h_d^f f - \frac{17}{48}f_{[\mu} c^D|c|D^dD_{\nu]}h_d(a b)_d + \\
& \frac{1}{96}f_{[\mu} c^D|cD^dD(a h^b)_d|_{\nu]} - \frac{31}{192}e_{[\mu} (a f_{\nu]}|cD_cD^d|D^b)h_d^f f + \frac{5}{24}\eta^{ab}f_{[\mu} c^D|cD^dD^f h_d f|_{\nu]} \\
& + \frac{5}{48}e_{[\mu} (a f_{\nu]}|cD_cD^dD^f|h^b) f f + \frac{1}{3}D_cD_{[\nu}f^d|d|D_{\mu]}h(a b)_c - \frac{1}{3}D_cD(a f|d|_dD_{[\mu}h^b)_c]_{\nu]} - \\
& \frac{3}{8}D_cD_{[\nu}f(a|d|D_{\mu]}h^b)_c^d + \frac{3}{8}D_cD(a f_{[\nu}|d|D_{\mu]}h^b)_c^d + \frac{1}{48}D_cD_{[\nu}f(a|d|D_{\mu]}h^b)_c^d - \frac{1}{48}D_cD(a f_{[\nu}|d|D_{\mu]}h^b)_c^d c \\
& + \frac{19}{96}D_cD_{[\nu}f(a b)_D_{\mu]}h_c^d d - \frac{35}{192}D_cD(a f^b)_{[\nu}D_{\mu]}h_c^d d + \frac{1}{9}\eta^{ab}D_cD_d f^f f D_{[\mu}h_c^d]_{\nu]} + \frac{1}{3}D_cD(a f^b)_d D_{[\mu}h_c^d]_{\nu]} \\
& - \frac{1}{4}\eta^{ab}D_cD_d f_{[\nu}|f|D_{\mu]}h_c^d f + \frac{71}{432}\eta^{ab}D_cD_{[\nu}f|d f|D_{\mu]}h_c^d f - \frac{605}{1728}\eta^{ab}D_cD_{[\nu}f^d|d|D_{\mu]}h_c^f f + \\
& \frac{29}{144}\eta^{ab}D_cD_d f_d_{[\nu}D_{\mu]}h_c^f f - \frac{1}{9}\eta^{ab}D_cD_d f_d f D_{[\mu}h_c^f]_{\nu]} + \frac{3}{8}D_cD_{[\nu}f(a b)_D_{\mu]}h_c^d d - \frac{17}{48}D_cD(a f^b)_{[\nu}D_{\mu]}h_c^d d \\
& - \frac{1}{4}\eta^{ab}D_cD_d f_{[\nu}|f|D_{\mu]}h_c^d f - \frac{13}{432}\eta^{ab}D_cD_{[\nu}f|d f|D_{\mu]}h_c^d f + \frac{13}{432}\eta^{ab}D_cD_{[\nu}f^d|d|D_{\mu]}h_c^f f \\
& + \frac{11}{36}\eta^{ab}D_cD_d f_d_{[\nu}D_{\mu]}h_c^f f + \frac{7}{36}\eta^{ab}D_cD_d f_{[\nu}|f|D_{\mu]}h_c^f d - \frac{17}{96}D_cD_{[\nu}h(a|d|_d|D_{\mu]}f^b)_c \\
& + \frac{1}{6}D_cD(a h|d|_{[\nu}|d|D_{\mu]}f^b)_c + \frac{13}{96}D_cD(a h^b)_d D_{[\mu}f^c]_{\nu]} - \frac{5}{36}\eta^{ab}D_cD^d h_d^f f D_{[\mu}f^c]_{\nu]} - \\
& \frac{31}{72}\eta^{ab}D_cD_d h^f_{[\nu}|f|D_{\mu]}f^c d + \frac{1}{24}D_cD_{[\nu}h(a b)_d|D_{\mu]}f^c d - \frac{1}{48}D_cD(a h^b)_{[\nu}|d|D_{\mu]}f^c d + \\
& \frac{17}{96}\eta^{ab}D_cD_{[\nu}h^d|f_d|D_{\mu]}f^c f + \frac{7}{36}\eta^{ab}D_cD^d h_d_{[\nu}|f|D_{\mu]}f^c f - \frac{9}{16}\eta^{ab}f^c d D_{[\mu}D|cD_d|h^f_{\nu]}_f \\
& - \frac{7}{27}\eta^{ab}h^c d f D_{[\mu}D|cD_d f f|_{\nu]} - \frac{1}{12}f^c d D_{[\mu}D|c|D_{\nu]}h(a b)_d - \frac{7}{32}f(a|c|D_{[\mu}D|c|D_{\nu]}h^b)_d d \\
& + \frac{11}{48}\eta^{ab}h^c d f D_{[\mu}D|c|D_{\nu]}f_d f - \frac{3}{8}h(a|c d|D_{[\mu}D|c|D_{\nu]}f^b)_d + \frac{1}{3}h(a b)_c D_{[\mu}D|c|D_{\nu]}f^d_d \\
& + \frac{1}{24}f^c d D_{[\mu}D|cD(a h^b)_d|_{\nu]} + \frac{7}{32}f(a|c|D_{[\mu}D|c|D^b)h_d^d_{\nu]}_d + \frac{3}{8}h(a|c d|D_{[\mu}D|cD^b) f_d|_{\nu]} + \\
& \frac{4}{9}\eta^{ab}f^c d D_{[\mu}D|cD^f h_d f|_{\nu]} - f^c d D_{[\mu}D|dD_c|h(a b)_{\nu]} - \frac{1}{16}\eta^{ab}f^c d D_{[\mu}D|dD_c|h^f_{\nu]}_f - \\
& \frac{13}{54}\eta^{ab}h^c d f D_{[\mu}D|dD_c f f|_{\nu]} + \frac{7}{36}\eta^{ab}h^c d f D_{[\mu}D|dD^f c|_{\nu]} + \frac{223}{288}\eta^{ab}f^c d D_{[\mu}D|d|D_{\nu]}h_c^f f \\
& - f^c d D_{[\mu}D|d|D_{\nu]}h(a b)_c + \frac{5}{144}\eta^{ab}h^c d f D_{[\mu}D|d|D_{\nu]}f_c f + \frac{3}{8}h^c c^d D_{[\mu}D|d|D_{\nu]}f(a b)_c + \\
& \frac{7}{24}h^c d c^D D_{[\mu}D|d|D_{\nu]}f(a b)_c + \frac{1}{48}h(a|c d|D_{[\mu}D|d|D_{\nu]}f^b)_c - \frac{5}{144}\eta^{ab}h^c c^d D_{[\mu}D|d|D_{\nu]}f^f f
\end{aligned}$$

$$\begin{aligned}
& -\frac{61}{144}\eta^{ab}h^cd^cD[\mu D|d|Dv]f^ff + f^cdD[\mu D|dD(ahb)|c|v] - \frac{17}{48}h^cd^cD[\mu D|d|D(afb)|v] - \\
& \frac{13}{48}h^cd^cD[\mu D|d|D(afb)|v] - \frac{1}{48}h^c|cd|D[\mu D|dD(b)f|c|v] - \frac{2}{3}\eta^{ab}f^cdD[\mu D|dD^fh^cf|v] + \\
& \frac{11}{36}\eta^{ab}h^cd^cD[\mu D|dD^ff|v] + \frac{5}{18}\eta^{ab}h^cd^cD[\mu D|dD^ff|v] - \frac{1}{3}D^cf^dD[\mu Dv]h^c(b)c - \\
& \frac{3}{8}D^cf^c(a_dD[\mu Dv]h^b)c^d + \frac{17}{48}D^cf^c(a_dD[\mu Dv]h^b)d^c + \frac{35}{96}D^cf^c(ab)D[\mu Dv]h^cd^d + \frac{71}{432}\eta^{ab}D^cf^dD[\mu Dv]h^cd^f \\
& - \frac{941}{1728}\eta^{ab}D^cf^dD[\mu Dv]h^cf^f + \frac{3}{8}D^cf^c(ab)D[\mu Dv]h^cd^d - \frac{13}{432}\eta^{ab}D^cf^dD[\mu Dv]h^cd^f \\
& + \frac{13}{432}\eta^{ab}D^cf^dD[\mu Dv]h^cf^f - \frac{61}{96}D^ch^c(a|d|dD[\mu Dv]f^b)c + \frac{41}{24}D^ch^c(ab)_dD[\mu Dv]f^cd + \\
& \frac{7}{288}\eta^{ab}D^ch^d^fdD[\mu Dv]f^cf - \frac{1}{12}\eta^{ab}D^ch^d^fdD[\mu Dv]f^fc + \frac{1}{18}\eta^{ab}f^cdD[\mu Dv]D^ch^d^ff + \\
& \frac{5}{3}f^cdD[\mu Dv]D^ch^c(ab)_d - \frac{7}{8}f^c(a|c|D[\mu Dv]D^ch^b)_d - \frac{2}{3}h^c(ab)_cD[\mu Dv]D^cf^d^d - \frac{1}{12}\eta^{ab}f^cdD[\mu Dv]D^ch^cf^f \\
& + \frac{1}{6}h^cd^cD[\mu Dv]D^df^c(ab) + \frac{1}{3}h^c(a|cd|D[\mu Dv]D^df^b)_c - \frac{1}{18}\eta^{ab}h^cd^cD[\mu Dv]D^df^ff - \\
& \frac{5}{6}f^cdD[\mu Dv]D^ch^b)_c^d + \frac{37}{24}f^cd^cD[\mu Dv]D^ch^b)_d^d + \frac{1}{8}f^c(a|c|D[\mu Dv]D^b)_h^cd^d - \frac{1}{3}h^c(a|cd|D[\mu Dv]D^b)_f^cd + \\
& \frac{5}{12}h^c(a|c|cD[\mu Dv]D^b)_f^d^d - \frac{1}{12}f^c(ab)D[\mu Dv]D^ch^cd^d - \frac{1}{18}\eta^{ab}f^cdD[\mu Dv]D^dh^d^ff - \frac{8}{3}f^cdD[\mu Dv]D^dh^c(ab)_d \\
& + \frac{5}{6}f^c(a|cdD[\mu Dv]D^d|h^b)_c^d + \frac{2}{3}h^c(ab)_cD[\mu Dv]D^df^cd - \frac{1}{2}h^c(a|cD[\mu Dv]D^d|f^b)_d + \frac{1}{18}\eta^{ab}h^cd^cD[\mu Dv]D^ff^d^f \\
& - \frac{1}{3}D^cf^d^dD[\mu D(ahb)|c|v] + \frac{3}{8}f^cdD[\mu D(adv)h^b)_c^d + \frac{5}{24}f^cdD[\mu D(adv)h^b)_d^d + \frac{11}{48}h^cd^cD[\mu D(adv)f^b)_d - \\
& \frac{89}{192}h^cd^cD[\mu D(adv)f^b)_d - \frac{3}{8}f^cdD[\mu D(adv)h^b)_c|d|v] - \frac{5}{24}f^cdD[\mu D(adv)h^b)_d|v] - \frac{11}{48}h^cd^cD[\mu D(adv)f^b)_d|v] \\
& + \frac{89}{192}h^cd^cD[\mu D(adv)f^b)_d|v] - \frac{1}{3}D^cf^c(a_dD[\mu D(b)h^cd^d|v] + \frac{1}{3}D^cf^c(a_dD[\mu D(b)h^cd^d|v] - \frac{95}{96}D^ch^c(a|d|dD[\mu D(b)f^c|v] \\
& + \frac{19}{24}f^c(a|c|D[\mu D(b)D|c|h^d|v] + \frac{2}{3}h^c(a|cd|D[\mu D(b)D|cf^d|v] - \frac{1}{3}h^c(a|cd|D[\mu D(b)D|df^c|v] - \\
& \frac{27}{32}f^c(a|c|D[\mu D(b)D|v]h^cd^d - \frac{1}{8}h^c(a|cd|D[\mu D(b)D|v]f^cd + \frac{1}{3}h^c(a|c|cD[\mu D(b)D|v]f^d^d + \frac{1}{6}f^c(a|c|D[\mu D(b)D^dh^c|d|v] \\
& - \frac{2}{3}h^c(a|c|cD[\mu D(b)D^df^d|d|v] + \frac{1}{3}D^cf^d^dD[\mu D^ch^c(ab)|v] + \frac{1}{48}D^cf^c(a_dD[\mu D|c|h^b)_d|v] - \frac{5}{6}D^cf^c(ab)_D[\mu D^ch^d|v]d \\
& - \frac{11}{72}\eta^{ab}D^cf^d^fD[\mu D^ch^d^ff|v] + \frac{79}{144}\eta^{ab}D^cf^d^dD[\mu D^ch^ff|v] + \frac{51}{32}D^ch^c(a|d^dD[\mu D^cf^b)|v] \\
& - \frac{19}{12}D^ch^c(ab)_dD[\mu D^cf^d|v] - \frac{109}{288}\eta^{ab}D^ch^d^fdD[\mu D^cf^f|v] - \frac{25}{48}f^c(ab)_D[\mu D^cd|c|h^d|v]d \\
& + \frac{125}{48}f^c(ab)_D[\mu D^cdv]h^cd^d - 2f^c(ab)_D[\mu D^cd^dh^c|d|v] + \frac{7}{18}\eta^{ab}D^cf^d^fD[\mu D^dh^cf^f|v] - \\
& \frac{11}{36}\eta^{ab}D^cf^d^fD[\mu D^dh^cf^f|v] - D^ch^c(ab)_dD[\mu D^df^c|v] + \frac{3}{2}f^c(a|cD[\mu D^d|D|ch^b)_d|v] + \frac{7}{3}f^cdD[\mu D^dd|d|h^c(ab)|v] \\
& - \frac{37}{24}f^c(a|cD[\mu D^d|D|d|h^b)_c|v] + \frac{1}{4}\eta^{ab}f^cdD[\mu D^dd|d|h^ff|v] - \frac{17}{24}h^c(ab)_cD[\mu D^dd|d|df^c|v] \\
& + \frac{5}{8}h^c(a|cD[\mu D^d|D|d|f^b)|v] - \frac{11}{8}\eta^{ab}f^cdD[\mu D^ddv]h^d^ff + \frac{7}{3}f^cdD[\mu D^ddv]h^c(ab)_d - \\
& \frac{31}{24}f^c(a|cD[\mu D^d|Dv]h^b)_c^d + \frac{1}{24}h^c(ab)_cD[\mu D^ddv]f^cd - \frac{1}{8}h^c(a|cD[\mu D^d|Dv]f^b)_d - \frac{7}{3}f^cdD[\mu D^dd(ahb)|d|v] \\
& + \frac{4}{3}f^c(a|cD[\mu D^d|D^b)h^c|d|v] + \frac{1}{12}h^c(a|cD[\mu D^d|D^b)f^d|d|v] + \frac{10}{9}\eta^{ab}f^cdD[\mu D^dd^fh^d|d|v] +
\end{aligned}$$

$$\begin{aligned} & \frac{2}{9}\eta^{ab}D_c f^d{}_d D[\mu D^f h_{|f|} c_v] + \frac{1}{8}\eta^{ab}D_c h^d{}_d f^c{}_c D[\mu D^f f^c{}_c v] - \frac{17}{18}\eta^{ab}f^c{}_c d^c{}_d D[\mu D^f D_{|c} h^d{}_d f_{|v|}] - \\ & \frac{1}{36}\eta^{ab}h^c{}_c d^c{}_d D[\mu D^f D_{|d} f_{|f|} v] + \frac{31}{72}\eta^{ab}f^c{}_c d^c{}_d D[\mu D^f D_{|f} h^c{}_d v] + \frac{11}{48}\eta^{ab}h^c{}_c d^c{}_d D[\mu D^f D_{|f} f^d{}_d v] \\ & - \frac{271}{576}\eta^{ab}h^c{}_c d^c{}_d D[\mu D^f D_{|f} f^d{}_d v] + \frac{37}{72}\eta^{ab}f^c{}_c d^c{}_d D[\mu D^f D_{|v|} h^c{}_d f] - \frac{11}{48}\eta^{ab}h^c{}_c d^c{}_d D[\mu D^f D_{|v|} f^d{}_d f] \\ & + \frac{239}{576}\eta^{ab}h^c{}_c d^c{}_d D[\mu D^f D_{|v|} f^d{}_d f] + \frac{37}{72}\eta^{ab}D[\mu D^c f^d{}_d D_{|v|} h^c{}_d f] - \frac{19}{32}D[\mu D^c (af^b) c D_{|v|} h^c{}_d f] + \\ & \frac{101}{48}D[\mu D^c f^d (ab) D_{|v|} h^c{}_d f] - \frac{31}{24}\eta^{ab}D[\mu D^c f^d d_{|d|} D_{|v|} h^c{}_f f] + \frac{199}{288}\eta^{ab}D[\mu D^c f^d c_{|c|} d D_{|v|} h^d{}_f f] + \\ & \frac{11}{6}D[\mu D^c f^d d_{|d|} D_{|v|} h^c (ab) c] - \frac{13}{12}D[\mu D^c f^d c_{|c|} d D_{|v|} h^c (ab) d] + \frac{3}{8}D[\mu D^c (af^b c_{|d|} D_{|v|} h^b) c d] - \frac{31}{24}D[\mu D^c f^d (a d_{|d|} D_{|v|} h^b) c d] \\ & + \frac{11}{24}D[\mu D^c (af^b c_{|c|} c_{|c|} D_{|v|} h^b) d] - \frac{7}{32}D[\mu D^c f^d (a c_{|c|} D_{|v|} h^b) d] - \frac{11}{48}e[\mu^{(a} D_{|c} d f^b)_{f|} D_{|v|} h^c{}_d f] + \\ & \frac{7}{36}e[\mu^{(a} D_{|c} d^b) f^d{}_d D_{|v|} h^c{}_d f] - \frac{119}{288}e[\mu^{(a} D_{|c} d^b) f^d{}_d D_{|v|} h^c{}_f f] + \frac{11}{64}e[\mu^{(a} D_{|c} d^b d_{|d|} f^b)_{d|} D_{|v|} h^c{}_f f] \\ & - \frac{11}{48}e[\mu^{(a} D_{|c} d^b f^b)_{f|} D_{|v|} h^d{}_c f] - \frac{5}{144}e[\mu^{(a} D_{|c} d^b) f^d{}_d D_{|v|} h^d{}_c f] + \frac{5}{144}e[\mu^{(a} D_{|c} d^b) f^d{}_d D_{|v|} h^f{}_c f] \\ & + \frac{11}{48}e[\mu^{(a} D_{|c} d^b d_{|d|} f^b)_{d|} D_{|v|} h^f{}_c f] + \frac{11}{48}e[\mu^{(a} D_{|c} d^b f^b)_{f|} D_{|v|} h^f{}_c d] - \frac{1}{8}D[\mu D^c (ah^b) c^d D_{|v|} f^c{}_d] \\ & + \frac{1}{24}D[\mu D^c h^d (ab) d D_{|v|} f^c{}_d] - \frac{19}{48}\eta^{ab}D[\mu D^c h^d d_{|d|} f^c{}_d D_{|v|} f^c{}_f] + \frac{191}{576}\eta^{ab}D[\mu D^c h^d f^c{}_d d_{|d|} D_{|v|} f^c{}_f] \\ & + \frac{31}{72}\eta^{ab}D[\mu D^c h^d c_{|c|} d^c{}_d D_{|v|} f^d{}_d f] + \frac{2}{3}D[\mu D^c h^d c^d{}_d D_{|v|} f^c (ab)] + \frac{3}{8}D[\mu D^c h^d (a d_{|d|} d_{|d|} D_{|v|} f^b) c] + \\ & \frac{11}{48}D[\mu D^c (ah^b c^c c_{|c|} d_{|d|} D_{|v|} f^b) d] - \frac{41}{192}D[\mu D^c (ah^b c^c d_{|d|} c_{|c|} D_{|v|} f^b) d] - \frac{41}{48}D[\mu D^c h^d (a c_{|c|} d_{|d|} D_{|v|} f^b) d] - \\ & \frac{11}{96}e[\mu^{(a} D_{|c} d^b d_{|d|} h^d f^c_{|f|} D_{|v|} f^b) c] - \frac{11}{24}e[\mu^{(a} D_{|c} d^b h^b) f^c_{|f|} D_{|v|} f^c{}_d] + \frac{5}{24}e[\mu^{(a} D_{|c} d^b) h^d{}_d f^c_{|f|} D_{|v|} f^c{}_f] \\ & + \frac{11}{48}e[\mu^{(a} D_{|c} d^b d_{|d|} h^b)_{d|} f^c_{|f|} D_{|v|} f^c{}_f] - \frac{5}{12}D[\mu D^c (ah^b) c^c c_{|c|} D_{|v|} f^d{}_d] + \frac{4}{3}D[\mu D^c h^d (ab) c_{|c|} D_{|v|} f^d{}_d] \\ & - \frac{3}{8}\eta^{ab}D[\mu D^c h^d c^c d_{|d|} D_{|v|} f^c{}_f] - \frac{19}{192}\eta^{ab}D[\mu f^c{}_c d^c{}_d D_{|v|} D_{|c} h^d{}_d f^c{}_f] - \frac{1}{24}D[\mu f^c{}_c d^c{}_d D_{|v|} D_{|c} h^d (ab) d] \\ & - \frac{3}{8}D[\mu f^c (a c_{|c|} D_{|v|} D_{|c} h^b) d] - \frac{109}{144}\eta^{ab}D[\mu h^c{}_c d^c{}_d D_{|v|} D_{|c} f^d{}_d f] + \frac{21}{16}D[\mu h^c (a c_{|c|} d_{|d|} D_{|v|} D_{|c} f^b) d] - \\ & \frac{11}{6}D[\mu h^c (ab) c^c D_{|v|} D_{|c} f^d{}_d] - \frac{119}{192}e[\mu^{(a} f^c c_{|d|} D_{|v|} D_{|c} d^b h^b) f^c_{|f|}] - \frac{17}{72}e[\mu^{(a} h^c c^d f^c_{|d|} D_{|v|} D_{|c} d^b f^b)_{f|}] \\ & - \frac{1}{9}\eta^{ab}h^c_{|c} d^c_{|d} D_{|v|} D_{|c} d^b f^c_{|f|} f^c_{|f|} + \frac{203}{192}f[\mu^c D_{|v|} D_{|c} D_{|c} (ah^b) d] - \frac{1}{3}h[\mu^c d^c D_{|v|} D_{|c} D_{|c} (af^b) d] - \\ & \frac{1}{64}e[\mu^{(a} f^c c_{|d|} D_{|v|} D_{|c} d^b) h^d{}_d f^c_{|f|}] + \frac{13}{48}e[\mu^{(a} h^c c^d f^c_{|d|} D_{|v|} D_{|c} d^b) f^d{}_d f^c_{|f|}] + \frac{1}{3}h[a_{|c|} \mu^c D_{|v|} D_{|c} d^b) f^d{}_d f^c_{|f|}] \\ & - \frac{35}{576}\eta^{ab}f^c_{|c} d^c_{|d} D_{|v|} D_{|c} d^b h^d{}_d f^c_{|f|} - \frac{97}{48}f[\mu^c D_{|v|} D_{|c} d^b h^d (ab) d] + \frac{13}{24}e[\mu^{(a} f^c c_{|d|} D_{|v|} D_{|c} d^b f^c_{|f|} h^b)_{d|}] \\ & + \frac{1}{9}\eta^{ab}h^c_{|c} d^c_{|d} D_{|v|} D_{|c} d^b f^c_{|f|} f^c_{|f|} + \frac{47}{288}\eta^{ab}D[\mu f^c{}_c d^c{}_d D_{|v|} D_{|c} h^c{}_d f^c{}_f] - \frac{5}{144}\eta^{ab}D[\mu h^c{}_c d^c{}_d D_{|v|} D_{|c} f^c{}_f] \\ & - \frac{3}{8}D[\mu h^c c^c c_{|c|} d^c_{|d} D_{|v|} D_{|c} f^c (ab)] - \frac{83}{48}D[\mu h^c c^c c_{|c|} d^c_{|d} D_{|v|} D_{|c} f^c (ab)] - \frac{1}{48}D[\mu h^c (a c_{|c|} d_{|d|} D_{|v|} D_{|c} f^b) c] - \\ & \frac{35}{144}\eta^{ab}D[\mu h^c c^c c_{|c|} d^c_{|d} D_{|v|} D_{|c} f^c f^c_{|f|}] + \frac{221}{144}\eta^{ab}D[\mu h^c c^c c_{|c|} d^c_{|d} D_{|v|} D_{|c} f^c f^c_{|f|}] - \frac{143}{192}e[\mu^{(a} f^c c_{|d|} D_{|v|} D_{|c} d^b h^b) f^c_{|f|}] \\ & - \frac{2}{9}e[\mu^{(a} h^c c^d f^c_{|d|} D_{|v|} D_{|c} d^b) f^c_{|f|}] + \frac{11}{48}e[\mu^{(a} h^c c^d f^c_{|d|} D_{|v|} D_{|c} d^b f^c_{|f|} b) c] + \frac{47}{64}e[\mu^{(a} f^c c_{|d|} D_{|v|} D_{|c} d^b) h^c{}_c f^c_{|f|}] + \\ & \frac{1}{24}e[\mu^{(a} h^c c^d f^c_{|d|} D_{|v|} D_{|c} d^b) f^c_{|f|}] - \frac{1}{24}e[\mu^{(a} h^c c^c c_{|c|} d^c_{|d} D_{|v|} D_{|c} d^b) f^c_{|f|}] - \frac{1}{2}e[\mu^{(a} h^c c^c c_{|c|} d^c_{|d} D_{|v|} D_{|c} d^b) f^c_{|f|} f^c_{|f|}] \end{aligned}$$

$$\begin{aligned}
& + \frac{11}{48} e [\mu (a h | c | c | d v) D d f | f b) f + \frac{11}{48} e [\mu (a h | c d | c | d v) D d f | f b) f + \frac{5}{18} \eta a b D [\mu h^c d f D v] D f f c d \\
& + \frac{1}{8} D [\mu f^c d D v] D (a h b) c d - \frac{25}{24} D c f [\mu | d | D v] D (a h b) c d + \frac{5}{12} D [\mu f^c | c | D v] D (a h b) d d + \\
& \frac{17}{48} D c f [\mu | d | D v] D (a h b) d c - \frac{11}{48} D [\mu h^c | c | d v] D (a f b) d + \frac{79}{96} D [\mu h^c d | c | D v] D (a f b) d - \\
& \frac{31}{24} D c h d [\mu | d | D v] D (a f b) c + \frac{101}{192} f [\mu^c D v] D (a D c h b) d d + \frac{2}{3} h [\mu^c d v] D (a D c f b) d - \frac{1}{3} h [\mu^c d v] D (a D d f b) c - \\
& \frac{19}{32} f [\mu^c D v] D (a D b) h c d d - \frac{1}{8} h [\mu^c d v] D (a D b) f c d + \frac{1}{3} h^c [\mu | c | D v] D (a D b) f d d + \frac{17}{96} f [\mu^c D v] D (a D | d | h b) c d \\
& - \frac{2}{3} h^c [\mu | c | D v] D (a D | d | f b) d - \frac{1}{64} D [\mu f (a | c | D v) D b) h c d d + \frac{35}{192} D c f (a [\mu D v] D b) h c d d + \\
& \frac{7}{36} e [\mu (a D | c f d f | D v) D b) h c d f - \frac{167}{288} e [\mu (a D | c f | d | d | D v) D b) h c f f + \frac{17}{48} D c f (a [\mu D v] D b) h d c d - \\
& \frac{5}{144} e [\mu (a D | c f d f | D v) D b) h d c f + \frac{5}{144} e [\mu (a D | c f | d | d | D v) D b) h f c f - \frac{3}{8} D [\mu h (a | c d | D v) D b) f c d \\
& + \frac{1}{48} D c h (a [\mu | d | D v] D b) f c d + \frac{5}{24} e [\mu (a D | c h | d | f d | D v) D b) f c f - \frac{11}{24} D [\mu h (a | c | c | D v) D b) f d d + \\
& \frac{5}{192} f (a [\mu D v] D b) D c h c d d - \frac{2}{3} D [\mu f (a b) D v] D c h c d d + \frac{17}{24} D c f [\mu | d | D v] D c h (a b) d - \frac{5}{8} D c f (a [\mu D v] D | c | h b) d d \\
& - \frac{5}{16} e [\mu (a D | c f d f | D v) D | c | h b) d f + \frac{137}{192} e [\mu (a D | c f | d d | D v) D c | h b) f f + \frac{133}{192} \eta a b D c f [\mu | d | D v] D c h d f f \\
& - \frac{23}{32} e [\mu (a D | c f b) d | D v] D c h d f f - \frac{11}{48} \eta a b D c f [\mu | d | D v] D c h f d f + \frac{13}{48} e [\mu (a D | c f b) d | D v] D c h f d f \\
& + \frac{61}{48} D c h d [\mu | d | D v] D c f (a b) + \frac{25}{24} D c h (a [\mu | d | D v] D | c | f b) d - \frac{79}{192} e [\mu (a D | c h | d f d | D v) D c | f b) f \\
& - \frac{11}{6} D c h (a b) [\mu D v] D c f d d - \frac{19}{72} \eta a b D c h [\mu | d f | D v] D c f d f - \frac{5}{8} e [\mu (a D | c h b) d f | D v] D c f d f + \\
& \frac{197}{192} e [\mu (a D | c h b) d d | D v] D c f f f - \frac{5}{144} \eta a b D c h d [\mu | d | D v] D c f f f - \frac{139}{96} f (a [\mu D v] D | c | D c h b) d d \\
& - \frac{1}{3} h (a b) [\mu D v] D c D c f d d + \frac{105}{64} f (a [\mu D v] D | c | D b) h c d d - \frac{7}{48} f (a [\mu D v] D | c D d | h b) c d + \\
& \frac{3}{8} \eta a b D [\mu f^c | c | D v] D d h d f f - \frac{4}{3} D [\mu f^c | c | D v] D d h (a b) d + \frac{41}{48} D [\mu f (a | c D v) D d | h b) c d + \\
& \frac{11}{24} e [\mu (a D | c f d f | D v) D | d | h b) c f - \frac{11}{48} e [\mu (a D | c f d f | D v) D | d | h b) f c - \frac{25}{144} \eta a b D c f [\mu | d | D v] D d h c f f \\
& + \frac{11}{64} e [\mu (a D | c f b) d | D v] D d h c f f - \frac{11}{36} \eta a b D c f [\mu | d | D v] D d h f c f + \frac{11}{48} e [\mu (a D | c f b) d | D v] D d h f c f + \\
& \frac{13}{12} D [\mu h (a b) c D v] D d f c d + D c h (a b) [\mu D v] D d f d c + \frac{7}{32} D [\mu h (a | c | c | D v) D d | f b) d - D c h (a [\mu | d | D v] D | d | f b) c \\
& + \frac{7}{12} \eta a b D c h [\mu | d f | D v] D d f c f + \frac{11}{48} e [\mu (a D | c h b) d f | D v] D d f c f - \frac{97}{64} \eta a b f [\mu^c D v] D d D c h d f f \\
& + \frac{131}{96} e [\mu (a f b) c D v] D d D c h d f f + \frac{97}{48} f [\mu^c D v] D d D c h (a b) d + \frac{167}{288} \eta a b f [\mu^c D v] D d D d h c f f - \\
& \frac{23}{32} e [\mu (a f b) c D v] D d D d h c f f + \frac{19}{12} f [\mu^c D v] D d D d h (a b) c + \frac{139}{96} e [\mu (a f | c | c | D v) D d | D d h b) f f \\
& + \frac{5}{6} h^c [\mu | c | D v] D d D d f (a b) - \frac{1}{48} h (a [\mu | c D v] D d | D d f b) c + \frac{13}{24} e [\mu (a h b) c | c | D v] D d D d f f f \\
& - \frac{3}{8} \eta a b h^c [\mu | c | D v] D d D d f f f - \frac{173}{96} f [\mu^c D v] D d D (a h b) c d - \frac{1}{8} h^c [\mu | c | D v] D d D (a f b) d - \\
& \frac{139}{96} e [\mu (a f | c | c | D v) D d | D b) h d f f + \frac{1}{48} h (a [\mu | c D v] D d | D b) f c d + \frac{61}{72} \eta a b f [\mu^c D v] D d D f h c d f -
\end{aligned}$$

$$\begin{aligned}
& \frac{13}{24} e_{[\mu} (a f b) c D \nu] D^d D^f h c d f - \frac{11}{24} e_{[\mu} (a h b) c |c| D \nu] D^d D^f f d f + \frac{5}{12} \eta^{a b h c} [\mu |c| D \nu] D^d D^f f d f \\
& - \frac{31}{72} \eta^{a b D} [\mu f c d D \nu] D^f h c d f + \eta^{a b D} c f [\mu |d| D \nu] D^f h f c d - \frac{11}{12} e_{[\mu} (a D |c f b) d | D \nu] D^f h f c d - \\
& \frac{7}{18} \eta^{a b D} c f [\mu |d| D \nu] D^f h f c d + \frac{11}{24} e_{[\mu} (a D |c f b) d | D \nu] D^f h f c d + \frac{23}{48} \eta^{a b D} [\mu h c |c| d D \nu] D^f f d f - \\
& \frac{337}{288} \eta^{a b D} [\mu h c d |c| D \nu] D^f f d f - \frac{149}{96} e_{[\mu} (a D |c h b) d d | D \nu] D^f f f c + \frac{5}{6} \eta^{a b D} c h d [\mu |d| D \nu] D^f f f c \\
& + \frac{47}{48} e_{[\mu} (a D |c h |d f d | D \nu] D^f |f b) c} - \frac{1}{2} \eta^{a b h} [\mu c d D \nu] D^f D c f d f + \frac{11}{24} e_{[\mu} (a h b) c d D \nu] D^f D c f d f \\
& + \frac{11}{36} \eta^{a b h} [\mu c d D \nu] D^f D d f c f - \frac{11}{48} e_{[\mu} (a h b) c d D \nu] D^f D d f c f - \frac{5}{8} e_{[\mu} (a f |c d D \nu] D^f |D f h b) c d + \\
& \frac{11}{72} \eta^{a b h} [\mu c d D \nu] D^f D f f c d - \frac{5}{16} e_{[\mu} (a h b) c d D \nu] D^f D f f c d + \frac{13}{48} e_{[\mu} (a h |c |c| d D \nu] D^f |D f f b) d - \\
& \frac{47}{96} e_{[\mu} (a h |c d |c| D \nu] D^f |D f b) d} + \frac{5}{8} e_{[\mu} (a f |c d D \nu] D^f |D b) h c d f - \frac{13}{48} e_{[\mu} (a h |c |c| d D \nu] D^f |D b) f d f \\
& + \frac{47}{96} e_{[\mu} (a h |c d |c| D \nu] D^f |D b) f d f} + \frac{9}{8} D [\mu D \nu] f d d D (a h b) c c - \frac{23}{24} D [\mu D d f |d | \nu] D (a h b) c c \\
& - \frac{11}{6} D [\mu D |c f d |d | D (a h b) c \nu] + \frac{25}{24} D [\mu D d f |d c| D (a h b) c \nu] + \frac{95}{48} D [\mu D |c| f \nu] d D (a h b) c d - \\
& \frac{17}{48} D [\mu D |d | f \nu] c D (a h b) c d - \frac{23}{24} D [\mu D \nu] f c d D (a h b) c d - \frac{5}{8} D [\mu D c h |c d d | D (a f b) \nu] + \frac{17}{12} D [\mu D |c| h d \nu] d D (a f b) c \\
& - \frac{19}{32} D [\mu D \nu] h d c d D (a f b) c - \frac{25}{96} f [\mu c D (a D |c| D \nu] h b) d d - \frac{49}{192} f [\mu c D (a D |c| D \nu] h d \nu] d + \\
& \frac{11}{32} f [\mu c D (a D |c D |d | h b) d | \nu] + \frac{5}{24} D [\mu f d |d | D (a D \nu] h b) c c + \frac{3}{8} D [\mu f |c d | D (a D \nu] h b) c d - \\
& \frac{15}{64} D [\mu h d |c d | D (a D \nu] f b) c + \frac{3}{32} f [\mu c D (a D \nu] D c h b) d d - \frac{5}{64} f [\mu c D (a D \nu] D b) h c d d - \frac{1}{96} f [\mu c D (a D \nu] D |d | h b) c d - \\
& \frac{5}{24} D [\mu f d |d | D (a D b) h c \nu] c - \frac{35}{48} D [\mu f \nu] d D (a D b) h c d c + \frac{127}{96} D [\mu f \nu] c D (a D b) h c d d - \frac{3}{8} D [\mu f |c d | D (a D b) h c d \nu] \\
& - \frac{1}{3} D [\mu h d \nu] d D (a D b) f c c + \frac{15}{64} D [\mu h d |c d | D (a D b) f c \nu] + \frac{1}{8} D [\mu h \nu] c d D (a D b) f c d + \frac{17}{192} f [\mu c D (a D b) D |c| h d \nu] d \\
& - \frac{17}{192} f [\mu c D (a D b) D \nu] h c d d - \frac{1}{6} D [\mu f \nu] d D (a D |c| h b) c d - \frac{13}{24} D [\mu f \nu] c D (a D |c| h b) d d + \\
& \frac{2}{3} D [\mu h d \nu] d D (a D |c| f b) c - \frac{1}{3} D [\mu h \nu] c d D (a D |c| f b) d - \frac{17}{96} f [\mu c D (a D |d | D |c h b) d | \nu] - \\
& \frac{1}{6} f [\mu c D (a D |d | D |d h b) c | \nu] + \frac{17}{96} f [\mu c D (a D |d | D \nu] h b) c d + \frac{1}{6} f [\mu c D (a D |d | D b) h |c d | \nu] - \\
& \frac{19}{24} D [\mu D (a f |d | |d | D b) h c \nu] c + \frac{85}{96} D [\mu D d f (a |d | D b) h c \nu] c - \frac{17}{48} D [\mu D |d | f (a \nu) D b) h c d c + \\
& \frac{11}{48} D [\mu D \nu] f (a d D b) h c d c - \frac{11}{24} D [\mu D (a f \nu) d D b) h c d c + \frac{7}{24} e_{[\mu} (a D \nu] D d f |f | f D b) h c d c - \\
& \frac{7}{12} e_{[\mu} (a D \nu] D |f | f f d D b) h c d c - \frac{119}{96} D [\mu D |c| f (a \nu) D b) h c d d - \frac{17}{192} D [\mu D \nu] f (a c D b) h c d d + \\
& \frac{247}{192} D [\mu D (a f \nu) c D b) h c d d - \frac{167}{96} e_{[\mu} (a D \nu] D c f |f | f D b) h c d d + \frac{125}{96} e_{[\mu} (a D \nu] D |f | f f c D b) h c d d \\
& + \frac{2}{3} D [\mu D |c f (a d | D b) h c d \nu] + \frac{1}{3} D [\mu D |d f (a c | D b) h c d \nu] - \frac{1}{4} D [\mu D (a f |c d | D b) h c d \nu] + \\
& \frac{11}{12} e_{[\mu} (a D \nu] D c f d f D b) h c d f + \frac{1}{24} e_{[\mu} (a D \nu] D d f c f D b) h c d f - \frac{1}{3} e_{[\mu} (a D \nu] D f f c d D b) h c d f \\
& + \frac{7}{8} D [\mu D \nu] h (a |d | d D b) f c c - \frac{19}{24} D [\mu D (a h |d | \nu] d D b) f c c - \frac{1}{3} D [\mu D d h (a |d | \nu] D b) f c c -
\end{aligned}$$

$$\frac{13}{24} e_{[\mu} \langle a D_{\nu]} D [d h_a f]_f D^b \rangle f^c c - \frac{29}{24} D_{[\mu} D_{|c} h \langle a [d]_a] D^b \rangle f^c c_{\nu]} + \frac{53}{64} D_{[\mu} D \langle a h [d]_{|c} a] D^b \rangle f^c c_{\nu]}$$

$$\begin{aligned}
& \frac{11}{16} D_{[\mu} D^d h^a (a|d c|D^b) f^c v] - \frac{1}{48} D_{[\mu} D_{|c|} h^a (a v|d D^b) f^c d + \frac{1}{24} D_{[\mu} D_{v]} h^a (a c d D^b) f^c d - \frac{1}{4} D_{[\mu} D^a (a h v|c d D^b) f^c d \\
& + \frac{5}{16} e_{[\mu} (a D v] D^c h^a |f| d f D^b) f^c d - \frac{3}{32} e_{[\mu} (a D v] D^d h^a |f| c f D^b) f^c d + \frac{5}{16} e_{[\mu} (a D v] D^f |h f c d D^b) f^c d \\
& - \frac{7}{64} e_{[\mu} (a f v|c|D^b) D^c D^d h^a d f^c + \frac{11}{48} D_{[\mu} f^a (a|d|D^b) D_{v]} h^c d c - \frac{103}{96} D_{[\mu} f^a (a|c|D^b) D_{v]} h^c d d \\
& + \frac{1}{3} D_{[\mu} h^a (a|d|d|D^b) D_{v]} f^c c - \frac{1}{8} D_{[\mu} h^a (a|c d|D^b) D_{v]} f^c d - \frac{5}{192} f^a (a_{[\mu} D^b) D_{v]} D^c h^c d d + \\
& \frac{1}{6} D_{[\mu} f^a (a|d D^b) D^c h^c |d v] + \frac{19}{24} D_{[\mu} f^a (a|c|D^b) D^c h^d v] d - \frac{2}{3} D_{[\mu} h^a (a|d|d|D^b) D^c f^c |v] + \frac{1}{3} D_{[\mu} h^a (a|c d|D^b) D^c f^d v] \\
& + \frac{3}{16} f^a (a_{[\mu} D^b) D^c D_{|c|} h^d v] d + \frac{23}{192} f^a (a_{[\mu} D^b) D^c D_{v]} h^c d d - \frac{3}{16} f^a (a_{[\mu} D^b) D^c D^d h^c |d v] - \\
& \frac{1}{192} e_{[\mu} (a f v|c|D^b) D^d D^c h^d f^c - \frac{11}{48} e_{[\mu} (a f v|c|D^b) D^d D^d h^c f^c + \frac{11}{48} e_{[\mu} (a f v|c|D^b) D^d D^f h^c d f + \\
& \frac{7}{12} D_{[\mu} D_{v]} f^a (a b) D^c h^c d d - \frac{5}{8} D_{[\mu} D^a (a f b) v] D^c h^c d d + \frac{1}{3} D_{[\mu} D_{|c|} f^d |d| D^c h^a (a b) v] - \frac{17}{24} D_{[\mu} D_{|c|} f^c v] d D^c h^a (a b) d \\
& + \frac{5}{8} D_{[\mu} D_{|c|} f^a (a v|D^c |h b) d d + \frac{13}{96} D_{[\mu} D_{v]} f^a (a c d |c| h b) d d - \frac{7}{32} D_{[\mu} D^a (a f v|c d |c| h b) d d + \\
& \frac{1}{48} D_{[\mu} D_{|c|} f^a (a|d|D^c |h b) d v] - \frac{5}{16} e_{[\mu} (a D v] D^c f^d d f D^c |h b) d f + \frac{185}{192} e_{[\mu} (a D v] D^c f^d d d |c| h b) f^c f \\
& - \frac{13}{12} D_{[\mu} D_{|c|} f^a (a b) D^c h^d v] d + \frac{1}{8} D_{[\mu} D^a (a f b) |c| D^c h^d v] d - \frac{51}{64} \eta^{a b} D_{[\mu} D_{|c|} f^c v] d D^c h^d f^c f + \\
& \frac{55}{1728} \eta^{a b} D_{[\mu} D_{v]} f^c d D^c h^d f^c f - \frac{51}{64} e_{[\mu} (a D v] D^c f^b) d D^c h^d f^c f + \frac{25}{288} e_{[\mu} (a D v] D^b) f^c d D^c h^d f^c f \\
& - \frac{11}{72} \eta^{a b} D_{[\mu} D_{|c|} f^d f|D^c h^d f^c v] + \frac{133}{144} \eta^{a b} D_{[\mu} D_{|c|} f^d |d| D^c h^f v] f + \frac{11}{48} \eta^{a b} D_{[\mu} D_{|c|} f^c v] d D^c h^f d f \\
& - \frac{7}{108} \eta^{a b} D_{[\mu} D_{v]} f^c d D^c h^f d f + \frac{13}{48} e_{[\mu} (a D v] D^c f^b) d D^c h^f d f - \frac{11}{144} e_{[\mu} (a D v] D^b) f^c d D^c h^f d f \\
& - \frac{73}{48} D_{[\mu} D_{|c|} h^d v] d D^c f^a (a b) + \frac{51}{32} D_{[\mu} D_{|c|} h^a (a|d|D^c |f b) v] - \frac{25}{24} D_{[\mu} D_{|c|} h^a (a v|d D^c |f b) d \\
& - \frac{15}{16} D_{[\mu} D_{v]} h^a (a c d D^c |f b) d + D_{[\mu} D^a (a h v|c d D^c |f b) d - \frac{47}{96} e_{[\mu} (a D v] D^c h^d |f d d |c| f b) f + \\
& \frac{11}{6} D_{[\mu} D_{|c|} h^a (a b) v] D^c f^d d + \frac{3}{2} D_{[\mu} D_{v]} h^a (a b) c D^c f^d d - \frac{3}{2} D_{[\mu} D^a (a h b) v] c D^c f^d d - \frac{19}{12} D_{[\mu} D_{|c|} h^a (a b) |d| D^c f^d v] \\
& + \frac{15}{16} D_{[\mu} D^a (a h b) |c d| D^c f^d v] + \frac{19}{72} \eta^{a b} D_{[\mu} D_{|c|} h^c v] d f D^c f^d f + \frac{41}{108} \eta^{a b} D_{[\mu} D_{v]} h^c d f D^c f^d f - \\
& \frac{5}{8} e_{[\mu} (a D v] D^c h^b) d f D^c f^d f + \frac{67}{144} e_{[\mu} (a D v] D^b) h^c d f D^c f^d f + \frac{59}{144} \eta^{a b} D_{[\mu} D_{|c|} h^d v] d D^c f^f f \\
& + \frac{245}{192} e_{[\mu} (a D v] D^c h^b) d d D^c f^f f - \frac{139}{288} \eta^{a b} D_{[\mu} D_{|c|} h^d f |d| D^c f^f v] + \frac{51}{32} D_{[\mu} f^a (a v|D^c |D^c h b) d d \\
& - \frac{25}{48} D_{[\mu} f^a (a b) D^c D_{|c|} h^d v] d + \frac{1}{3} D_{[\mu} h^a (a b) v] D^c D^c f^d d - \frac{7}{192} f^a (a_{[\mu} D^c |c| D_{|c|} D_{v]} h^b) d d + \\
& \frac{7}{192} f^a (a_{[\mu} D^c |c| D_{|c|} D^b) h^d v] d + \frac{125}{48} D_{[\mu} f^a (a b) D^c D_{v]} h^c d d - \frac{9}{8} D_{[\mu} f^c |c d| D^c D_{v]} h^a (a b) d - \\
& \frac{1}{24} D_{[\mu} f^a (a|c|D^c |D_{v]} h^b) d d + \frac{197}{216} \eta^{a b} D_{[\mu} f^c |c d| D^c D_{v]} h^d f^c f - \frac{17}{54} \eta^{a b} D_{[\mu} f^c |c d| D^c D_{v]} h^f d f \\
& + \frac{7}{54} \eta^{a b} D_{[\mu} h^c |c d f| D^c D_{v]} f^d f - \frac{25}{192} f^a (a_{[\mu} D^c |c| D_{v]} D^c h^b) d d - \frac{1}{96} f^a (a_{[\mu} D^c |c| D_{v]} D^b) h^c d d \\
& + \frac{3}{32} f^a (a_{[\mu} D^c |c D_{v]} D^d |h b) c d - \frac{113}{96} D_{[\mu} f^c v] c D^c D^a (a h b) d d + \frac{17}{16} D_{[\mu} f^c |c d| D^c D^a (a h b) d v] - \\
& \frac{51}{32} D_{[\mu} f^a (a v|D^c |D^b) h^c d d + \frac{5}{96} D_{[\mu} f^a (a|c|D^c |D^b) h^d v] d + \frac{259}{288} e_{[\mu} (a D v] f^c d D^c |c| D^b) h^d f^c f -
\end{aligned}$$



$$\begin{aligned}
& \frac{7}{18}e_{[\mu} (a D_{\nu]} f_{c d} D_{|c|} D_{|b)} h^f d^f + \frac{11}{72}e_{[\mu} (a D_{\nu]} h_{c d} f_{|c|} D_{|b)} f^f d^f - \frac{13}{64}f_{[\mu} D_{|c|} D_{|b)} D_{|c|} h^f d_{\nu]} a \\
& - \frac{5}{32}f_{[\mu} D_{|c|} D_{|b)} D_{\nu]} h_{c d} d^f + \frac{23}{96}f_{[\mu} D_{|c|} D_{|b)} D^d h_{|c d|} \nu] - 2D_{[\mu} f_{(a b)} D^c D^d h_{|c d|} \nu] + \\
& \frac{11}{72}\eta^{a b} D_{[\mu} f_{\nu]} c D^c D^d h_{d f} + \frac{11}{96}e_{[\mu} (a D_{\nu]} f_{b)} c D^c D^d h_{d f} + 2D_{[\mu} f_{\nu]} c D^c D^d h_{(a b)} d - D_{[\mu} f_{|c d|} D^c D^d h_{(a b)} \nu] \\
& - \frac{29}{32}e_{[\mu} (a D_{\nu]} f_{c d} D_{|c|} D_{|d|} h^b) f^f - \frac{7}{36}\eta^{a b} D_{[\mu} f_{|c d|} D^c D^d h^f \nu] + \frac{1}{6}f_{[\mu} D_{|c|} D_{|d|} D_{|c h b)} d_{\nu]} \\
& - \frac{1}{6}f_{[\mu} D_{|c|} D_{|d|} D_{|d h b)} c_{\nu]} + \frac{7}{96}f_{[\mu} D_{|c|} D_{|d|} D_{\nu]} h^b) c_d - \frac{7}{96}f_{[\mu} D_{|c|} D_{|d|} D_{|b)} h_{|c d|} \nu] - \\
& \frac{5}{12}\eta^{a b} D_{[\mu} f_{|c d} D^c D^d h^f d_{\nu]} + \frac{5}{16}e_{[\mu} (a D_{\nu]} f_{c d} D_{|c|} D_{|d|} h^b) f^f d - D_{[\mu} D^c f_{(a b)} D^d h_{|c d|} \nu] - \\
& \frac{31}{72}\eta^{a b} D_{[\mu} D_{\nu]} f_{c c} D^d h_{d f} + \frac{37}{72}\eta^{a b} D_{[\mu} D^c f_{|c|} \nu] D^d h_{d f} - \frac{13}{24}e_{[\mu} (a D_{\nu]} D_{|b)} f_{c c} D^d h_{d f} + \\
& \frac{11}{24}e_{[\mu} (a D_{\nu]} D_{|c|} f_{b)} c D^d h_{d f} - \frac{4}{3}D_{[\mu} D_{\nu]} f_{c c} D^d h_{(a b)} d + D_{[\mu} D^c f_{|c|} \nu] D^d h_{(a b)} d - \frac{1}{48}D_{[\mu} D_{\nu]} f_{(a |c|} D_{|d|} h^b) c_d \\
& + \frac{11}{16}D_{[\mu} D_{(a f \nu]} D_{|c|} D_{|d|} h^b) c_d - \frac{1}{3}D_{[\mu} D_{(a f |c|} D_{|c|} D_{|d|} h^b) d_{\nu]} - \frac{13}{48}e_{[\mu} (a D_{\nu]} D_{|c|} f_{c d} D_{|d|} h^b) f^f + \\
& \frac{31}{72}\eta^{a b} D_{[\mu} D_{|c|} f_{\nu]} d D^d h^c f^f + \frac{37}{96}e_{[\mu} (a D_{\nu]} D_{c f} b) d D^d h^c f^f - \frac{3}{8}\eta^{a b} D_{[\mu} D^c f_{|c d|} D^d h^f \nu] f - \\
& \frac{5}{12}D_{[\mu} D_{\nu]} h_{(a b)} c D^d f_{c d} + \frac{25}{24}D_{[\mu} D_{(a h b)} \nu] c D^d f_{c d} - D_{[\mu} D^c h_{(a b)} \nu] D^d f_{c d} - \frac{23}{24}D_{[\mu} D_{(a h b)} c_{|c|} D^d f_{d \nu]} \\
& + D_{[\mu} D^c h_{(a b)} |c| D^d f_{d \nu]} + \frac{49}{32}D_{[\mu} D_{\nu]} h_{c d} c D^d f_{(a b)} - D_{[\mu} D^c h_{|c|} \nu] d D^d f_{(a b)} - \frac{23}{32}D_{[\mu} D_{\nu]} h_{(a |c|} c D_{|d|} f_{b)} d \\
& + \frac{85}{96}D_{[\mu} D_{(a h |c|} \nu] c D_{|d|} f_{b)} d - \frac{203}{192}D_{[\mu} D_{(a h |c|} d_{c|} D_{|d|} f_{b)} \nu] + D_{[\mu} D_{|c|} h_{(a \nu]} d D_{|d|} f_{b)} c - \\
& \frac{5}{16}e_{[\mu} (a D_{\nu]} D_{|c h c d f} D_{|d|} f_{b)} f^f - D_{[\mu} D_{|c h (a b)} d_{\nu]} D^d f_{c \nu]} - \frac{2}{3}\eta^{a b} D_{[\mu} D_{|c|} h_{\nu]} d^f D^d f_{c f} - \\
& \frac{1439}{1728}\eta^{a b} D_{[\mu} D_{\nu]} h_{c d} c D^d f^f + \frac{2}{3}\eta^{a b} D_{[\mu} D^c h_{|c|} \nu] d D^d f^f - \frac{65}{72}e_{[\mu} (a D_{\nu]} D_{|b)} h_{c d} c D^d f^f \\
& - \frac{5}{12}\eta^{a b} D_{[\mu} D^c h_{|c d f|} D^d f^f \nu] + \frac{11}{8}\eta^{a b} D_{[\mu} f_{\nu]} c D^d D_{c h} d^f + \frac{1}{8}\eta^{a b} D_{[\mu} f_{c \nu]} D^d D_{c h} d^f \\
& + \frac{131}{96}e_{[\mu} (a D_{\nu]} f_{b)} c D^d D_{c h} d^f - 2D_{[\mu} f_{\nu]} c D^d D_{c h} (a b) d + \frac{3}{2}D_{[\mu} f_{(a |c|} D_{|d|} D_{|c h b)} d_{\nu]} + \\
& \frac{47}{192}e_{[\mu} (a f \nu] |c| D_{|d|} D_{c D} d_{h b)} f^f + \frac{15}{64}\eta^{a b} f_{[\mu} c D^d D_{|c d|} h^f \nu] + \frac{7}{32}\eta^{a b} f_{[\mu} c D^d D_{|c|} D_{\nu]} h_{d f} \\
& + \frac{23}{96}e_{[\mu} (a f \nu] |c| D_{|d|} D_{c D} b) h_{d f} - \frac{29}{96}\eta^{a b} f_{[\mu} c D^d D_{|c d|} h^f d_{\nu]} - \frac{31}{96}e_{[\mu} (a f \nu] |c| D^d D_{c D} f_{|h b)} d^f \\
& + \frac{11}{288}\eta^{a b} D_{[\mu} f_{\nu]} c D^d D_{d h} c^f - \frac{31}{192}e_{[\mu} (a D_{\nu]} f_{b)} c D^d D_{d h} c^f - \frac{19}{12}D_{[\mu} f_{\nu]} c D^d D_{d h} (a b) c \\
& + \frac{7}{3}D_{[\mu} f_{c |c|} D^d D_{d|} h_{(a b)} \nu] - \frac{37}{24}D_{[\mu} f_{(a |c|} D_{|d|} D_{|d h b)} c_{\nu]} + \frac{139}{96}e_{[\mu} (a D_{\nu]} f_{|c|} c D_{|d|} D_{d h b)} f^f - \\
& \frac{107}{144}\eta^{a b} D_{[\mu} f_{c \nu]} D^d D_{d h} c^f - \frac{107}{192}e_{[\mu} (a D_{\nu]} f_{b)} c D^d D_{d h} c^f + \frac{1}{4}\eta^{a b} D_{[\mu} f_{c |c|} D^d D_{d|} h^f \nu] f - \\
& \frac{17}{24}D_{[\mu} h_{(a b)} c D^d D_{|d f c|} \nu] - \frac{5}{6}D_{[\mu} h_{c \nu]} c D^d D_{d f} (a b) + \frac{1}{48}D_{[\mu} h_{(a \nu]} |c| D_{|d|} D_{d f} b) c + \frac{5}{8}D_{[\mu} h_{(a |c|} c D_{|d|} D_{d|} f_{b)} \nu] \\
& + \frac{3}{8}\eta^{a b} D_{[\mu} h_{c \nu]} c D^d D_{d f} f^f + \frac{13}{24}e_{[\mu} (a D_{\nu]} h_{b)} c c D^d D_{d f} f^f - \frac{5}{64}e_{[\mu} (a f \nu] |c| D_{|d|} D_{d D} c_{h b)} f^f - \\
& \frac{13}{192}\eta^{a b} f_{[\mu} c D^d D_{|d d c|} h^f \nu] + \frac{13}{192}\eta^{a b} f_{[\mu} c D^d D_{|d|} D_{\nu]} h_{c f} + \frac{5}{64}e_{[\mu} (a f \nu] |c| D_{|d|} D_{d D} b) h_{c f} \\
& - \frac{11}{8}\eta^{a b} D_{[\mu} f_{c |c|} D^d D_{\nu]} h_{d f} + \frac{7}{3}D_{[\mu} f_{c |c|} D^d D_{\nu]} h_{(a b)} d - \frac{31}{24}D_{[\mu} f_{(a |c|} D_{|d|} D_{\nu]} h^b) c_d
\end{aligned}$$

$$\begin{aligned}
& + \frac{1}{24} D [\mu h (a b) c D d v] f c d + \frac{3}{32} D [\mu h c | d c | D d v] f (a b) - \frac{1}{8} D [\mu h (a | c | c | D d | D v] f b) d - \\
& \frac{239}{1728} \eta^{a b} D [\mu h c | d c | D d v] f f f - \frac{5}{96} \eta^{a b} f [\mu c D d v] D c h d f f + \frac{19}{192} \eta^{a b} f [\mu c D d v] D d h c f f - \\
& \frac{1}{32} \eta^{a b} f [\mu c D d v] D f h c d f + \frac{43}{24} D [\mu f v] c D d (a h b) c d - \frac{7}{3} D [\mu f c | c D d (a h b) d | v] + \frac{1}{8} D [\mu h c v] c D d (a f b) d \\
& - \frac{17}{192} D [\mu h c | d c | D d (a f b) v] + \frac{4}{3} D [\mu f (a | c D d | D b) h | c d | v] - \frac{139}{96} e [\mu (a D v) f | c c D d | D b) h d f f \\
& - \frac{1}{48} D [\mu h (a v) | c D d | D b) f c d + \frac{1}{12} D [\mu h (a | c | c D d | D b) f d | v] - \frac{47}{288} e [\mu (a D v) h | c d c D d | D b) f f f - \\
& \frac{7}{96} e [\mu (a f v) | c D d | D b) D c h d f f + \frac{17}{192} e [\mu (a f v) | c D d | D b) D d h c f f - \frac{1}{96} e [\mu (a f v) | c D d | D b) D f h c d f \\
& - \frac{13}{18} \eta^{a b} D [\mu f v] c D d f h c d f - \frac{13}{24} e [\mu (a D v) f b) c D d f h c d f + \frac{10}{9} \eta^{a b} D [\mu f c | c D d f h d f | v] - \\
& \frac{5}{12} \eta^{a b} D [\mu h c v] c D d f f d f - \frac{11}{24} e [\mu (a D v) h b) c c D d f f d f + \frac{11}{144} \eta^{a b} D [\mu h c | d c D d f f | v] + \\
& \frac{11}{192} e [\mu (a D v) h | c d c D d f | f b) f + \frac{13}{96} \eta^{a b} f [\mu c D d f D | c h d f | v] + \frac{5}{32} e [\mu (a f v) | c D d f | D c h b) d f \\
& - \frac{1}{6} \eta^{a b} f [\mu c D d f D | d h c f | v] - \frac{1}{6} e [\mu (a f v) | c D d f | D d h b) c f + \frac{1}{6} \eta^{a b} f [\mu c D d f D | f h c d | v] + \\
& \frac{1}{6} e [\mu (a f v) | c D d f | D f h b) c d - \frac{13}{96} \eta^{a b} f [\mu c D d f D v] h c d f - \frac{5}{32} e [\mu (a f v) | c D d f | D b) h c d f \\
& + \frac{31}{72} \eta^{a b} D [\mu D v] f c d D f h c d f - \frac{37}{36} \eta^{a b} D [\mu D c f v] d D f h c d f + \frac{5}{16} e [\mu (a D v) D b) f c d D f h c d f - \\
& \frac{37}{48} e [\mu (a D v) D | c | f b) d D f h c d f + \frac{8}{9} \eta^{a b} D [\mu D c f d | d D f h c f | v] - \frac{1}{6} \eta^{a b} D [\mu D c f | c d D f h d f | v] + \\
& \frac{13}{24} e [\mu (a D v) D | c f c d D f | h b) d f - \frac{5}{6} \eta^{a b} D [\mu D c h d v] d D f f c f - \frac{151}{96} e [\mu (a D v) D | c | h b) d d D f f c f \\
& - \frac{23}{48} \eta^{a b} D [\mu D v] h c c d D f f d f + \frac{79}{96} \eta^{a b} D [\mu D v] h c d c D f f d f - \frac{1}{6} \eta^{a b} D [\mu D c h | c | v] d D f f d f - \\
& \frac{7}{12} e [\mu (a D v) D b) h c c d D f f d f + \frac{13}{16} e [\mu (a D v) D b) h c d c D f f d f + \frac{13}{24} e [\mu (a D v) D | c | h b) c d D f f d f \\
& + \frac{29}{72} \eta^{a b} D [\mu D v] h c d d D f f c - \frac{3}{8} \eta^{a b} D [\mu D c h d v] d D f f c + \frac{47}{96} e [\mu (a D v) D b) h c d d D f f c - \\
& \frac{1}{4} e [\mu (a D v) D | c | h b) d d D f f c + \frac{37}{72} \eta^{a b} D [\mu D c h | c d d D f f | v] + \frac{11}{24} e [\mu (a D v) D | c h c d d D f | f b) f + \\
& \frac{185}{192} e [\mu (a D v) D c h | d f d D f | f b) c + \frac{155}{144} \eta^{a b} D [\mu D | c h d f d | D f f c v] - \frac{17}{18} \eta^{a b} D [\mu f c d D f D | c h d f | v] \\
& + \frac{1}{2} \eta^{a b} D [\mu h v] c d D f D c f d f + \frac{11}{24} e [\mu (a D v) h b) c d D f D c f d f - \frac{1}{144} \eta^{a b} D [\mu h c d | d D f D c f | v] - \\
& \frac{1}{192} e [\mu (a D v) h | c d d D f | D c f b) f - \frac{11}{36} \eta^{a b} D [\mu h v] c d D f D d f c f - \frac{11}{48} e [\mu (a D v) h b) c d D f D d f c f - \\
& \frac{1}{48} \eta^{a b} D [\mu h c d | c D f D d f | v] + \frac{1}{192} e [\mu (a D v) h | c d c D f | D d f b) f + \frac{31}{72} \eta^{a b} D [\mu f c d D f D | f h c d | v] \\
& - \frac{5}{8} e [\mu (a D v) f | c d D f | D f h b) c d - \frac{11}{72} \eta^{a b} D [\mu h v] c d D f D f f c d - \frac{5}{16} e [\mu (a D v) h b) c d D f D f f c d + \\
& \frac{11}{48} \eta^{a b} D [\mu h c | c d D f D f d | v] - \frac{809}{1728} \eta^{a b} D [\mu h c d | c D f D f f d | v] - \frac{1}{432} \eta^{a b} D [\mu h c d | d D f D f | v] c - \\
& \frac{1}{576} e [\mu (a D v) h | c d d D f | D f b) c + \frac{13}{48} e [\mu (a D v) h | c c d D f | D f b) d - \frac{281}{576} e [\mu (a D v) h | c d c D f | D f b) d \\
& + \frac{37}{72} \eta^{a b} D [\mu f c d D f D v] h c d f - \frac{11}{48} \eta^{a b} D [\mu h c | c | d D f D v] f d f + \frac{239}{576} \eta^{a b} D [\mu h c d | c | D f D v] f d f +
\end{aligned}$$

$$\begin{aligned}
& \frac{5}{8}e_{[\mu} \langle a D_{\nu} \rangle f | c d D^f | D^b \rangle h_{c d f} - \frac{13}{48}e_{[\mu} \langle a D_{\nu} \rangle h | c c^d D^f | D^b \rangle f_{d f} + \frac{47}{96}e_{[\mu} \langle a D_{\nu} \rangle h | c d c^d D^f | D^b \rangle f_{d f} \\
& + \frac{1}{24}\eta^{ab} f_{[\mu} c f d^f D | c h d f | \nu] - \frac{7}{16}\eta^{ab} f_{[\mu} c f \nu] d D c h d^f f + \frac{21}{32}e_{[\mu} \langle a f \nu \rangle | d | f b \rangle c D c h d^f f - \\
& \frac{5}{4}f_{[\mu} c f \nu] d D c h \langle a b \rangle_d + \frac{4}{3}f_{[\mu} c f d | d D c | h \langle a b \rangle_{\nu]} - \frac{7}{24}e_{[\mu} \langle a f \nu \rangle | c f d^f | D c h b \rangle_d f - f_{[\mu} d^f \langle a | c | D | c h b \rangle_d | \nu] + \\
& \frac{2}{3}f \langle a | \mu f | c d | D | c h b \rangle_d | \nu] + \frac{5}{6}f_{[\mu} c f \langle a_{\nu} \rangle D c h b \rangle_d d - \frac{89}{96}e_{[\mu} \langle a f \nu \rangle | c f d | d D c h b \rangle_f f + \frac{103}{48}f_{[\mu} c f \langle a b \rangle D | c | h d^d_{\nu]} d \\
& - \frac{17}{96}f \langle a | c | f b \rangle_{[\mu} D | c | h d^d_{\nu]} d - \frac{17}{96}f \langle a | \mu f b \rangle c D | c | h d^d_{\nu]} d - \frac{41}{32}\eta^{ab} f_{[\mu} c f d | d D c | h^f_{\nu]} f \\
& - \frac{13}{24}\eta^{ab} h_{[\mu} c d f \nu] f D c f d f + \frac{5}{8}e_{[\mu} \langle a h b \rangle c d f \nu] f D c f d f + \frac{7}{24}h \langle a | c d | f b \rangle_{[\mu} D | c f d | \nu] - \\
& \frac{1}{3}\eta^{ab} h c d f f_{[\mu} D | c f f | \nu] + \frac{7}{24}h_{[\mu} c d f \langle a_{\nu} \rangle D c f b \rangle_d - \frac{1}{3}e_{[\mu} \langle a h | c d f | f | d | \nu] D c f b \rangle_f - \\
& \frac{4}{3}h \langle a b \rangle_{[\mu} f \nu] c D c f d d + \frac{2}{3}h \langle a | \mu | c | f b \rangle_{\nu]} D c f d d - \frac{2}{3}\eta^{ab} f_{[\mu} c f d^f D | d h c f | \nu] + \frac{7}{16}\eta^{ab} f_{[\mu} c f \nu] d D d h c^f f \\
& + \frac{67}{96}e_{[\mu} \langle a f \nu \rangle | d | f b \rangle c D d h c^f f + \frac{1}{4}e_{[\mu} \langle a f b \rangle_{\nu]} f c d D d h c^f f + \frac{5}{4}f_{[\mu} c f \nu] d D d h \langle a b \rangle_c \\
& + 2f c^d f c_{[\mu} D | d | h \langle a b \rangle_{\nu]} - \frac{2}{3}e_{[\mu} \langle a f \nu \rangle | c f d^f | D d h b \rangle_c f - \frac{17}{24}f_{[\mu} d^f \langle a | c | D | d h b \rangle_c | \nu] + \\
& \frac{15}{64}e_{[\mu} \langle a f | c | | d f c | \nu] D d h b \rangle_f f - \frac{9}{64}e_{[\mu} \langle a f \nu \rangle c f | c d | D d h b \rangle_f f + \frac{13}{64}\eta^{ab} f c^d f c_{[\mu} D | d | h^f_{\nu]} f \\
& - \frac{17}{192}\eta^{ab} f_{[\mu} | c f c^d D d | h^f_{\nu]} f + \frac{29}{48}\eta^{ab} h_{[\mu} c d f \nu] f D d f c f - \frac{31}{48}e_{[\mu} \langle a h b \rangle c d f \nu] f D d f c f \\
& - \frac{11}{8}h \langle a b \rangle c f_{[\mu} d D | d f c | \nu] + \frac{3}{16}h \langle a | c d | f b \rangle_{[\mu} D | d f c | \nu] - \frac{5}{24}\eta^{ab} h c d f f c_{[\mu} D | d f f | \nu] - \\
& \frac{1}{6}\eta^{ab} h c d c f_{[\mu} f D | d f f | \nu] + \frac{5}{12}h c_{[\mu} | c | f \nu] d D d f \langle a b \rangle + \frac{31}{48}h \langle a | \mu | c f \nu \rangle d | D d f b \rangle_c - \frac{23}{48}h_{[\mu} c d f \langle a_{\nu} \rangle D d f b \rangle_c \\
& - \frac{7}{24}e_{[\mu} \langle a h | c d f | f | c | \nu] D d f b \rangle_f - \frac{1}{6}e_{[\mu} \langle a h | c d | c | f \nu] f | D d f b \rangle_f + \frac{25}{24}h \langle a | c c f_{[\mu} d | D | d | f b \rangle_{\nu]} \\
& + \frac{1}{6}h c^d c f \langle a | \mu D | d | f b \rangle_{\nu]} - \frac{2}{3}\eta^{ab} h_{[\mu} c d f | c | \nu] D d f f + \frac{2}{3}e_{[\mu} \langle a h b \rangle c d f | c | \nu] D d f f + \\
& \frac{7}{24}e_{[\mu} \langle a h b \rangle c | c | f \nu] d D d f f + \frac{1}{8}\eta^{ab} h c_{[\mu} | c | f \nu] d D d f f + \frac{1}{3}e_{[\mu} \langle a h | c d | | c | f b \rangle_{\nu]} D d f f \\
& - \frac{11}{48}\eta^{ab} h_{[\mu} c d f \nu] f D f f c d - \frac{11}{48}e_{[\mu} \langle a h b \rangle c d f \nu] f D f f c d - \frac{1}{16}\eta^{ab} h c d f f_{[\mu} D | f f c | \nu] + \\
& \frac{3}{16}\eta^{ab} h c c^d f_{[\mu} f D | f f d | \nu] - \frac{19}{48}\eta^{ab} h c d c f_{[\mu} f D | f f d | \nu] - \frac{1}{48}e_{[\mu} \langle a h | c d f | f | d | \nu] D f f b \rangle_c + \\
& \frac{7}{16}e_{[\mu} \langle a h | c | c | d f \nu] f | D f f b \rangle_d - \frac{53}{96}e_{[\mu} \langle a h | c d | c | f \nu] f | D f f b \rangle_d + 2f \langle a | c | f b \rangle_d D_{[\mu} h | c d | \nu] - \\
& 2f \langle a b \rangle_f c^d D_{[\mu} h | c d | \nu] + \frac{5}{3}\eta^{ab} f c c f d^f D_{[\mu} h | d f | \nu] - \eta^{ab} f c^d f c^f D_{[\mu} h | f d | \nu] + 2f c c f d^d D_{[\mu} h \langle a b \rangle_{\nu]} \\
& - 4f \langle a | c f d | d D_{[\mu} h b \rangle_{| c | \nu]} + 2f c^d f \langle a | c | D_{[\mu} h b \rangle_{| d | \nu]} - 3f \langle a | c | f b \rangle_c D_{[\mu} h d^d_{\nu]} d + \frac{13}{2}f \langle a b \rangle_f c c D_{[\mu} h d^d_{\nu]} d \\
& + \frac{1}{2}\eta^{ab} f c d f c^d D_{[\mu} h^f_{\nu]} f - \frac{19}{12}\eta^{ab} f c c f d d D_{[\mu} h^f_{\nu]} f - \frac{2}{3}\eta^{ab} h c d f f d f D_{[\mu} f | c | \nu] + \\
& 2h \langle a | c d | f b \rangle_d D_{[\mu} f | c | \nu] - 2h \langle a b \rangle c f c^d D_{[\mu} f | d | \nu] - 2h c c^d f \langle a b \rangle D_{[\mu} f | d | \nu] - \frac{5}{2}h c^d c f \langle a b \rangle D_{[\mu} f | d | \nu] \\
& + \frac{1}{2}h \langle a | c | c f b \rangle_d D_{[\mu} f | d | \nu] - \frac{1}{3}\eta^{ab} h c c^d f f D_{[\mu} f | d | \nu] + \frac{7}{4}\eta^{ab} h c^d c f f f D_{[\mu} f | d | \nu] + \\
& \frac{2}{3}\eta^{ab} h c c^d f d^f D_{[\mu} f | f | \nu] - \eta^{ab} h c^d c f d^f D_{[\mu} f | f | \nu] + h c^d c f \langle a d D_{[\mu} f b \rangle_{\nu]} - h \langle a | c c f d | d D_{[\mu} f b \rangle_{\nu]} +
\end{aligned}$$



$$\begin{aligned}
& + \frac{3}{4} e_{[\mu} (a f^b)_{\nu]} f^c{}_c D^d h_d{}^f{}_f - \frac{7}{32} \eta^{ab} f_{[\mu} |c| f^c{}_{\nu]} D^d h_d{}^f{}_f - \frac{1}{24} f_{[\mu}{}^c f^c (a_{\nu]} D^d |d| h^b)_{\phantom{b}c}{}_d + \\
& f_{[\mu} |c| f^c (a^{|c|} D^d |h^b)_{\phantom{b}d}| \nu]} - \frac{5}{3} f^c (a_{[\mu} f^c |c| D^d |h^b)_{\phantom{b}d}| \nu]} - \frac{2}{3} h^c (a_{[\mu} |c| f^b)_{\nu]} D^d f^c{}_d - \frac{19}{24} h^c (a^{|c|} c f^b)_{[\mu} D^d f^c |d| \nu]} \\
& + \frac{5}{24} h^c{}_{[\mu} |c| f^c (a_{\nu]} D^d |d| f^b)_{\phantom{b}d}{}_d - \frac{17}{24} e_{[\mu} (a f_{\nu]} |d| f^b)_{\phantom{b}c} D^d f^c h_c{}^d{}_f - \frac{1}{3} e_{[\mu} (a f^b)_{\nu]} f^c{}_c D^d f^c h_c{}^d{}_f \\
& + \frac{5}{3} \eta^{ab} f_{[\mu}{}^c f^c |d| D^d f^c h_c{}^f| \nu]} + \frac{3}{16} \eta^{ab} f^c{}_c f^c{}_{[\mu} D^d f^c h_c{}^f| \nu]} - \frac{1}{16} \eta^{ab} f_{[\mu} |c| f^c{}_c D^d f^c h_c{}^f| \nu]} + \\
& \frac{5}{3} e_{[\mu} (a f_{\nu]} |c| f^c{}_d D^d f^c |h^b)_{\phantom{b}c}{}_f + \frac{1}{16} e_{[\mu} (a f_{\nu]} |c| |d| f^c{}_{\nu]} D^d f^c |h^b)_{\phantom{b}d}{}_f - \frac{1}{48} e_{[\mu} (a f_{\nu]} c f^c |c| D^d f^c |h^b)_{\phantom{b}d}{}_f \\
& + \frac{2}{3} \eta^{ab} h_{[\mu}{}^c{}_d f^c |c| \nu]} D^d f^c{}_d f^c{}_f - \frac{2}{3} e_{[\mu} (a h^b)_{\nu]} c^c{}_d f^c |c| \nu]} D^d f^c{}_d f^c{}_f - \frac{1}{8} e_{[\mu} (a h^b)_{\nu]} c^c |c| f_{\nu]} D^d f^c{}_d f^c{}_f + \\
& \frac{1}{24} \eta^{ab} h^c{}_{[\mu} |c| f_{\nu]} D^d f^c{}_d f^c{}_f - \frac{1}{3} e_{[\mu} (a h^c |c| |c| f^b)_{\nu]} D^d f^c{}_d f^c{}_f + \frac{29}{48} \eta^{ab} h^c{}_c c^c{}_d f^c{}_d [\mu D^d f^c |f| \nu]} + \\
& \frac{7}{16} \eta^{ab} h^c{}_c c^c{}_d f^c{}_d [\mu D^d f^c |f| \nu]} + \frac{31}{48} e_{[\mu} (a h^c |c| c^c{}_d f^c{}_d | \nu]} D^d f^c |f^b)_{\phantom{b}f}{}_f + \frac{23}{48} e_{[\mu} (a h^c |c| c^c f^c{}_d | \nu]} D^d f^c |f^b)_{\phantom{b}f}{}_f
\end{aligned}$$
